# Supplementary material for: Magnetic Structures Database from Symmetry-aided High-Throughput Calculations
Source: arXiv:2601.01617 source file (2026-10-14)
Supplement: Supplementary file 1 [file SM-0122woP-0124.tex]

\documentclass[superscriptaddress]{revtex4-1}
\usepackage{graphicx}% Include figure files
\usepackage{dcolumn}% Align table columns on decimal point
\usepackage{bm}% bold math
\usepackage{blindtext}
\usepackage{amsfonts}
\usepackage{amsmath}
\usepackage{amssymb}
\usepackage{color}
\usepackage{multirow}
\usepackage{tabularx}
\usepackage{epstopdf}
\usepackage{booktabs}
\usepackage{longtable}
\usepackage{rotating}
\usepackage{geometry}
\usepackage{makecell}
\usepackage{hyperref}% add hypertext capabilities

\geometry{a4paper, margin=1cm}
\usepackage[capitalize]{cleveref}
%\usepackage{pdfpages}

 %change text font to Times New Roman
 
\DeclareSymbolFont{myletters}{OML}{ztmcm}{m}{it}
\DeclareMathSymbol{\uplambda}{\mathord}{myletters}{"15}

\setcounter{tocdepth}{2}
\setcounter{secnumdepth}{3}

\begin{document}

\title{Supplemental Materials for “Magnetic Structures Database from Symmetry-aided High-Throughput Calculations”}
\date{\today }

\author{Hanjing Zhou}
\thanks{These authors contributed equally to this work.}
\affiliation{National Laboratory of Solid State Microstructures and School of Physics,
Nanjing University, Nanjing 210093, China}
\affiliation{Collaborative Innovation Center of Advanced Microstructures, Nanjing
University, Nanjing 210093, China}
\author{Yuxuan Mu}
\thanks{These authors contributed equally to this work.}
\affiliation{National Laboratory of Solid State Microstructures and School of Physics,
Nanjing University, Nanjing 210093, China}
\affiliation{Collaborative Innovation Center of Advanced Microstructures, Nanjing
University, Nanjing 210093, China}
\author{Dingwen Zhang}
\thanks{These authors contributed equally to this work.}
\affiliation{National Laboratory of Solid State Microstructures and School of Physics,
Nanjing University, Nanjing 210093, China}
\affiliation{Collaborative Innovation Center of Advanced Microstructures, Nanjing
University, Nanjing 210093, China}
\author{Hangbing Chu}
\affiliation{National Laboratory of Solid State Microstructures and School of Physics,
Nanjing University, Nanjing 210093, China}
\affiliation{Collaborative Innovation Center of Advanced Microstructures, Nanjing
University, Nanjing 210093, China}
\author{Erjun Kan}
\affiliation{MIIT Key Laboratory of Semiconductor Microstructure and Quantum Sensing, Nanjing University of Science and Technology, Nanjing, Jiangsu 210037, People's Republic of China}
\author{Chun-Gang Duan}
\affiliation{Key Laboratory of Polar Materials and Devices, Ministry of Education, East China Normal University, Shanghai 200241, China}
\affiliation{Shanghai Center of Brain-inspired Intelligent Materials and Devices, East China Normal University, Shanghai 200241, China}
\author{Di Wang}
\thanks{The corresponding author: diwang0214@nju.edu.cn.}
\affiliation{National Laboratory of Solid State Microstructures and School of Physics,
Nanjing University, Nanjing 210093, China}
\affiliation{Collaborative Innovation Center of Advanced Microstructures, Nanjing
University, Nanjing 210093, China}
\author{Huimei Liu}
\thanks{The corresponding author: huimeiliu@nju.edu.cn.}
\affiliation{National Laboratory of Solid State Microstructures and School of Physics,
Nanjing University, Nanjing 210093, China}
\affiliation{Collaborative Innovation Center of Advanced Microstructures, Nanjing
University, Nanjing 210093, China}
\author{Xin-Gao Gong}
\affiliation{Key Laboratory of Computational Physical Sciences (Ministry of Education), Institute of Computational Physical Sciences,
and Department of Physics, Fudan University, Shanghai 200433, China}
\affiliation{Hefei National Laboratory, Hefei 230088, China}
\author{Xiangang Wan}
\thanks{The corresponding author: xgwan@nju.edu.cn.}
\affiliation{National Laboratory of Solid State Microstructures and School of Physics,
Nanjing University, Nanjing 210093, China}
\affiliation{Collaborative Innovation Center of Advanced Microstructures, Nanjing
University, Nanjing 210093, China}
\affiliation{Hefei National Laboratory, Hefei 230088, China}
\affiliation{Jiangsu Physical Science Research Center, Nanjing University, Nanjing
210093, China}

\maketitle

\tableofcontents

\newpage
\section{Detailed description of our strategy based on irreducible-representation basis-vector, and take $\text{Mn}_3\text{GaN}$ as a demonstrative example}

\subsection{Irreducible-representation basis-vector strategy of initial magnetic structures}

Most magnetic phase transitions are continuous and can be described within the Landau framework~\cite{authier2014international}. 
From a symmetry perspective, the ordered phase is described by magnetic space groups (MSGs) that are subgroups of the parent crystallographic space group. 
However, the subgroup landscape is typically vast: a given parent space group admits many magnetic subgroups associated with many irreducible representations (irreps).

To systematically reduce this space, we take the magnetic moments $\boldsymbol{\mu}$ on the magnetic Wyckoff positions as a basis. 
For a crystal with $N$ magnetic atoms in the crystallographic unit cell (at $\mathbf{q}=0$), the $3N$ components of the local moments
$\boldsymbol{\mu}=(m_{1x},m_{1y},m_{1z},\dots,m_{Nx},m_{Ny},m_{Nz})$
span a representation $\Gamma_{\mathrm{mag}}$ of the parent space group, which is in general reducible and can be decomposed into irreducible representations as
\begin{equation}
\Gamma_{\mathrm{mag}}=\sum_{\oplus i} n_i\,\Gamma_i(j) .
\label{eq1}
\end{equation}
Here we adopt the Cracknell--Davies--Miller--Love (CDML) notation~\cite{Cracknell1979CDML}, where the subscript $i$ labels distinct irreducible representations, $j$ denotes the irrep dimensionality, and the prefactor $n_i$ specifies the multiplicity.

Within Landau theory, a continuous magnetic transition is driven by the instability of a single irreducible representation in Eq.~(\ref{eq1}).
Consequently, only the MSGs compatible with this unstable irrep need to be considered. Namely, only these irreps that actually appear in Eq.~(\ref{eq1}) are relevant, which substantially reduces the search space of candidate MSGs compared with a brute-force subgroup search, 
as shown in the Mn$_3$GaN example below.

In general, the magnetic structure is still not uniquely determined even after both the unstable irrep and its corresponding MSGs are fixed, except in the special case where $j=1$ and $n_i=1$.
In this special case where $\Gamma_{\mathrm{mag}}$ contains only one-dimensional irreps ($j=1$) and each irrep appears only once ($n_i=1$), the basis vectors of irreps are uniquely fixed. 
As a result, the magnetic structure is uniquely determined since there is no other freedom of the selection of basis vectors. 

However, $\Gamma_{\mathrm{mag}}$ generally contains multidimensional irreps ($j>1$) and/or repeated occurrences ($n_i>1$), as also demonstrated in the following benchmark section; in this situation, additional degrees of freedom remain within the irrep space.
This leads to the non-uniqueness of the magnetic configuration, even after the relevant irrep and its compatible MSGs are fixed.
A more proper strategy for constructing explicit magnetic configurations is therefore to employ the symmetry-adapted basis vectors of the irrep. 
Nevertheless, residual degrees of freedom may remain within this basis-vector description; in the following, we introduce two strategies to systematically constrain these freedoms and generate a finite set of predetermined magnetic structures.

\bigskip

\noindent\textit{Strategy I: multidimensional irreps ($j>1$).}
For multi-dimensional irreducible representations $\Gamma_i(j)$ with $j>1$ in Eq.~(\ref{eq1}), the set of the order parameter within the irrep space is not uniquely fixed, and different symmetry-allowed choices generally correspond to different MSGs. In principle, the physically realized order parameter could be determined by minimizing the higher-order terms of the Landau free energy. 
In the present work, however, we do not pursue such an explicit free-energy minimization. 
Instead, we adopt a symmetry-based criterion and retain \textbf{all} the maximal-symmetry magnetic subgroups among those compatible with the irrep in Eq.~(\ref{eq1}). Physically, ordering patterns belonging to these MSGs correspond to minimal symmetry breaking at the magnetic transition and therefore provide a natural representative set for screening~\cite{perez2015symmetry,Zhou-FeGe}. Consistent with this strategy, our benchmark shows that \textbf{100\%} of the surveyed materials follow the maximal-symmetry selection rule, as shown in the Benchmark section.

\bigskip

\noindent\textit{Strategy II: repeated irreps ($n_i>1$).}
A second source of non-uniqueness arises when a given irrep appears multiple times in the representation, i.e., $n_i>1$ in Eq.~(\ref{eq1}). 
In this case, multiple symmetry-equivalent sets of the basis vectors exist and can be linearly combined with one another, leading to an infinite number of possible predetermined magnetic configurations.
To systematically remove this redundancy and generate a finite set of configurations, we retain only those basis vectors that generate magnetic configurations with moments aligned along all possible high-symmetry crystallographic directions compatible with the corresponding MSGs. This strategy captures the majority of experimentally reported magnetic structures, as shown in the benchmark below.

\bigskip

\noindent\textbf{Example: Mn$_3$GaN.} We take Mn$_3$GaN as a representative example~\cite{Mn3GaN} to illustrate our workflow. Mn$_3$GaN belongs to the antiperovskite Mn$_3A$N family and has attracted considerable interest due to its noncollinear antiferromagnetism and its relevance to Hall-type transport responses, whose measured signals are highly sensitive to the underlying symmetry of the magnetic structure~\cite{PhysRevMaterials.3.044409,matsunami2015giant,PhysRevB.78.184414,PhysRevB.99.104428}.

Mn$_3$GaN crystallizes in the cubic space group $Pm\bar{3}m$ (No.~221)~\cite{Mn3GaN}. This parent symmetry admits \textbf{98} distinct MSGs and \textbf{10} inequivalent irreducible representations (counting each irrep only once), all of which can, in principle, serve as symmetry-breaking channels for magnetic ordering.
The \textbf{10} inequivalent irreducible representations of $Pm\bar{3}m$ are listed in Table~\ref{IRREP-221}.

\begin{table}[h]
\caption{Character table for the irreducible representations of the point group $m\bar{3}m$ (No.~32), corresponding to the $\Gamma$ point of crystallographic space group No.~221 ($Pm\bar{3}m$)\cite{alma991016971289704336}. The point group contains ten conjugacy classes, denoted as $\bm{C_1}$-$\bm{C_{10}}$. 
The symmetry operations in $\bm{C_1}$-$\bm{C_{10}}$ are listed as follows: \\
}
\begin{tabular}{ll}
$\bm{C_1}\colon 1$  & $\bm{C_2}\colon 2_{001}, 2_{010}, 2_{100}$ \\
$\bm{C_3}\colon 2_{01\bar{1}}, 2_{011}, 2_{1\bar{1}0}, 2_{\bar{1}01}, 2_{101}, 2_{110}$ & $\bm{C_4}\colon \ 3^-_{\bar{1}1\bar{1}}, 3^-_{1\bar{1}\bar{1}}, 3^+_{1\bar{1}\bar{1}}, 3^+_{\bar{1}\bar{1}1}, 3^+_{\bar{1}1\bar{1}}, 3^+_{111}, 3^-_{\bar{1}\bar{1}1}, 3^-_{111}$ \\
$\bm{C_5}\colon 4^+_{001}, 4^-_{010}, 4^+_{010}, 4^-_{001}, 4^+_{100}, 4^-_{100}$ & $\bm{C_6}\colon \bar{1}$  \\
$\bm{C_7}\colon m_{001}, m_{010}, m_{100}$ & $\bm{C_8}\colon  m_{01\bar{1}}, m_{011}, m_{1\bar{1}0}, m_{\bar{1}01}, m_{101}, m_{110}$   \\
$\bm{C_9}\colon \bar{3}^-_{\bar{1}1\bar{1}}, \bar{3}^-_{1\bar{1}\bar{1}}, \bar{3}^+_{1\bar{1}\bar{1}}, \bar{3}^+_{\bar{1}\bar{1}1}, \bar{3}^+_{\bar{1}1\bar{1}}, \bar{3}^+_{111}, \bar{3}^-_{\bar{1}\bar{1}1}, \bar{3}^-_{111}$ & $\bm{C_{10}}\colon \bar{4}^+_{001}, \bar{4}^-_{010}, \bar{4}^+_{010}, \bar{4}^-_{001}, \bar{4}^+_{100}, \bar{4}^-_{100}$                                                         
\end{tabular}

\vspace{0.5cm} 
\begin{tabular}{ccccccccccc}
\hline
                 & $C_1$ & $C_2$ & $C_3$ & $C_4$ & $C_5$ & $C_6$ & $C_7$ & $C_8$ & $C_9$ & $C_{10}$ \\ \hline
$\Gamma_{1}^{+}$ & 1     & 1     & 1     & 1     & 1     & 1     & 1     & 1     & 1     & 1        \\ \hline
$\Gamma_{1}^{-}$ & 1     & 1     & 1     & 1     & 1     & -1    & -1    & -1    & -1    & -1       \\ \hline
$\Gamma_{2}^{+}$ & 1     & 1     & -1    & 1     & -1    & 1     & 1     & -1    & 1     & -1       \\ \hline
$\Gamma_{2}^{-}$ & 1     & 1     & -1    & 1     & -1    & -1    & -1    & 1     & -1    & 1        \\ \hline
$\Gamma_{3}^{+}$ & 2     & 2     & 0     & -1    & 0     & 2     & 2     & 0     & -1    & 0        \\ \hline
$\Gamma_{3}^{-}$ & 2     & 2     & 0     & -1    & 0     & -2    & -2    & 0     & 1     & 0        \\ \hline
$\Gamma_{4}^{+}$ & 3     & -1    & -1    & 0     & 1     & 3     & -1    & -1    & 0     & 1        \\ \hline
$\Gamma_{4}^{-}$ & 3     & -1    & -1    & 0     & 1     & -3    & 1     & 1     & 0     & -1       \\ \hline
$\Gamma_{5}^{+}$ & 3     & -1    & 1     & 0     & -1    & 3     & -1    & 1     & 0     & -1       \\ \hline
$\Gamma_{5}^{-}$ & 3     & -1    & 1     & 0     & -1    & -3    & 1     & -1    & 0     & 1        \\ \hline
\end{tabular}
\label{IRREP-221}
\end{table}

Instead of considering all these \textbf{10} irreps in Table~\ref{IRREP-221} which are admitted by the parent space group $Pm\bar{3}m$, we take the local magnetic-moment components $\boldsymbol{\mu}$ of Mn, which occupy the $3c$ Wyckoff positions, as the basis to construct the representation for Mn$_3$GaN. Since the unit cell contains three Mn atoms ($N=3$), the magnetic degrees of freedom consist of $3N=9$ magnetic-moment components,
\begin{equation}
\boldsymbol{\mu}=(m_{1x},m_{1y},m_{1z},,m_{2x},m_{2y},m_{2z},,m_{3x},m_{3y},m_{3z}),
\end{equation}
which form a natural basis for the magnetic representation $\Gamma_{\mathrm{mag}}$ of the parent space group $G$.
Here, the subscripts $1$, $2$, and $3$ label the three Mn ions occupying the Wyckoff $3c$ positions at
$(x,y,z)=(\tfrac{1}{2},\tfrac{1}{2},0)$, $(\tfrac{1}{2},0,\tfrac{1}{2})$, and $(0,\tfrac{1}{2},\tfrac{1}{2})$, respectively. Decomposing the representation $\Gamma_{\mathrm{mag}}$ into irreducible representations yields,
\begin{equation}
\Gamma_{\mathrm{mag}} = 2\times \Gamma_4^+(3) \oplus 1\times \Gamma_5^+(3),
\label{irrep1}
\end{equation}
where the superscript $+$ denotes even parity under inversion. Both $\Gamma_4^+(3)$ and $\Gamma_5^+(3)$ are three-dimensional ($j=3$) irreps of the parent space group $Pm\bar{3}m$.

It is evident from Eq.~(\ref{irrep1}) that, incorporating the Mn atoms at the $3c$ Wyckoff positions reduces the set of irreps relevant for magnetic ordering of Mn$_3$GaN. Specifically, the original \textbf{10} irreps of the parent space group $Pm\bar{3}m$ are reduced to only \textbf{2} relevant irreps, $\Gamma_4^+$ and $\Gamma_5^+$. 
This irrep reduction immediately and substantially constrains the space of symmetry-allowed magnetic orderings.

As a consequence, instead of considering all \textbf{98} magnetic space groups compatible with $Pm\bar{3}m$, only the \textbf{9} magnetic space groups associated with $\Gamma_4^+$ and $\Gamma_5^+$ need to be examined, namely
$R\bar{3}m'$, $R\bar{3}m$, $P4/mm'm'$, $P4'/mm'm$, $Cmm'm'$, $C2'/m'$, $C2/m$, $P2'/m'$, and $P\bar{1}$.
This represents an effective reduction of the  MSG search space by approximately one order of magnitude.

For Mn$_3$GaN, the representation $\Gamma_{\mathrm{mag}}$ contains two copies of $\Gamma_4^+(3)$ and one copy of $\Gamma_5^+(3)$, i.e., $n_4=2$ and $n_5=1$ in Eq.~\eqref{irrep1}. Both irreducible representations are three-dimensional ($j=3$).
Mn$_3$GaN therefore provides a prototypical example in which both intrinsic sources of magnetic-structure non-uniqueness are present: 
(i) the freedom of the order parameter within a multidimensional irrep ($j>1$), and 
(ii) the basis ambiguity associated with repeated irreps ($n_i>1$).

We first address the ambiguity associated with multidimensional irreps by applying the maximal-symmetry criterion.
This further reduces the \textbf{9} symmetry-compatible magnetic space groups to a compact set of \textbf{5} maximal magnetic subgroups (with duplicated MSGs counted only once).
Specifically, the maximal-symmetry MSGs are $R\bar{3}m'$, $P4/mm'm'$, and $Cmm'm'$ for the $\Gamma_4^+$ channel, and $R\bar{3}m$, $P4'/mm'm$, and $Cmm'm'$ for the $\Gamma_5^+$ channel, as illustrated in Fig.~(\ref{max}).

In Mn$_3$GaN, the irreducible representation $\Gamma_4^+$ appears twice in the magnetic representation, i.e., $n_4=2$, and its dimensionality $j=3$.
As a direct consequence, two independent but symmetry-equivalent sets of symmetry-adapted basis vectors are associated with $\Gamma_4^+$.
These two basis sets, denoted as $\{\boldsymbol{\phi}^{(a)}_l\}$ with 
$a\in\{1,2\}$ labeling the two symmetry-equivalent copies of $\Gamma_4^+$ 
and $l=1,2,3$ labeling its dimensionality, are explicitly given by
\begin{equation}
\begin{aligned}
\boldsymbol{\phi}_{1}^{(1)} &= (1,0,0;\;1,0,0;\;0,0,0),\\
\boldsymbol{\phi}_{2}^{(1)} &= (0,1,0;\;0,0,0;\;0,1,0),\\
\boldsymbol{\phi}_{3}^{(1)} &= (0,0,0;\;0,0,1;\;0,0,1),
\end{aligned}
\label{eq:GM4_basis_set1}
\end{equation}
and
\begin{equation}
\begin{aligned}
\boldsymbol{\phi}_{1}^{(2)} &= (0,0,0;\;0,0,0;\;1,0,0),\\
\boldsymbol{\phi}_{2}^{(2)} &= (0,0,0;\;0,1,0;\;0,0,0),\\
\boldsymbol{\phi}_{3}^{(2)} &= (0,0,1;\;0,0,0;\;0,0,0).
\end{aligned}
\label{eq:GM4_basis_set2}
\end{equation}

We first apply the maximal-symmetry criterion (Strategy~I) to identify the candidate magnetic space groups associated with $\Gamma_4^+$. 
As shown in Fig.~\ref{max}, three maximal-symmetry MSGs are obtained, namely $R\bar{3}m'$, $P4/mm'm'$, and $Cmm'm'$. 
Taking the maximal magnetic subgroup $R\bar{3}m'$ (No.~166.101) as an example, the basis vectors of the $\Gamma_4^+$ irrep compatible with this MSG can be constructed as linear combinations of the irrep basis functions:
\begin{equation}
\boldsymbol{\eta}^{(1)} \propto \boldsymbol{\phi}_{1}^{(1)}+\boldsymbol{\phi}_{2}^{(1)}+\boldsymbol{\phi}_{3}^{(1)},\qquad
\boldsymbol{\eta}^{(2)} \propto \boldsymbol{\phi}_{1}^{(2)}+\boldsymbol{\phi}_{2}^{(2)}+\boldsymbol{\phi}_{3}^{(2)}.
\label{eq:Psi_def}
\end{equation}
 
In general, for the maximal MSG $R\bar{3}m'$ (No.~166.101), the basis vectors can be expressed as linear superpositions of these two basis sets,
\begin{equation}
\boldsymbol{\eta}=\alpha\,\boldsymbol{\eta}^{(1)}+\beta\,\boldsymbol{\eta}^{(2)},
\label{eq:etaL}
\end{equation}
where real numbers $\alpha$ and $\beta$ are free parameters, which reflects the intrinsic basis ambiguity associated with repeated irreducible representations ($n_i>1$).%, and in principle leads to infinite symmetry-allowed magnetic configurations.

For a given choice of $(\alpha,\beta)$, based on Eqs.~\eqref{eq:GM4_basis_set1}-\eqref{eq:etaL}, the resulting magnetic moments on the three Mn ions of Mn$_3$GaN can be written as:
\begin{equation}
\boldsymbol{\mu}\propto (\alpha  , \alpha , \beta  ;\ \alpha  , \beta , \alpha ; \beta ,  \alpha ,  \alpha ),
\label{mu_1}
\end{equation}
which illustrates that infinite magnetic configurations are symmetry-allowed at this stage.

Then, to construct a finite and physically relevant set of magnetic structures, we impose an additional constraint by retaining only those basis vectors that generate magnetic moments aligned along high-symmetry crystallographic directions.
For Mn$_3$GaN with space group $Pm\bar{3}m$, these typically directions include the fourfold ($[100]$, $[010]$, $[001]$), threefold ($[111]$, $[1\bar{1}1]$, $[\bar{1}11]$, $[11\bar{1}]$), and twofold ($[1\bar{1}0]$, $[110]$, $[01\bar{1}]$, $[011]$, $[\bar{1}01]$, $[101]$) rotational axes, as well as  in-plane directions perpendicular to the threefold axes ($[112]$, $[\bar{1}12]$, $[1\bar{1}2]$, $[\bar{1}\bar{1}2]$, 
$[121]$, $[\bar{1}21]$, $[12\bar{1}]$, $[\bar{1}2\bar{1}]$, 
$[211]$, $[2\bar{1}1]$, $[21\bar{1}]$, $[2\bar{1}\bar{1}]$)~\cite{hahn1983international}.

For MSG $R\bar{3}m'$ (No.~166.101) of Mn$_3$GaN, we take the Mn ion at $(\tfrac{1}{2},\tfrac{1}{2},0)$ as a representative site (the magnetic moments on the other two Mn ions are then fixed by applying the $C_3$ symmetry operation), the corresponding local magnetic moment is given by
\begin{equation}
(m_{1x},\,m_{1y},\,m_{1z}) \propto (\alpha,\,\alpha,\,\beta),
\end{equation}
which corresponds to the first three components of Eq. \eqref{mu_1}. 
By comparing this direction with the aforementioned 25 high-symmetry crystallographic directions of the space group $Pm\bar{3}m$, only 6 distinct possibilities are allowed.
These correspond to the following high-symmetry directions:
\begin{alignat}{5}
\label{direction1}
&[001] \; (\alpha=0,\beta=1), \ \ \ \ & \ \ \ \
&[111] \; (\alpha=\beta=1),  \ \ \ \ & \ \ \ \ \ \
&[\bar{1}\bar{1}1] \; (\alpha=-1,\beta=1), 
\notag \\
&[110] \; (\alpha=1,\beta=0),   &
&[112] \; (\alpha=1,\beta=2),  &
&[\bar{1}\bar{1}2] \; (\alpha=-1,\beta=2),
\end{alignat}
as summarized (a)-(f) panels in Table~\ref{Mn3}.
Since these configurations correspond to the maximal MSG $R\bar{3}m'$ (No.~166.101) associated with the irrep $\Gamma_4^+$, it can be constructed straightforwardly following the procedure in Eqs.~(\ref{eq:Psi_def})--(\ref{direction1}). 
In particular, the magnetic moment of the Mn ion at $(\tfrac{1}{2},\tfrac{1}{2},0)$ is constrained to and only to the six high-symmetry directions listed in Eq.~(\ref{direction1}). 
As an illustrative example, the configuration shown in panel~(a) of Table~\ref{Mn3} corresponds to choosing $\alpha=0$ and $\beta=1$ in Eq.~(\ref{direction1}), yielding the magnetic moment of Mn ion at $(\tfrac{1}{2},\tfrac{1}{2},0)$  aligned along the $[001]$ direction.

By repeating this procedure for all subgroups in Fig.~(\ref{max}), we obtain a total of 11 predetermined magnetic configurations for Mn$_3$GaN, see Table~\ref{Mn3} (including 7 noncollinear and 4 collinear magnetic configurations).

Although our irreducible-representation basis-vector strategy considers only 11 initial magnetic configurations, 
notably, the experimentally reported magnetic structure as in \textbf{panel~(k)} of Table~\ref{Mn3} is already included in this candidate set; this structure belongs to the $\Gamma_5^+$ irrep and corresponds to MSG $R\bar{3}m$ (No.~166.97).

More generally, as demonstrated in the Benchmark section below, the majority of experimental magnetic structure in the MAGNDATA database are captured by our irrep basis-vector strategy.
Consequently, with sufficiently accurate total-energy calculations, the correct magnetic structure can be identified by energy ranking within these compact candidate sets.

\begin{figure}[h]
\centering
\includegraphics[width=0.9\textwidth]{Mn3GaN\_GM.png}
\caption{\textbf{Symmetry-compatible MSGs for Mn$_3$GaN.} 
Maximal-symmetry candidate MSGs associated with the irreducible representations $\Gamma_4^+$ and $\Gamma_5^+$.}
\label{max}
\end{figure}

\subsection{First-principles total-energy screening for the magnetic structure}

Based on the finite number of initial states selected by our irrep basis-vector strategy, first-principles total-energy calculations were then performed among these well-selected structures using the Vienna Ab initio Simulation Package (VASP) \cite{vasp1,vasp2}, employing a spin-polarized GGA + SOC + $U$ approach.  The Coulomb interaction parameters $U$ and Hund $J$ were taken as the averaged values recommended for transition-metal elements based on the linear-response scheme \cite{Uvalue}. 
The $k$-mesh of the Brillouinzone is set by 60/$a$ along each direction, where $a$ denotes the length of the lattice constant in Å.

For Mn$_3$GaN, $U$ and $J$ were set to $U = 4.8$ eV and $J = 0.7$ eV.  A $17\times17\times17$ $k$-point mesh was employed for the first-principles calculations. By comparing the total energies of the 11 candidate magnetic configurations listed in Table~\ref{Mn3}, we identify the magnetic structure of Mn$_3$GaN as the one shown in \textbf{panel~(k)}, which belongs to the $\Gamma_5^+(3)$ irrep in Eq.~\eqref{irrep1} and corresponds to the MSG $R\bar{3}m$ (No.~166.97), consistent with the experimentally reported ground state~\cite{Mn3GaN}.

\begin{table}
\caption{Candidate magnetic structures for Mn$_3$GaN, generated using our irreducible-representation basis-vector strategy. For each configuration, we list the magnetic structure, the associated irreducible representation, MSG and the magnetic moment direction of the Mn atom at $(\tfrac{1}{2}, \tfrac{1}{2}, 0)$, which is chosen as a representative site to visualize the noncollinear nature of different magnetic configurations.}
\begin{tabular}{|c|c|c|c|c|}
\hline
\begin{tabular}[c]{@{}c@{}}Magnetic \\ Configration\end{tabular}               
 & \multicolumn{1}{c|}{
\rule{0pt}{1.8cm}
\begin{minipage}[c]{0.2\columnwidth}
\centering
\includegraphics[height=3cm]{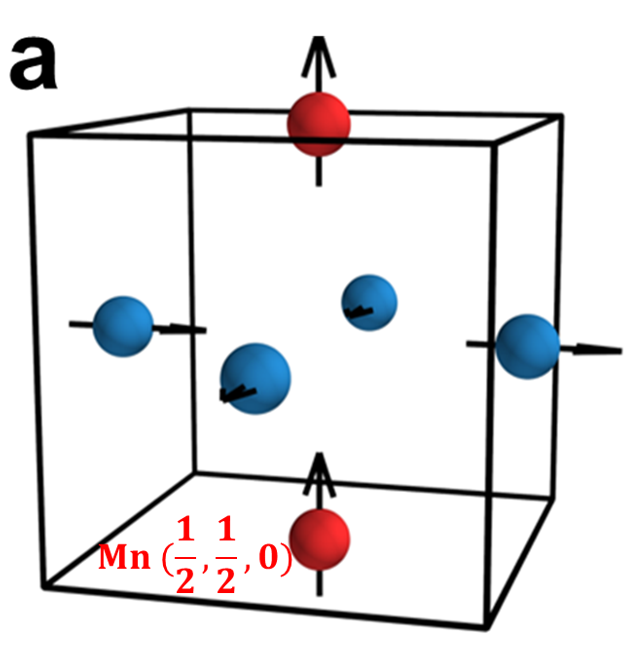}
\end{minipage}
}
 & \multicolumn{1}{c|}{
\rule{0pt}{1.8cm}
\begin{minipage}[c]{0.2\columnwidth}
\centering
\includegraphics[height=3cm]{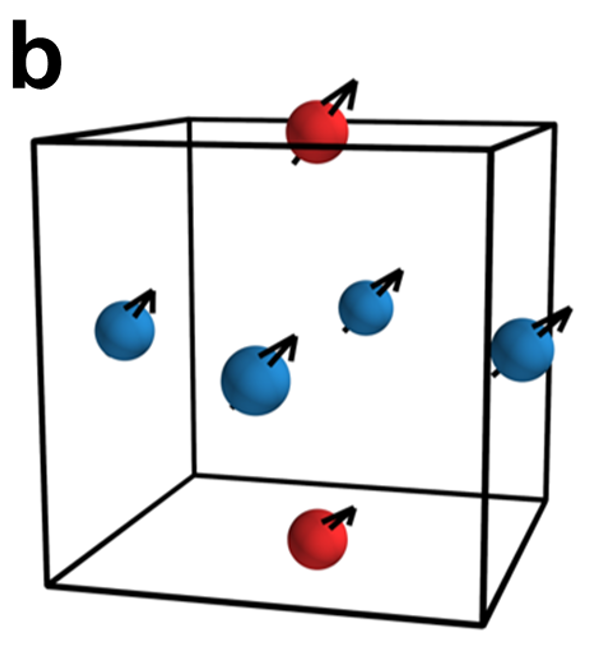}
\end{minipage}
}                
 & \multicolumn{1}{c|}{
\rule{0pt}{1.8cm}
\begin{minipage}[c]{0.2\columnwidth}
\centering
\includegraphics[height=3cm]{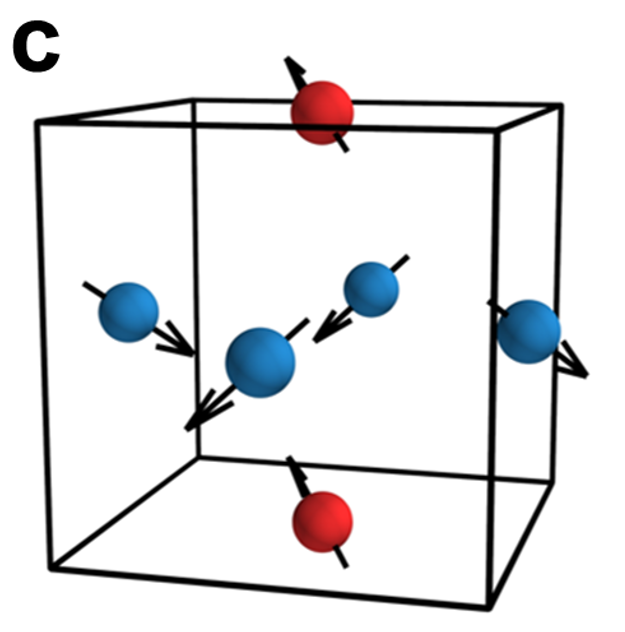}
\end{minipage}
}                
 & \multicolumn{1}{c|}{
\rule{0pt}{1.8cm}
\begin{minipage}[c]{0.2\columnwidth}
\centering
\includegraphics[height=3cm]{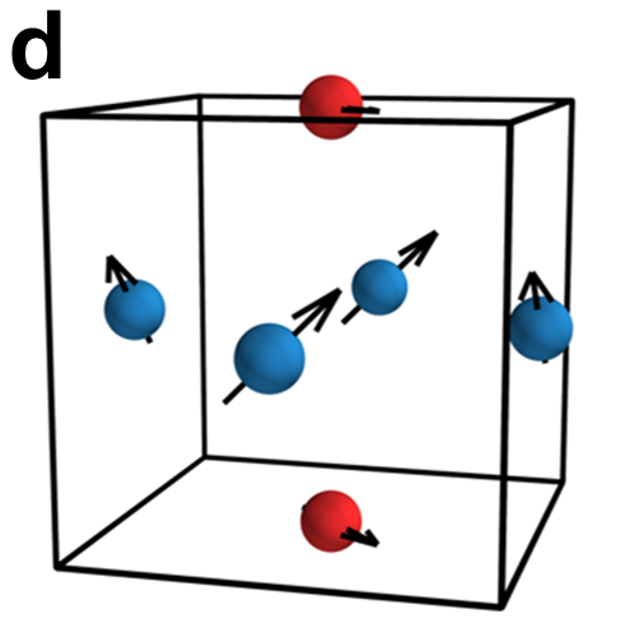}
\end{minipage}
}                 \\ \cline{1-1}
\begin{tabular}[c]{@{}c@{}}Irreducible \\ Representations\end{tabular}           & $\Gamma_{4}^{+}$ & $\Gamma_{4}^{+}$ & $\Gamma_{4}^{+}$ & $\Gamma_{4}^{+}$ \\\cline{1-1}
MSG  & $R\bar{3}m'$ (166.101)          & $R\bar{3}m'$ (166.101)           & $R\bar{3}m'$ (166.101)            & $R\bar{3}m'$ (166.101)            \\ \cline{1-1}
\begin{tabular}[c]{@{}c@{}}Moment Direction \\ of Mn (1/2, 1/2, 0)\end{tabular} & [001]        & [111]      & [$\bar{1}\bar{1}1$] & [110]        \\ \hline
\begin{tabular}[c]{@{}c@{}}Magnetic \\ Configration\end{tabular}
 & \multicolumn{1}{c|}{
\rule{0pt}{1.8cm}
\begin{minipage}[c]{0.2\columnwidth}
\centering
\includegraphics[height=3cm]{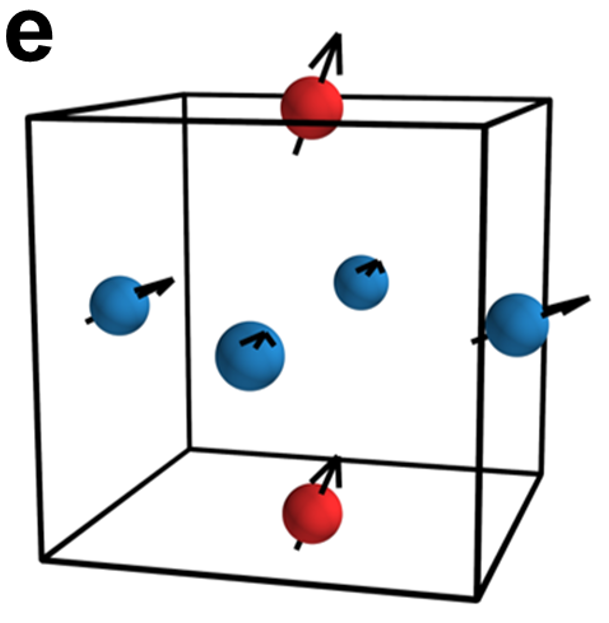}
\end{minipage}
}
& \multicolumn{1}{c|}{
\rule{0pt}{1.8cm}
\begin{minipage}[c]{0.2\columnwidth}
\centering
\includegraphics[height=3cm]{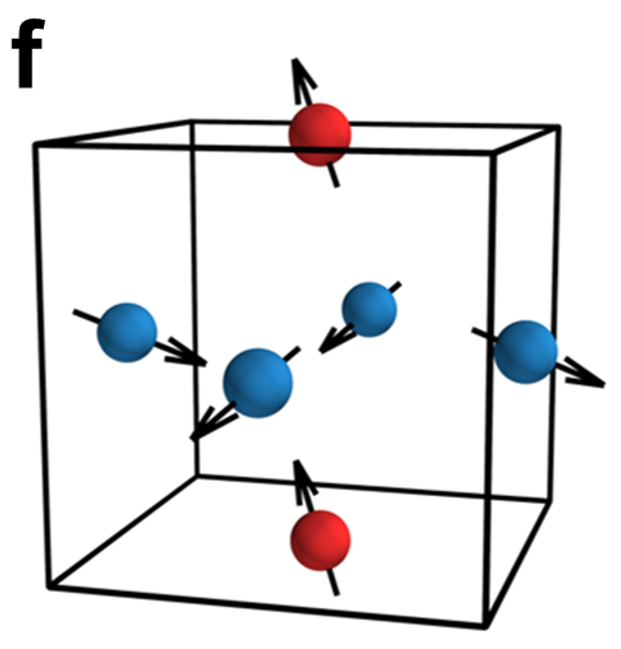}
\end{minipage}
}
 & \multicolumn{1}{c|}{
\rule{0pt}{1.8cm}
\begin{minipage}[c]{0.2\columnwidth}
\centering
\includegraphics[height=3cm]{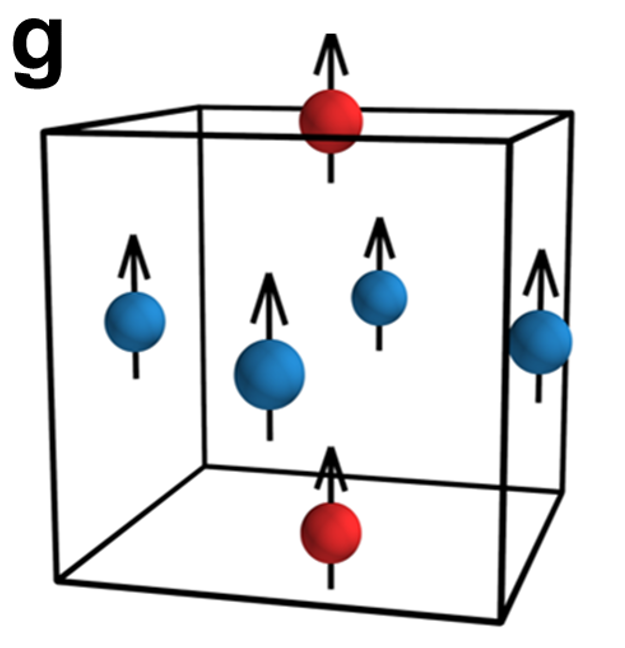}
\end{minipage}
}
 & \multicolumn{1}{c|}{
\rule{0pt}{1.8cm}
\begin{minipage}[c]{0.2\columnwidth}
\centering
\includegraphics[height=3cm]{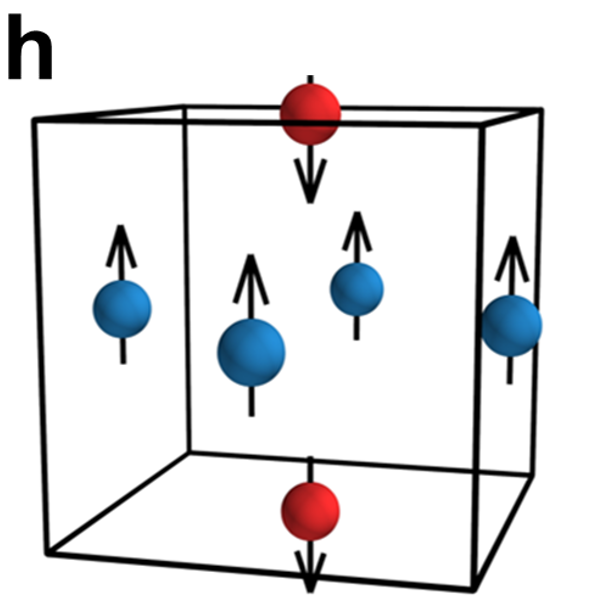}
\end{minipage}
}                 \\ \cline{1-1}
\begin{tabular}[c]{@{}c@{}}Irreducible \\ Representations\end{tabular}           & $\Gamma_{4}^{+}$ & $\Gamma_{4}^{+}$ & $\Gamma_{4}^{+}$ & $\Gamma_{4}^{+}$ \\ \cline{1-1}
MSG  & $R\bar{3}m'$ (166.101)            & $R\bar{3}m'$ (166.101)            & $P4/mm'm'$ (123.345)          & $P4/mm'm'$ (123.345)         \\ \cline{1-1}
\begin{tabular}[c]{@{}c@{}}Moment Direction \\ of Mn (1/2, 1/2, 0)\end{tabular} & [112]        & [$\bar{1}\bar{1}2$]        & [001]        & [00$\bar{1}$]       \\ \hline
\begin{tabular}[c]{@{}c@{}}Magnetic \\ Configration\end{tabular}
 & \multicolumn{1}{c|}{
\rule{0pt}{1.8cm}
\begin{minipage}[c]{0.2\columnwidth}
\centering
\includegraphics[height=3cm]{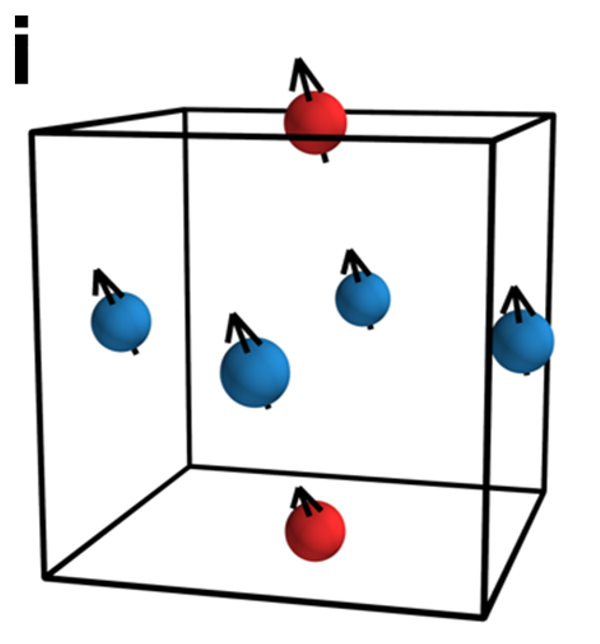}
\end{minipage}
} 
 &  \multicolumn{1}{c|}{
\rule{0pt}{1.8cm}
\begin{minipage}[c]{0.2\columnwidth}
\centering
\includegraphics[height=3cm]{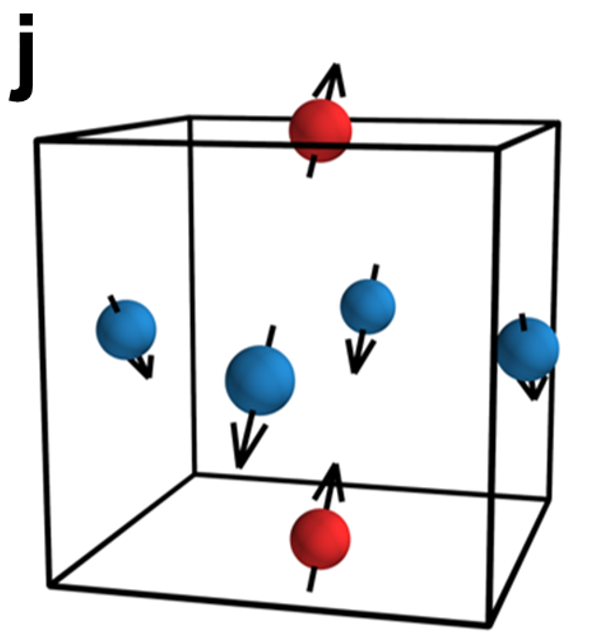}
\end{minipage}
} &  \multicolumn{1}{c|}{
\rule{0pt}{1.8cm}
\begin{minipage}[c]{0.2\columnwidth}
\centering
\includegraphics[height=3cm]{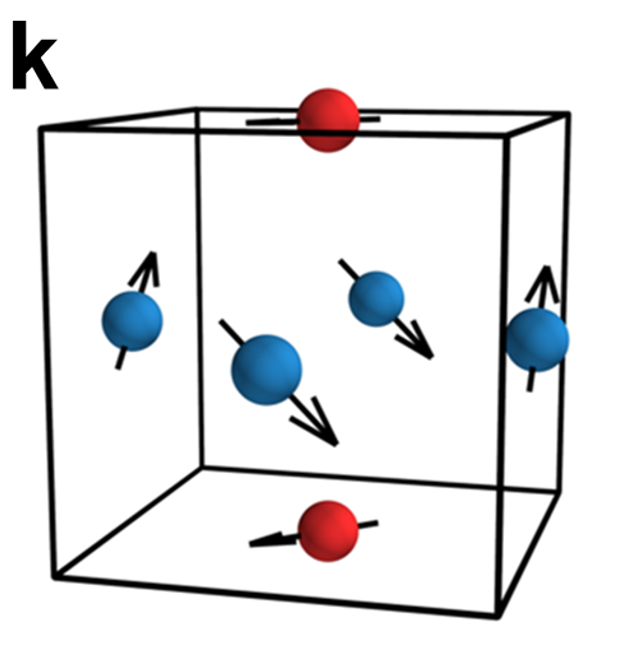}
\end{minipage}
} &  \\ \cline{1-1}
\begin{tabular}[c]{@{}c@{}}Irreducible \\ Representations\end{tabular}           & $\Gamma_{4}^{+}$ & $\Gamma_{4}^{+}$ & $\Gamma_{5}^{+}$ &                  \\ \cline{1-1}
MSG  & $Cmm'm'$(65.486)           & $Cmm'm'$(65.486)           & $R\bar{3}m$ (166.97)           &                  \\ \cline{1-1}
\begin{tabular}[c]{@{}c@{}}Moment Direction \\ of Mn (1/2, 1/2, 0)\end{tabular} & [101]        & [$\bar{1}01$]       & [1$\bar{1}0$]       &                  \\ \hline
\end{tabular}
\label{Mn3}
\end{table}
\clearpage

\section{Details of Benchmark Testing Using the MAGNDATA Database}

The discrepancies between the magnetic structure obtained from our irrep basis-vector strategy and the experimentally reported magnetic structures originate from two distinct factors:
(1) the experimental magnetic structure is not included in the set of our initial candidate magnetic configurations. 
This limitation is intrinsic to our irrep basis-vector strategy, arising from our ``all possible high-symmetry crystallographic directions compatible with the corresponding irrep'' strategy used to address the presence of repeated irreducible representations (i.e., $n_i>1$ in Eq.~(\ref{eq1}));
(2) the experimental magnetic structure is included in the initial input set, but first-principles total-energy calculations fail to identify it as the lowest-energy state.
The latter issue is, in principle, addressable through enhanced computational resources and more efficient algorithms. 

In the following, we benchmark these two aspects separately by systematically examining experimentally established magnetic structures documented in the MAGNDATA database~\cite{gallego2016magndata}.

\subsection{Accuracy of our Strategy for Selecting Input Magnetic Structures}

We restrict our analysis to stoichiometric materials with fewer than 40 atoms per unit cell and a zero propagation vector ($\mathbf{q}=0$). Only materials that explicitly contain transition-metal ions are considered, while lanthanoid and actinoid ions are excluded due to the challenges in accurately described within standard density functional theory \cite{kotliar2006electronic}.
These criteria reduce the MAGNDATA dataset to 328 materials, which serve as benchmark cases for evaluating our irrep basis-vector strategy.

Among these 328 materials, 26 entries do not satisfy the criteria for continuous magnetic phase transitions considered in this work, as  they cannot be characterized by a single irreducible representation of the crystallographic space group, which possibly due to the structural phase transitions, magnetoelastic coupling, etc. Detailed information on these 26 magnetic materials is provided in Table \ref{table2irrep}. 
The remaining 302 materials therefore fall within the applicability range of our irrep basis-vector strategy.

We first analyze the magnetic structure of these 302 materials as reported in MAGNDATA. Among them, 
the experimental magnetic structure of 76 materials correspond to a one-dimensional irreducible representation appearing only once, i.e., the case with  $j=1$ and $n_i=1$ in Eq. (\ref{eq1}), as listed in Table \ref{n1j1}. In this situation, the associated basis vectors of this irrep are uniquely fixed by symmetry, and consequently, the magnetic structure is uniquely determined without additional constraints. These cases therefore admit no any ambiguity and are fully captured by our framework by construction, namely, the magnetic structures of these materials
are included in our initial magnetic configuration set.

We now turn to examine the ambiguity associated with multidimensional irreducible representations (i.e., cases with $n_i=1$ and $j>1$ in Eq. (\ref{eq1})). 
For such cases, the
order parameter within the irrep space is not uniquely determined, corresponding to different MSGs, giving rise to an intrinsic ambiguity in the  magnetic configurations. Among the remaining 226 materials in our benchmark set, 12 fall into this category, as summarized in Table~\ref{n1j3}.
To resolve this ambiguity, our irrep basis-vector strategy adopts a maximal-symmetry criterion: instead of attempting to determine the order-parameter direction by explicitly minimizing higher-order Landau free-energy terms, we retain the magnetic structures associated with maximal symmetry magnetic subgroups compatible with the given multidimensional irrep. Remarkably, without exception, the experimentally reported magnetic structure of all 12 materials are consistent with this maximal magnetic subgroup scenario.
This benchmark therefore demonstrates that the maximal-symmetry criterion resolves the ambiguity associated with multidimensional irreducible representations ($j>1$) with \textbf{100\% success} for all materials examined — meaning the corresponding magnetic structures are also successfully contained within our set of initial magnetic configurations.

We then turn to the ambiguity arising from repeated irreducible representations ($n_i>1$). Among the remaining 214 materials, magnetic moments deviate from high-symmetry directions in 49 materials, which fall outside the scope of our irrep basis-vector strategy, as summarized in Table~\ref{Non-highsym}. The remaining 165 cases exhibit magnetic moments aligned along high-symmetry directions and are therefore successfully captured by our irrep basis-vector strategy, as listed in Table \ref{165}. 

Consequently, for 253 out of the 302 benchmark materials (83.8\%), the experimentally reported magnetic structure fall within the very limited ($\sim$20) candidate set generated by our irrep basis-vector strategy.

\newpage 

\begin{table*}[h]
\caption{A detailed list of 26 magnetic structures incompatible with a continuous phase transition is provided, including the MAGNDATA labels, chemical formulas, crystallographic space groups, magnetic space groups, and irreducible representations of the crystallographic space group. Material names are followed by their corresponding labels (in parentheses) from the MAGNDATA database \cite{gallego2016magndata}.}
\begin{tabular}{llll}
\hline
 Materials & Crystallographic space group & Magnetic space group  & Irreps \\ \hline
Fe$_{4}$O$_{5}$ (0.999) \cite{0.1000} & $Cmcm$ (No.63) & $Cm'c2_1'$ (No.36.174) & $\Gamma_{3}^{-}$, $\Gamma_{4}^{+}$ \\ 
Fe$_4$O$_5$ (0.1000)  \cite{0.1000} & $Cmcm$ (No.63) & $P2_1'$ (No.4.9) & $\Gamma_{3}^{-}$, $\Gamma_{4}^{+}$, $\Gamma_{3}^{+}$ \\
BaFe$_2$Se$_4$ (0.1024)\cite{0.1024} & $I4/m$ (No.87) & $C2'$ (No.5.15) & $\Gamma_{3}^{+}\Gamma_{4}^{+}$, $\Gamma_{3}^{-}\Gamma_{4}^{-}$ \\
Mn$_3$Si$_2$Te$_6$ (0.1026)\cite{0.1026} & $P\bar{3}1c$ (No.163) & $C2'/c'$ (No.15.89) & $\Gamma_{3}^{+}$, $\Gamma_{2}^{+}$ \\
LuFe$_{4}$Ge$_{2}$ (0.140)\cite{0.140} & $P4_2/mnm$ (No.136) & $Pn'n'm'$ (No.58.399) & $\Gamma_{2}^{-}$, $\Gamma_{2}^{+}$ \\
LiFePO$_{4}$ (0.152)\cite{0.152} & $Pnma$ (No.62) & $P2_1/c'$ (No.14.78) & $\Gamma_{2}^{-}$, $\Gamma_{1}^{-}$ \\
CaMnGe$_{2}$O$_{6}$ (0.155) \cite{0.155} & $C2/c$ (No.15) & $P\bar{1}'$ (No.2.6) & $\Gamma_{2}^{-}$, $\Gamma_{1}^{-}$ \\
SrMn(VO$_{4}$)(OH) (0.165)\cite{0.165} & $P2_12_12_1$ (No.19) & $P2_1$ (No.4.7) &$\Gamma_{1}$, $\Gamma_{3}$ \\
FePO$_{4}$ (0.17) \cite{0.17} & $Pnma$ (No.62) & $P2_12_12_1$ (No.19.25) & $\Gamma_{1}^{-}$, $\Gamma_{1}^{+}$ \\
Co$_{4}$Nb$_{2}$O$_{9}$ (0.196) \cite{0.196} & $P\bar{3}c1$ (No.165) & $C2/c'$ (No.15.88) & $\Gamma_{3}^{-}$, $\Gamma_{1}^{-}$ \\
Mn$_{3}$Ge (0.203)\cite{0.203} & $P6_3/mmc$ (No.194) & $C2'/m'$ (No.12.62) & $\Gamma_{6}^{+}$, $\Gamma_{2}^{+}$ \\
RbMnF$_{4}$ (0.329)\cite{0.329} & $P2_1/a$ (No.14) & $P\bar{1}$ (No.2.4) & $\Gamma_{1}^{+}$, $\Gamma_{2}^{+}$ \\
LiCoPO$_{4}$ (0.384)\cite{0.384} & $Pnma$ (No.62) & $P2_1'/c$ (No.14.77) &$\Gamma_{2}^{-}$, $\Gamma_{4}^{-}$ \\
LiCoPO$_{4}$ (0.385)\cite{0.385} & $Pnma$ (No.62) & $P2_1/c'$ (No.14.78) & $\Gamma_{2}^{-}$, $\Gamma_{1}^{-}$ \\
YMnO$_{3}$ (0.44)\cite{0.44} & $P6_3cm$ (No.185) & $P6_3'$ (No.173.131) & $\Gamma_{3}$, $\Gamma_{4}$ \\
La$_{2}$NiO$_{4}$ (0.45)\cite{0.45} & $P4_2/ncm$ (No.138) & $Pc'c'n$ (No.56.369) & $\Gamma_{3}^{+}$, $\Gamma_{4}^{+}$ \\
Cr$_{2}$S$_{3}$ (0.5)\cite{0.5} & $R\bar{3}$ (No.148) & $P\bar{1}$ (No.2.4) & $\Gamma_{2}^{+}\Gamma_{3}^{+}$, $\Gamma_{1}^{+}$ \\
NaCrSi$_{2}$O$_{6}$ (0.504)\cite{0.504} & $C2/c$ (No.15) & $P\bar{1}'$ (No.2.6) & $\Gamma_{1}^{-}$, $\Gamma_{2}^{-}$ \\
CaMn$_{2}$Sb$_{2}$ (0.523)\cite{0.523} & $P\bar{3}m1$ (No.164) & $P\bar{1}'$ (No.2.6) & $\Gamma_{3}^{-}$, $\Gamma_{1}^{-}$  \\
CaMnGe (0.601)\cite{0.601} & $P4/nmm$ (No.129) & $P2_1/m'$ (No.11.53) & $\Gamma_{2}^{-}$, $\Gamma_{5}^{-}$ \\
CaMnGe (0.602)\cite{0.601} & $P4/nmm$ (No.129) & $P2_1/m'$ (No.11.53) &$\Gamma_{2}^{-}$, $\Gamma_{5}^{-}$ \\
Mn$_{3}$Ga (0.641)\cite{0.641} & $I4/mmm$ (No.139) & $C2'/m'$ (No.12.62) & $\Gamma_{3}^{+}$, $\Gamma_{5}^{+}$ \\
YVO$_{3}$ (0.788)\cite{0.788} & $P2_1/b11$ (No.14) & $P\bar{1}$ (No.2.4) & $\Gamma_{1}^{+}$, $\Gamma_{2}^{+}$ \\
NbMnP (0.803) \cite{0.803} & $Pnma$ (No.62) & $Pm'n2_1'$ (No.31.125) & $\Gamma_{3}^{+}$, $\Gamma_{4}^{-}$ \\
Fe$_{2}$WO$_{6}$ (0.812) \cite{0.812} & $Pbcn$ (No.60) &  $Pn'c2'$ (No.30.113) & $\Gamma_{3}^{+}$, $\Gamma_{2}^{-}$ \\
FeSb$_{2}$O$_{4}$ (0.97) \cite{0.97} & $P4_2/mbc$ (No.135) & $Pmc2_1$ (No.26.66) & $\Gamma_{2}^{+}$, $\Gamma_{5}^{-}$ \\

\hline
\end{tabular}
\label{table2irrep}
\end{table*}

%%%%%%%%    n=1j=1的表格
\begin{table}[]
\caption{Table of 76 materials with experimental magnetic structure corresponding to a one-dimensional irreducible representation appearing only once [$j$=1, $n_i$=1 in Eq. (\ref{eq1})]. Material names are followed by their corresponding labels (in parentheses) from the MAGNDATA database \cite{gallego2016magndata}.}
\begin{tabular}{cccc}
\hline
\multicolumn{4}{c}{Materials}                                                                                                                                \\ \hline
AlFe$_{2}$B$_{2}$ (0.414)   & Ba$_{2}$Mn$_{3}$Sb$_{2}$O$_{2}$ (0.471)  & Ba$_{2}$MnSi$_{2}$O$_{7}$ (0.229)        & BaCr$_{2}$As$_{2}$ (0.365)               \\
BaMn$_{2}$As$_{2}$ (0.18)   & BaMn$_{2}$Bi$_{2}$ (0.89)                & BaMn$_{2}$Ge$_{2}$ (0.605)               & BaMn$_{2}$Ge$_{2}$ (0.606)               \\
BaMn$_{2}$P$_{2}$ (0.464)   & BaMn$_{2}$Sb$_{2}$ (0.470)               & BaMnSb$_{2}$ (0.611)                     & Bi$_{2}$CuO$_{4}$ (0.348)                \\
Bi$_{2}$CuO$_{4}$ (0.694)   & CaMn$_{2}$Ge$_{2}$ (0.603)               & CaMn$_{2}$Ge$_{2}$ (0.604)               & CaMnBi$_{2}$ (0.72)                      \\
CaMnSi (0.599)              & CaMnSi (0.600)                           & CoF$_{2}$ (0.178)                        & CoF$_{3}$ (0.334)                        \\
CoTa$_{4}$Se$_{8}$ (0.1036) & Cr$_{2}$O$_{3}$ (0.59)                   & CrNb$_{4}$S$_{8}$ (0.708)                & CrSb (0.528)                             \\
Fe$_{2}$TeO$_{6}$ (0.142)   & Fe$_{2}$TeO$_{6}$ (0.960)                & FeCO$_{3}$ (0.116)                       & KFeSe$_{2}$ (0.637)                      \\
KMnBi (0.618)               & KMnF$_{3}$ (0.433)                       & KMnSb (0.617)                            & KOsO$_{4}$ (0.284)                       \\
KRuO$_{4}$ (0.285)          & La$_{2}$O$_{3}$Mn$_{2}$Se$_{2}$ (0.1091) & La$_{2}$O$_{3}$Mn$_{2}$Se$_{2}$ (0.1092) & La$_{2}$O$_{3}$Mn$_{2}$Se$_{2}$ (0.1093) \\
LaBaMn$_{2}$O$_{6}$ (0.737) & LaBaMn$_{2}$O$_{6}$ (0.738)              & LaCrO$_{3}$ (0.416)                      & LaMn$_{2}$Si$_{2}$ (0.472)               \\
LaMn$_{2}$Si$_{2}$ (0.498)  & LaMnAsO (0.619)                          & LaMnAsO (0.624)                          & LaMnSbO (0.667)                          \\
LaMnSi$_{2}$ (0.778)        & LaMnSi$_{2}$ (0.779)                     & LaMnSi$_{2}$ (0.780)                     & LiCoPO$_{4}$ (0.193)                     \\
LiCoPO$_{4}$ (0.383)        & LiFe$_{2}$F$_{6}$ (0.501)                & LiFePO$_{4}$ (0.95)                      & MgMnO$_{3}$ (0.277)                      \\
MnF$_{2}$ (0.15)            & MnGeO$_{3}$ (0.125)                      & MnTe$_{2}$ (0.20)                        & NaMnAs (0.629)                           \\
NaMnAs (0.630)              & NaMnBi (0.634)                           & NaMnBi (0.635)                           & NaMnP (0.626)                            \\
NaMnP (0.627)               & NaMnP (0.628)                            & NaMnSb (0.631)                           & NaMnSb (0.632)                           \\
NiCrO$_{4}$ (0.896)         & NiS$_{2}$ (0.150)                        & PbNiO$_{3}$ (0.21)                       & RbFeSe$_{2}$ (0.638)                     \\
RuO$_{2}$ (0.607)           & Sr$_{2}$Mn$_{3}$As$_{2}$O$_{2}$ (0.212)  & Sr$_{4}$Fe$_{4}$O$_{11}$ (0.401)         & SrCr$_{2}$As$_{2}$ (0.364)               \\
SrMnBi$_{2}$ (0.73)         & SrMnSb$_{2}$ (0.767)                     & YMnO$_{3}$ (0.6)                         & [Na(OH)$_{2}$]$_{3}$Mn(NCS)$_{3}$ (0.1078)                  \\ \hline
\end{tabular}
\label{n1j1}
\end{table}

%%%%%%%%    n=1j>1的表格
\begin{table}[]
\caption{Table of 12 materials with multidimensional irreducible representations appearing only once [$n_i=1$ and $j>1$ in Eq. (\ref{eq1})]. All of their experimental magnetic structures fall in the scope of our irrep basis-vector strategy. Material names are followed by their corresponding labels (in parentheses) from the MAGNDATA database \cite{gallego2016magndata}.}
\begin{tabular}{cccc}
\hline
\multicolumn{4}{c}{Materials}                                                                           \\ \hline
CaMn$_{2}$Sb$_{2}$ (0.92) & Mn$_{2}$Au (0.1081) & Mn$_{2}$Au (0.639)         & Mn$_{2}$Au (0.640)       \\
Mn$_{3}$GaN (0.177)       & Mn$_{3}$ZnN (0.273) & MnNb$_{4}$S$_{8}$ (0.709)  & MnPtGa (0.395)           \\
MnTa$_{4}$S$_{8}$ (0.711) & MnTe (0.800)        & SrMn$_{2}$As$_{2}$ (0.482) & VNb$_{3}$S$_{6}$ (0.712) \\ \hline
\end{tabular}
\label{n1j3}
\end{table}

%%%%%%%%    n>1的表格，不沿高对称方向的表格
\begin{table}[]
\caption{Table of 49 materials cannot be described by our method due to deviations of magnetic moments from high-symmetry directions, correspondng to the case when irreducible representations appeared multiple times [$n_i>1$ in Eq.~\eqref{eq1}] . Material names are followed by their corresponding labels (in parentheses) from the MAGNDATA database \cite{gallego2016magndata}.}
\begin{tabular}{ccccc}
\hline
\multicolumn{5}{c}{Materials}                                                                                                                                            \\ \hline
Ag$_{2}$RuO$_{4}$ (0.918)       & BaFe$_{2}$Se$_{2}$O (0.988)        & BaMnFeF$_{7}$ (0.577)      & Ca$_{2}$MnReO$_{6}$ (0.204)        & Ca$_{2}$RuO$_{4}$ (0.398)       \\
CaFe$_{5}$O$_{7}$ (0.357)       & Co$_{2}$SiO$_{4}$ (0.218)          & Co$_{2}$SiO$_{4}$ (0.219)  & Co$_{4}$Nb$_{2}$O$_{9}$ (0.197)    & Co$_{4}$Nb$_{2}$O$_{9}$ (0.529) \\
Co$_{4}$Ta$_{2}$O$_{9}$ (0.511) & CoFePO$_{5}$ (0.262)               & CoSO$_{4}$ (0.571)         & CoSO$_{4}$ (0.96)                  & CoSe$_{2}$O$_{5}$ (0.119)       \\
Cr$_{2}$F$_{5}$ (0.576)         & Cs$_{2}$Cu$_{3}$SnF$_{12}$ (0.506) & CsMn$_{2}$F$_{6}$ (0.726)  & Cu$_{2}$(OD)$_3$Cl (0.295)               & Cu$_{2}$OSO$_{4}$ (0.612)       \\
Fe(N(CN$_{2}$))$_2$ (0.132)             & Fe$_{2}$SeO (0.1061)               & Fe$_{2}$SiO$_{4}$ (0.1072) & Fe$_{2}$SiO$_{4}$ (0.221)          & Fe$_{2}$WO$_{6}$ (0.809)        \\
Fe$_{2}$WO$_{6}$ (0.810)        & GaV$_{4}$S$_{8}$ (0.756)           & KMnF$_{4}$ (0.328)         & La$_{2}$CoIrO$_{6}$ (0.375)        & LiNiPO$_{4}$ (0.88)             \\
Mn$_{2}$GeO$_{4}$ (0.101)       & Mn$_{2}$GeO$_{4}$ (0.102)          & Mn$_{2}$SiO$_{4}$ (0.220)  & Mn$_{3}$CoGe (0.900)               & Mn$_{3}$IrGe (0.899)            \\
Mn$_{3}$IrSi (0.898)            & Mn$_{3}$RhGe (0.1005)              & Mn$_{3}$Sn$_{2}$ (0.663)   & MnNb$_{2}$O$_{6}$ (0.819)          & MnPtGa (0.396)                  \\
MnTa$_{2}$O$_{6}$ (0.818)       & MnV$_{2}$O$_{4}$ (0.64)            & RbRuO$_{4}$ (0.924)        & SrCo(VO$_{4}$)(OH) (0.287)             & SrFe$_{2}$S$_{2}$O (0.762)      \\
SrFe$_{2}$Se$_{2}$O (0.761)     & Y$_{2}$MnCoO$_{6}$ (0.164)         & YFe$_{4}$Ge$_{2}$ (0.27)   & ZrCo$_{2}$Ge$_{4}$O$_{12}$ (0.314) &                                 \\ \hline
\end{tabular}
\label{Non-highsym}
\end{table}

%%%%%%%%    n>1的表格，沿高对称方向的表格
\begin{table}[]
\caption{Table of 165 materials with experimental magnetic moments aligned along high-symmetry directions and compatible with our irrep basis-vector strategy, in the presence of repeated irreducible representations [$n_i>1$, in Eq. (\ref{eq1})]. Material names are followed by their corresponding labels (in parentheses) from the MAGNDATA database \cite{gallego2016magndata}.}
\begin{tabular}{ccccc}
\hline
\multicolumn{5}{c}{Materials}                                                                                                                                                             \\ \hline
Ba$_{2}$CoGe$_{2}$O$_{7}$ (0.56) & Ba$_{3}$NiRu$_{2}$O$_{9}$ (0.748) & BaCrF$_{5}$ (0.303)                        & BaCuF$_{4}$ (0.191)              & BaFe$_{2}$S$_{2}$O (0.987)         \\
BaNi$_{2}$P$_{2}$O$_{8}$ (0.215) & Bi$_{2}$CuO$_{4}$ (0.695)         & BiCrO$_{3}$ (0.138)                        & Ca$_{2}$Fe$_{2}$O$_{5}$ (0.1080) & Ca$_{2}$FeOsO$_{6}$ (0.682)        \\
Ca$_{2}$MnGaO$_{5}$ (0.825)      & Ca$_{2}$NiOsO$_{6}$ (0.796)       & CaCu$_{3}$Fe$_{2}$Sb$_{2}$O$_{12}$ (0.672) & CaFe$_{2}$O$_{4}$ (0.968)        & CaFe$_{2}$O$_{4}$ (0.969)          \\
CaFe$_{4}$Al$_{8}$ (0.236)       & CaFe$_{5}$O$_{7}$ (0.358)         & CaIrO$_{3}$ (0.79)                         & CaMnGe$_{2}$O$_{6}$ (0.156)      & Co$_{2}$Mo$_{3}$O$_{8}$ (0.332)    \\
Co$_{2}$Mo$_{3}$O$_{8}$ (0.338)  & Co$_{3}$Sn$_{2}$S$_{2}$ (0.860)   & Co$_{3}$Sn$_{2}$S$_{2}$ (0.861)            & Co$_{4}$Nb$_{2}$O$_{9}$ (0.111)  & CoCO$_{3}$ (0.114)                 \\
CoSe$_{2}$O$_{5}$ (0.161)        & Cr$_{2}$CoAl (0.1073)             & Cr$_{2}$MoO$_{6}$ (0.1023)                 & Cr$_{2}$O$_{3}$ (0.110)          & Cr$_{2}$TeO$_{6}$ (0.143)          \\
Cr$_{2}$TeO$_{6}$ (0.76)         & Cr$_{2}$TeO$_{6}$ (0.959)         & Cr$_{2}$WO$_{6}$ (0.144)                   & Cr$_{2}$WO$_{6}$ (0.75)          & CrSbSe$_{3}$ (0.834)               \\
CsMnF$_{4}$ (0.327)              & CuFePO$_{5}$ (0.260)              & CuFeS$_{2}$ (0.802)                        & CuMnAs (0.222)                   & CuMnAs (0.881)                     \\
Fe$_{2}$Mo$_{3}$O$_{8}$ (0.331)  & Fe$_{2}$O$_{3}$ (0.299)           & Fe$_{2}$O$_{3}$ (0.300)                    & Fe$_{2}$O$_{3}$-alpha (0.65)           & Fe$_{2}$PO$_{5}$ (0.263)           \\
Fe$_{2}$SiO$_{4}$ (0.1071)       & Fe$_{2}$WO$_{6}$ (0.811)          & Fe$_{2}$WO$_{6}$ (0.813)                   & Fe$_{2}$WO$_{6}$ (0.814)         & Fe$_{3}$(PO$_{4}$)$_2$ (0.264)           \\
Fe$_{3}$(PO$_{4}$)$_2$(OH)$_2$ (0.392)       & Fe$_{3}$F$_{8}$(H$_{2}$O)$_2$ (0.582)   & Fe$_{4}$Nb$_{2}$O$_{9}$ (0.441)            & Fe$_{4}$Nb$_{2}$O$_{9}$ (0.443)  & FeBO$_{3}$ (0.112)                 \\
FeF$_{3}$ (0.335)                & FeF$_{3}$ (0.581)                 & FeOHSO$_{4}$ (0.760)                       & FeOOH (0.399)                    & FeSO$_{4}$F (0.128)                \\
GaFeO$_{3}$ (0.38)               & InCrO$_{3}$ (0.308)               & K$_{2}$ReI$_{6}$ (0.434)                   & K$_{2}$ReI$_{6}$ (0.553)         & KFeS$_{2}$ (0.633)                 \\
KMnF$_{3}$ (0.432)               & La$_{2}$LiRuO$_{6}$ (0.148)       & LaBaMn$_{2}$O$_{5}$ (0.735)                & LaCrO$_{3}$ (0.323)              & LaCrO$_{3}$ (0.417)                \\
LaMnO$_{3}$ (0.1)                & LaMnO$_{3}$ (0.642)               & Li$_{2}$Co(SO$_{4}$)$_2$ (0.121)                 & Li$_{2}$Mn(SO$_{4}$)$_2$ (0.122)       & Li$_{2}$Ni(SO$_{4}$)$_2$ (0.714)         \\
LiCrGe$_{2}$O$_{6}$ (0.217)      & LiCrGe$_{2}$O$_{6}$ (0.961)       & LiCrGe$_{2}$O$_{6}$ (0.962)                & LiCrGe$_{2}$O$_{6}$ (0.963)      & LiCrGe$_{2}$O$_{6}$ (0.964)        \\
LiFeP$_{2}$O$_{7}$ (0.83)        & LiFeSi$_{2}$O$_{6}$ (0.28)        & LiMn$_{6}$Sn$_{6}$ (0.699)                 & LiMnPO$_{4}$ (0.24)              & LiMnPO$_{4}$ (0.382)               \\
LuCrO$_{3}$ (0.1068)             & LuCrWO$_{6}$ (0.1082)             & LuFeO$_{3}$ (0.117)                        & LuVO$_{3}$ (0.984)               & Mn(N(CN$_{2}$))$_2$ (0.131)                \\
Mn$_{2}$FeReO$_{6}$ (0.541)      & Mn$_{2}$Mo$_{3}$O$_{8}$ (0.333)   & Mn$_{2}$Sb (0.855)                         & Mn$_{2}$SeO$_{3}$F$_{2}$ (0.755) & Mn$_{3}$AlN (0.275)                \\
Mn$_{3}$AlN (0.276)              & Mn$_{3}$As$_{2}$ (0.512)          & Mn$_{3}$As (0.279)                         & Mn$_{3}$As (0.280)               & Mn$_{3}$Ge (0.377)                 \\
Mn$_{3}$Ir (0.108)               & Mn$_{3}$IrGe (0.1006)             & Mn$_{3}$Pt (0.109)                         & Mn$_{3}$Sn (0.199)               & Mn$_{3}$Sn (0.200)                 \\
Mn$_{3}$Sn$_{2}$ (0.662)         & Mn$_{3}$Ti$_{2}$Te$_{6}$ (0.176)  & Mn$_{4}$N (0.274)                          & Mn$_{4}$Nb$_{2}$O$_{9}$ (0.507)  & Mn$_{4}$Ta$_{2}$O$_{9}$ (0.477)    \\
Mn$_{4}$Ta$_{2}$O$_{9}$ (0.526)  & Mn$_{5}$Ge$_{3}$ (0.286)          & MnCO$_{3}$ (0.115)                         & MnCoGe (0.445)                   & MnGeN$_{2}$ (0.1065)               \\
MnGeO$_{3}$ (0.312)              & MnLaMnSbO$_{6}$ (0.234)           & MnNb$_{2}$O$_{6}$ (0.815)                  & MnPS$_{3}$ (0.163)               & MnPSe$_{3}$ (0.180)                \\
MnPSe$_{3}$ (0.524)              & MnPd$_{2}$ (0.798)                & MnSiN$_{2}$ (0.1066)                       & MnTa$_{2}$O$_{6}$ (0.816)        & MnTiO$_{3}$ (0.19)                 \\
MnTiO$_{3}$ (0.50)               & Na$_{2}$BaCo(VO$_{4}$)$_2$ (0.266)      & NaCrGe$_{2}$O$_{6}$ (0.297)                & NaMnFeF$_{6}$ (0.310)            & NaOsO$_{3}$ (0.25)                 \\
NiCO$_{3}$ (0.113)               & NiCr$_{2}$O$_{4}$ (0.4)           & NiCr$_{2}$O$_{4}$ (0.895)                  & NiF$_{2}$ (0.36)                 & NiFePO$_{5}$ (0.261)               \\
RbFe$_{2}$F$_{6}$ (0.192)        & RbFeS$_{2}$ (0.636)               & ScCrO$_{3}$ (0.307)                        & ScMnO$_{3}$ (0.7)                & Sr$_{2}$CoOsO$_{6}$ (0.210)        \\
Sr$_{2}$CoTeO$_{6}$ (0.301)      & Sr$_{2}$CoTeO$_{6}$ (0.937)       & Sr$_{2}$Fe$_{2}$O$_{5}$ (0.1084)           & Sr$_{2}$LuRuO$_{6}$ (0.420)      & Sr$_{2}$MnGaO$_{5}$ (0.823)        \\
Sr$_{2}$MnTeO$_{6}$ (0.936)      & Sr$_{2}$NiTeO$_{6}$ (0.934)       & Sr$_{2}$ScOsO$_{6}$ (0.917)                & Sr$_{2}$YRuO$_{6}$ (0.795)       & Sr$_{4}$Fe$_{4}$O$_{11}$ (0.402)   \\
SrMnO$_{3}$ (0.1018)             & SrMnO$_{3}$ (0.1019)              & SrRuO$_{3}$ (0.732)                        & Tl$_{3}$Fe$_{2}$S$_{4}$ (0.801)  & TlCrO$_{3}$ (0.309)                \\
V$_{2}$WO$_{6}$ (0.966)          & Y$_{2}$Cu$_{2}$O$_{5}$ (0.241)    & YBaMn$_{2}$O$_{5}$ (0.739)                 & YCo$_{3}$ (0.859)                & YCrO$_{3}$ (0.586)                 \\
YCrO$_{3}$ (0.947)               & YNi$_{4}$Si (0.374)               & YRuO$_{3}$ (0.513)                         & YVO$_{3}$ (0.787)                & ZrMn$_{2}$Ge$_{4}$O$_{12}$ (0.315) \\ \hline
\end{tabular}
\label{165}
\end{table}

\clearpage
\subsection{First-Principles Total-Energy Calculations}
 
For these 253 materials whose magnetic structures are included in the initial set of magnetic configurations from our irrep basis-vector strategy,
the first-principles total-energy calculations were performed, using the Vienna \textit{ab initio} Simulation Package (VASP)~\cite{vasp1,vasp2}. The calculations employ a spin-polarized GGA + SOC + $U$ approach. The on-site Coulomb interaction parameters $U$ and $J$ are chosen as the averaged values recommended for transition-metal elements based on the linear-response scheme~\cite{Uvalue}. We further verify that reasonable variations of $U$ within physically relevant ranges do not alter the predicted magnetic structure.

Our DFT calculations successfully reproduce 198 out of 253 magnetic structures, yielding a total accuracy of 78.2\%, as summarized in Table~\ref{DFT-statistics}.

%%%%%%%%    DFT计算结果表格
\begin{table}[!h]
\caption{Table of first-principles benchmark results based on well-selected input structures. Among the 253 materials subjected to first-principles calculations, the magnetic structure obtained from DFT agree with experimental results in 198 cases, whereas deviations from experimental results are found in the remaining 55 cases, which may arise from the intrinsic limitations of DFT. Material names are followed by their corresponding labels (in parentheses) from the MAGNDATA database\cite{gallego2016magndata}.}
\begin{tabular}{c|ccccc}
\hline
                                                                                                                                                                         & \multicolumn{5}{c}{Materials}                                                                                                                                                                                \\ \hline
\multirow{40}{*}{\begin{tabular}[c]{@{}c@{}}Our framework \\ successfully \\ predict the \\ experimental \\magnetic \\  ground states \\ for these \\ materials\end{tabular}} & AlFe$_{2}$B$_{2}$ (0.414)                & Ba$_{2}$CoGe$_{2}$O$_{7}$ (0.56)         & Ba$_{2}$MnSi$_{2}$O$_{7}$ (0.229)       & Ba$_{3}$NiRu$_{2}$O$_{9}$ (0.748)          & BaCr$_{2}$As$_{2}$ (0.365)      \\
                                                                                                                                                                         & BaCrF$_{5}$ (0.303)                      & BaCuF$_{4}$ (0.191)                      & BaFe$_{2}$S$_{2}$O (0.987)              & BaMn$_{2}$As$_{2}$ (0.18)                  & BaMn$_{2}$Bi$_{2}$ (0.89)       \\
                                                                                                                                                                         & BaMn$_{2}$Ge$_{2}$ (0.605)               & BaMn$_{2}$Ge$_{2}$ (0.606)               & BaMn$_{2}$P$_{2}$ (0.464)               & BaMn$_{2}$Sb$_{2}$ (0.470)                 & BaMnSb$_{2}$ (0.611)            \\
                                                                                                                                                                         & BaNi$_{2}$P$_{2}$O$_{8}$ (0.215)         & Bi$_{2}$CuO$_{4}$ (0.348)                & Bi$_{2}$CuO$_{4}$ (0.694)               & Bi$_{2}$CuO$_{4}$ (0.695)                  & BiCrO$_{3}$ (0.138)             \\
                                                                                                                                                                         & Ca$_{2}$Fe$_{2}$O$_{5}$ (0.1080)         & Ca$_{2}$FeOsO$_{6}$ (0.682)              & Ca$_{2}$NiOsO$_{6}$ (0.796)             & CaCu$_{3}$Fe$_{2}$Sb$_{2}$O$_{12}$ (0.672) & CaFe$_{5}$O$_{7}$ (0.358)       \\
                                                                                                                                                                         & CaIrO$_{3}$ (0.79)                       & CaMn$_{2}$Ge$_{2}$ (0.603)               & CaMn$_{2}$Ge$_{2}$ (0.604)              & CaMn$_{2}$Sb$_{2}$ (0.92)                  & CaMnBi$_{2}$ (0.72)             \\
                                                                                                                                                                         & CaMnGe$_{2}$O$_{6}$ (0.156)              & CaMnSi (0.599)                           & CaMnSi (0.600)                          & Co$_{2}$Mo$_{3}$O$_{8}$ (0.332)            & Co$_{2}$Mo$_{3}$O$_{8}$ (0.338) \\
                                                                                                                                                                         & Co$_{3}$Sn$_{2}$S$_{2}$ (0.860)          & Co$_{3}$Sn$_{2}$S$_{2}$ (0.861)          & Co$_{4}$Nb$_{2}$O$_{9}$ (0.111)         & CoCO$_{3}$ (0.114)                         & CoF$_{2}$ (0.178)               \\
                                                                                                                                                                         & CoF$_{3}$ (0.334)                        & CoSe$_{2}$O$_{5}$ (0.161)                & CoTa$_{4}$Se$_{8}$ (0.1036)             & Cr$_{2}$O$_{3}$ (0.110)                    & Cr$_{2}$O$_{3}$ (0.59)          \\
                                                                                                                                                                         & Cr$_{2}$TeO$_{6}$ (0.143)                & Cr$_{2}$TeO$_{6}$ (0.76)                 & Cr$_{2}$TeO$_{6}$ (0.959)               & Cr$_{2}$WO$_{6}$ (0.144)                   & Cr$_{2}$WO$_{6}$ (0.75)         \\
                                                                                                                                                                         & CrSb (0.528)                             & CrSbSe$_{3}$ (0.834)                     & CuFePO$_{5}$ (0.260)                    & CuFeS$_{2}$ (0.802)                        & CuMnAs (0.222)                  \\
                                                                                                                                                                         & CuMnAs (0.881)                           & Fe$_{2}$Mo$_{3}$O$_{8}$ (0.331)          & Fe$_{2}$O$_{3}$-alpha (0.65)                  & Fe$_{2}$PO$_{5}$ (0.263)                   & Fe$_{2}$SiO$_{4}$ (0.1071)      \\
                                                                                                                                                                         & Fe$_{2}$TeO$_{6}$ (0.142)                & Fe$_{2}$TeO$_{6}$ (0.960)                & Fe$_{2}$WO$_{6}$ (0.814)                & Fe$_{3}$(PO$_{4}$)$_2$(OH)$_2$ (0.392)                 & Fe$_{3}$F$_{8}$(H$_{2}$O)$_2$ (0.582) \\
                                                                                                                                                                         & FeBO$_{3}$ (0.112)                       & FeCO$_{3}$ (0.116)                       & FeF$_{3}$ (0.335)                       & FeF$_{3}$ (0.581)                          & FeOHSO$_{4}$ (0.760)            \\
                                                                                                                                                                         & FeOOH (0.399)                            & FeSO$_{4}$F (0.128)                      & GaFeO$_{3}$ (0.38)                      & InCrO$_{3}$ (0.308)                        & K$_{2}$ReI$_{6}$ (0.434)        \\
                                                                                                                                                                         & K$_{2}$ReI$_{6}$ (0.553)                 & KFeS$_{2}$ (0.633)                       & KFeSe$_{2}$ (0.637)                     & KMnBi (0.618)                              & KMnF$_{3}$ (0.432)              \\
                                                                                                                                                                         & KMnF$_{3}$ (0.433)                       & KMnSb (0.617)                            & KOsO$_{4}$ (0.284)                      & KRuO$_{4}$ (0.285)                         & La$_{2}$LiRuO$_{6}$ (0.148)     \\
                                                                                                                                                                         & La$_{2}$O$_{3}$Mn$_{2}$Se$_{2}$ (0.1092) & La$_{2}$O$_{3}$Mn$_{2}$Se$_{2}$ (0.1093) & LaBaMn$_{2}$O$_{6}$ (0.737)             & LaBaMn$_{2}$O$_{6}$ (0.738)                & LaCrO$_{3}$ (0.323)             \\
                                                                                                                                                                         & LaCrO$_{3}$ (0.416)                      & LaCrO$_{3}$ (0.417)                      & LaMn$_{2}$Si$_{2}$ (0.472)              & LaMn$_{2}$Si$_{2}$ (0.498)                 & LaMnAsO (0.619)                 \\
                                                                                                                                                                         & LaMnAsO (0.624)                          & LaMnSbO (0.667)                          & Li$_{2}$Co(SO$_{4}$)$_2$ (0.121)              & Li$_{2}$Mn(SO$_{4}$)$_2$ (0.122)                 & Li$_{2}$Ni(SO$_{4}$)$_2$ (0.714)      \\
                                                                                                                                                                         & LiCoPO$_{4}$ (0.193)                     & LiCoPO$_{4}$ (0.383)                     & LiFe$_{2}$F$_{6}$ (0.501)               & LiFeP$_{2}$O$_{7}$ (0.83)                  & LiFePO$_{4}$ (0.95)             \\
                                                                                                                                                                         & LiMn$_{6}$Sn$_{6}$ (0.699)               & LiMnPO$_{4}$ (0.24)                      & LiMnPO$_{4}$ (0.382)                    & LuCrO$_{3}$ (0.1068)                       & LuCrWO$_{6}$ (0.1082)           \\
                                                                                                                                                                         & Mn(N(CN$_{2}$))$_2$ (0.131)                      & Mn$_{2}$Au (0.1081)                      & Mn$_{2}$Au (0.639)                      & Mn$_{2}$Au (0.640)                         & Mn$_{2}$FeReO$_{6}$ (0.541)     \\
                                                                                                                                                                         & Mn$_{2}$Sb (0.855)                       & Mn$_{3}$As$_{2}$ (0.512)                 & Mn$_{3}$GaN (0.177)                     & Mn$_{3}$Ge (0.377)                         & Mn$_{3}$Ir (0.108)              \\
                                                                                                                                                                         & Mn$_{3}$Sn (0.199)                       & Mn$_{3}$Sn (0.200)                       & Mn$_{3}$Ti$_{2}$Te$_{6}$ (0.176)        & Mn$_{3}$ZnN (0.273)                        & Mn$_{4}$N (0.274)               \\
                                                                                                                                                                         & Mn$_{4}$Nb$_{2}$O$_{9}$ (0.507)          & Mn$_{4}$Ta$_{2}$O$_{9}$ (0.477)          & Mn$_{4}$Ta$_{2}$O$_{9}$ (0.526)         & Mn$_{5}$Ge$_{3}$ (0.286)                   & MnCO$_{3}$ (0.115)              \\
                                                                                                                                                                         & MnF$_{2}$ (0.15)                         & MnGeN$_{2}$ (0.1065)                     & MnGeO$_{3}$ (0.125)                     & MnGeO$_{3}$ (0.312)                        & MnLaMnSbO$_{6}$ (0.234)         \\
                                                                                                                                                                         & MnNb$_{2}$O$_{6}$ (0.815)                & MnNb$_{4}$S$_{8}$ (0.709)                & MnPS$_{3}$ (0.163)                      & MnPSe$_{3}$ (0.180)                        & MnPSe$_{3}$ (0.524)             \\
                                                                                                                                                                         & MnPd$_{2}$ (0.798)                       & MnSiN$_{2}$ (0.1066)                     & MnTa$_{2}$O$_{6}$ (0.816)               & MnTa$_{4}$S$_{8}$ (0.711)                  & MnTe (0.800)                    \\
                                                                                                                                                                         & MnTe$_{2}$ (0.20)                        & MnTiO$_{3}$ (0.19)                       & MnTiO$_{3}$ (0.50)                      & Na$_{2}$BaCo(VO$_{4}$)$_2$(0.266)               & NaCrGe$_{2}$O$_{6}$ (0.297)     \\
                                                                                                                                                                         & NaMnAs (0.629)                           & NaMnAs (0.630)                           & NaMnBi (0.634)                          & NaMnBi (0.635)                             & NaMnFeF$_{6}$ (0.310)           \\
                                                                                                                                                                         & NaMnP (0.626)                            & NaMnP (0.627)                            & NaMnP (0.628)                           & NaMnSb (0.631)                             & NaMnSb (0.632)                  \\
                                                                                                                                                                         & NaOsO$_{3}$ (0.25)                       & NiCO$_{3}$ (0.113)                       & NiCr$_{2}$O$_{4}$ (0.4)                 & NiCrO$_{4}$ (0.896)                        & NiF$_{2}$ (0.36)                \\
                                                                                                                                                                         & NiFePO$_{5}$ (0.261)                     & NiS$_{2}$ (0.150)                        & PbNiO$_{3}$ (0.21)                      & RbFe$_{2}$F$_{6}$ (0.192)                  & RbFeS$_{2}$ (0.636)             \\
                                                                                                                                                                         & RbFeSe$_{2}$ (0.638)                     & RuO$_{2}$ (0.607)                        & ScCrO$_{3}$ (0.307)                     & Sr$_{2}$CoTeO$_{6}$ (0.301)                & Sr$_{2}$CoTeO$_{6}$ (0.937)     \\
                                                                                                                                                                         & Sr$_{2}$LuRuO$_{6}$ (0.420)              & Sr$_{2}$MnGaO$_{5}$ (0.823)              & Sr$_{2}$MnTeO$_{6}$ (0.936)             & Sr$_{2}$NiTeO$_{6}$ (0.934)                & Sr$_{2}$ScOsO$_{6}$ (0.917)     \\
                                                                                                                                                                         & Sr$_{2}$YRuO$_{6}$ (0.795)               & Sr$_{4}$Fe$_{4}$O$_{11}$ (0.401)         & Sr$_{4}$Fe$_{4}$O$_{11}$ (0.402)        & SrCr$_{2}$As$_{2}$ (0.364)                 & SrMn$_{2}$As$_{2}$ (0.482)      \\
                                                                                                                                                                         & SrMnBi$_{2}$ (0.73)                      & SrMnO$_{3}$ (0.1018)                     & SrMnO$_{3}$ (0.1019)                    & SrRuO$_{3}$ (0.732)                        & TlCrO$_{3}$ (0.309)             \\
                                                                                                                                                                         & V$_{2}$WO$_{6}$ (0.966)                  & VNb$_{3}$S$_{6}$ (0.712)                 & Y$_{2}$Cu$_{2}$O$_{5}$ (0.241)          & YCrO$_{3}$ (0.586)                         & YCrO$_{3}$ (0.947)              \\
                                                                                                                                                                         & YVO$_{3}$ (0.787)                        & ZrMn$_{2}$Ge$_{4}$O$_{12}$ (0.315)       & [Na(OH)$_{2}$]$_{3}$Mn(NCS)$_{3}$ (0.1078)                &                                            &                                 \\ \hline
\multirow{11}{*}{\begin{tabular}[c]{@{}c@{}}Our framework \\ failed to \\ identify the \\ experimental\\ magnetic \\ ground state \\ for these \\ materials\end{tabular}}        & Ba$_{2}$Mn$_{3}$Sb$_{2}$O$_{2}$ (0.471)  & Ca$_{2}$MnGaO$_{5}$ (0.825)              & CaFe$_{2}$O$_{4}$ (0.968)               & CaFe$_{2}$O$_{4}$ (0.969)                  & CaFe$_{4}$Al$_{8}$ (0.236)      \\
                                                                                                                                                                         & Cr$_{2}$CoAl (0.1073)                    & Cr$_{2}$MoO$_{6}$ (0.1023)               & CrNb$_{4}$S$_{8}$ (0.708)               & CsMnF$_{4}$ (0.327)                        & Fe$_{2}$O$_{3}$ (0.299)         \\
                                                                                                                                                                         & Fe$_{2}$O$_{3}$ (0.300)                  & Fe$_{2}$WO$_{6}$ (0.811)                 & Fe$_{2}$WO$_{6}$ (0.813)                & Fe$_{3}$(PO$_{4}$)$_2$ (0.264)                   & Fe$_{4}$Nb$_{2}$O$_{9}$ (0.441) \\
                                                                                                                                                                         & Fe$_{4}$Nb$_{2}$O$_{9}$ (0.443)          & La$_{2}$O$_{3}$Mn$_{2}$Se$_{2}$ (0.1091) & LaBaMn$_{2}$O$_{5}$ (0.735)             & LaMnO$_{3}$ (0.1)                          & LaMnO$_{3}$ (0.642)             \\
                                                                                                                                                                         & LaMnSi$_{2}$ (0.778)                     & LaMnSi$_{2}$ (0.779)                     & LaMnSi$_{2}$ (0.780)                    & LiCrGe$_{2}$O$_{6}$ (0.217)                & LiCrGe$_{2}$O$_{6}$ (0.961)     \\
                                                                                                                                                                         & LiCrGe$_{2}$O$_{6}$ (0.962)              & LiCrGe$_{2}$O$_{6}$ (0.963)              & LiCrGe$_{2}$O$_{6}$ (0.964)             & LiFeSi$_{2}$O$_{6}$ (0.28)                 & LuFeO$_{3}$ (0.117)             \\
                                                                                                                                                                         & LuVO$_{3}$ (0.984)                       & MgMnO$_{3}$ (0.277)                      & Mn$_{2}$Mo$_{3}$O$_{8}$ (0.333)         & Mn$_{2}$SeO$_{3}$F$_{2}$ (0.755)           & Mn$_{3}$AlN (0.275)             \\
                                                                                                                                                                         & Mn$_{3}$AlN (0.276)                      & Mn$_{3}$As (0.279)                       & Mn$_{3}$As (0.280)                      & Mn$_{3}$IrGe (0.1006)                      & Mn$_{3}$Pt (0.109)              \\
                                                                                                                                                                         & Mn$_{3}$Sn$_{2}$ (0.662)                 & MnCoGe (0.445)                           & MnPtGa (0.395)                          & NiCr$_{2}$O$_{4}$ (0.895)                  & ScMnO$_{3}$ (0.7)               \\
                                                                                                                                                                         & Sr$_{2}$CoOsO$_{6}$ (0.210)              & Sr$_{2}$Fe$_{2}$O$_{5}$ (0.1084)         & Sr$_{2}$Mn$_{3}$As$_{2}$O$_{2}$ (0.212) & SrMnSb$_{2}$ (0.767)                       & Tl$_{3}$Fe$_{2}$S$_{4}$ (0.801) \\
                                                                                                                                                                         & YBaMn$_{2}$O$_{5}$ (0.739)               & YCo$_{3}$ (0.859)                        & YMnO$_{3}$ (0.6)                        & YNi$_{4}$Si (0.374)                        & YRuO$_{3}$ (0.513)              \\ \hline
\end{tabular}
\label{DFT-statistics}
\end{table}

\clearpage 
\section{Magnetic Materials Database}

\subsection{Statistics of magnetic materials}
We applied our framework to the Inorganic Crystal Structure Database (ICSD) \cite{ICSD}. 
After excluding entries with fractional site occupancies, we focus on the materials with fewer than 30 atoms in the primitive unit cell and 
exclude lanthanoids and actinoids due to the challenges in accurately described within standard density functional theory \cite{kotliar2006electronic}.
To limit the computational cost at this stage, we consider the magnetic structures with a propagation vector $\mathbf{q}=0$, and performed systematic high-throughput first-principles calculations to determine the magnetic structure of 8,422 transition-metal compounds. Within this well-defined scope, our workflow identified 5,516 materials as non-magnetic. The remaining 2,906 magnetic materials were compiled into a magnetic structure database. 
Calculations for materials exceeding 30 atoms per unit cell are currently in progress. The magnetic structure, electronic band structures, and associated information of topological magnetic materials is available at \url{https://magdatabase.nju.edu.cn}, which is continuously updated. The corresponding magCIF files are also available for download on the website for user access. 

This database captures a broad diversity of magnetic configurations.
From the viewpoint of magnetic classification, 
1,449 materials exhibit ferromagnetic (FM) ordering, and 338 materials are classified as ferrimagnetic (FiM).
1,119 compounds exhibit
antiferromagnetic (AFM) order with vanishing net magnetization, including
392 altermagnets. Ferromagnetic materials, collinear ferrimagnetic materials, non-collinear ferrimagnetic materials, collinear antiferromagnetic materials, non-collinear antiferromagnetic materials, and altermagnetic materials are in Table \ref{FM}-\ref{FMfinal}, \ref{ColFiM}-\ref{ColFiMfinal}, \ref{NoCFiM}-\ref{NoCFiMfinal}, \ref{ColAFM}-\ref{ColAFMfinal}, \ref{NoCAFM}-\ref{NoCAFMfinal}, \ref{Alter}-\ref{Alterfinal}, respectively.

\begin{figure}[htbp]
    \centering
    \includegraphics[width=0.6\linewidth]{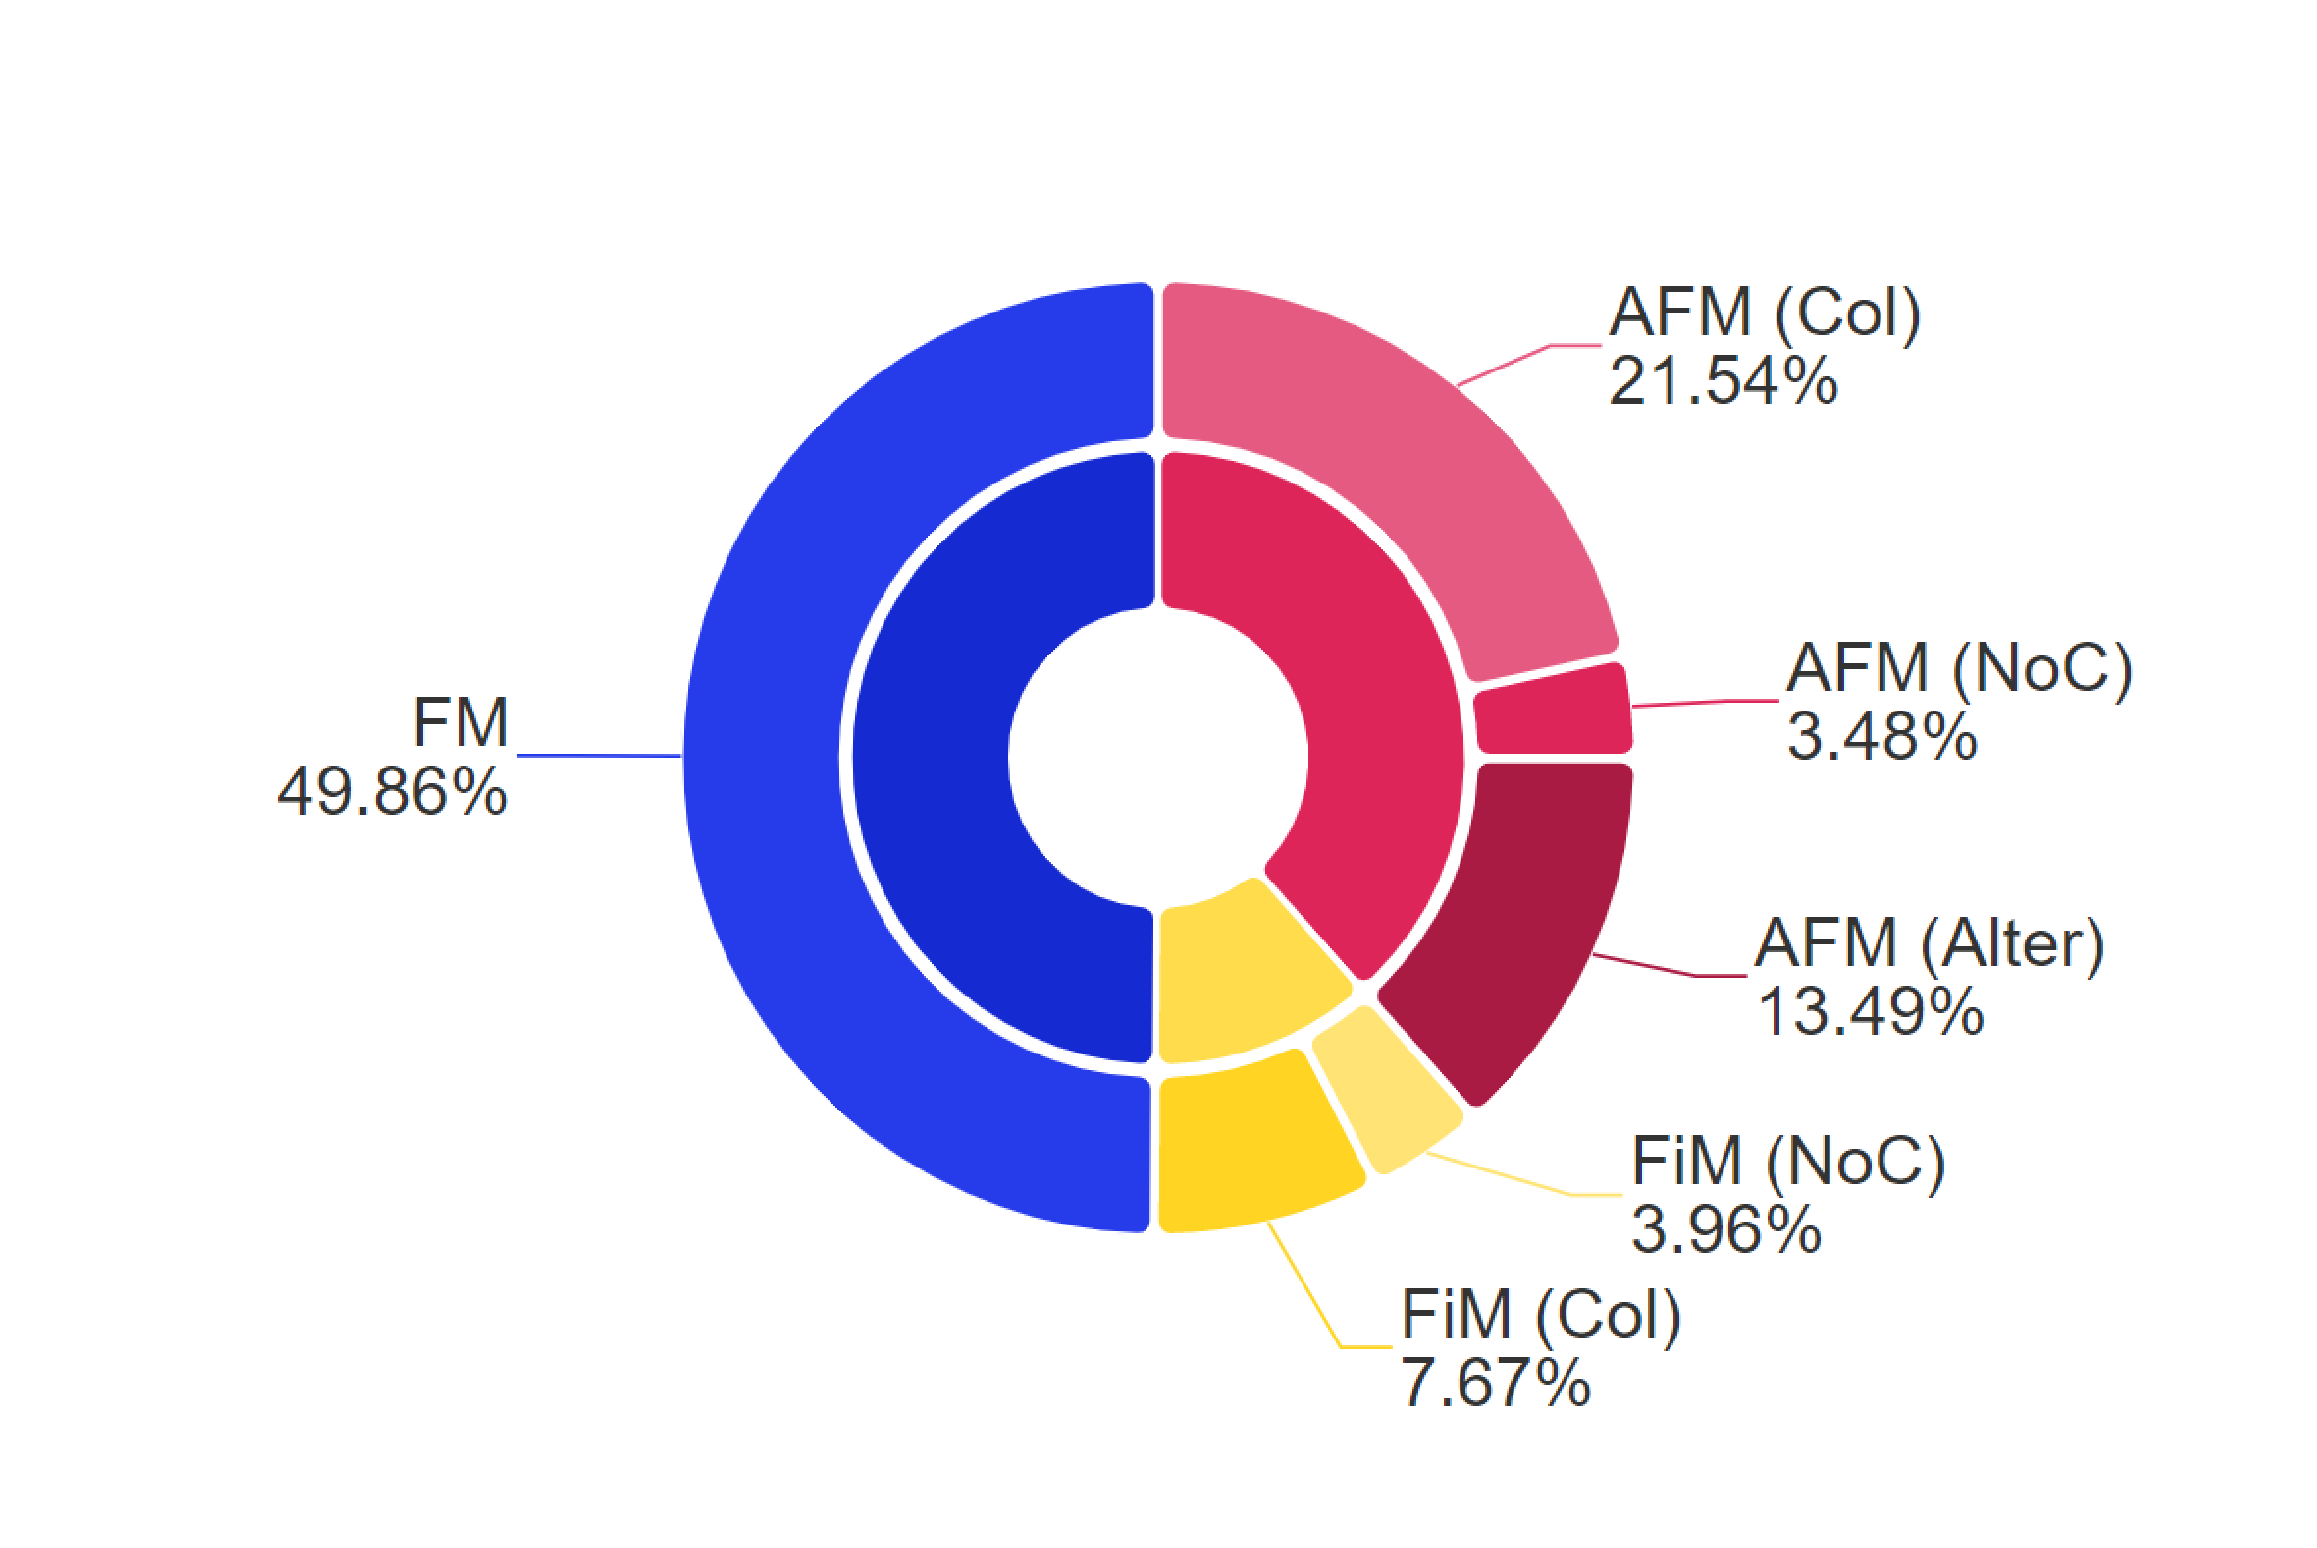}
\caption{\textbf{Magnetic and topological classification of our magnetic structure database.}
(a) Statistics of magnetic ground-state classification.Among the 2,906 identified magnetic materials, 49.86\% exhibit ferromagnetic (FM) ordering, 11.63\% are ferrimagnetic (FiM), and the remaining 38.51\% are antiferromagnetic (AFM).The FiM materials are further classified into 7.67\% collinear (Col) and 3.96\% noncollinear (NoC) states according to the relative orientation of magnetic moments.Within the AFM materials, 21.54\% exhibit collinear (Col) order, 3.48\% exhibit noncollinear (NoC) order, and 13.49\% are classified as altermagnets (Alter).}
    \label{MCStatistics_SM}
\end{figure}
\newpage

\subsection{Ferromagnetic materials}
The relevant information for the ferromagnetic materials is summarized in Table \ref{FM}-\ref{FMfinal}, including their chemical formula, space group, magnetic space group, band gap and corresponding irreducible representations of crystallographic space group.
\begin{table*}[!h]
\centering
\caption{Tabulated information on \textbf{ferromagnetic} materials, including the chemical formula, 
space group, magnetic space group, band gap and corresponding irreducible representations of crystallographic space group.}
\renewcommand{\arraystretch}{0.8}
% [inline block 0: 23 envs, 114899 chars -> data_tex | \begin{tabular}{cccccc} \hline...]

\label{FMfinal}
\end{table*}

\newpage
\subsection{Collinear ferrimagnetic materials}
The relevant information for ferrimagnetic materials is summarized in Table \ref{ColFiM}-\ref{ColFiMfinal}, including their chemical formula, space group, magnetic space group, band gap and corresponding irreducible representations of crystallographic space group.
\begin{table*}[!h]
\centering
\caption{Tabulated information on \textbf{collinear ferrimagnetic} materials, including the chemical formula, 
space group, magnetic space group, band gap and corresponding irreducible representations of crystallographic space group.}
\renewcommand{\arraystretch}{0.8}
\begin{tabular}{cccccc}
\hline
ICSD number & Chemical formula & SG NUM & BNS & Band Gap (eV)  & Irrep \\
\hline
icsd\_010509 & Al$_{11}$Mn$_{4}$ & 2 & 2.4 & 0.00 & $\Gamma_{1}^{+}$ \\
icsd\_063057 & As$_{2}$Cu$_{3}$O$_{8}$ & 2 & 2.4 & 2.05 & $\Gamma_{1}^{+}$ \\
icsd\_167202 & CoFLiO$_{4}$S & 2 & 2.4 & 3.41 & $\Gamma_{1}^{+}$ \\
icsd\_050507 & CrF$_{6}$Mo & 2 & 2.4 & 0.62 & $\Gamma_{1}^{+}$ \\
icsd\_193472 & Cu$_{3}$Nb$_{2}$O$_{8}$ & 2 & 2.4 & 0.20 & $\Gamma_{1}^{+}$ \\
icsd\_001143 & Cu$_{3}$O$_{8}$P$_{2}$ & 2 & 2.4 & 2.07 & $\Gamma_{1}^{+}$ \\
icsd\_050506 & CuF$_{6}$Mo & 2 & 2.4 & 0.70 & $\Gamma_{1}^{+}$ \\
icsd\_079695 & H$_{2}$As$_{2}$CuFe$_{2}$O$_{10}$ & 2 & 1.1 & 2.55 & $\Gamma_{1}^{-}$ \\
icsd\_192247 & CoY$_{3}$ & 4 & 4.9 & 0.00 & $\Gamma_{2}$ \\
icsd\_240499 & BrOTi & 11 & 11.54 & 0.00 & $\Gamma_{2}^{+}$ \\
icsd\_051677 & H$_{3}$ClCu$_{2}$O$_{3}$ & 11 & 11.54 & 1.70 & $\Gamma_{2}^{+}$ \\
icsd\_624485 & Co$_{2}$NiSe$_{4}$ & 12 & 12.62 & 0.00 & $\Gamma_{2}^{+}$ \\
icsd\_622499 & CoCr$_{2}$S$_{4}$ & 12 & 12.62 & 0.00 & $\Gamma_{2}^{+}$ \\
icsd\_601038 & CoCr$_{2}$Se$_{4}$ & 12 & 12.62 & 0.00 & $\Gamma_{2}^{+}$ \\
icsd\_622979 & CoFe$_{2}$Se$_{4}$ & 12 & 12.62 & 0.00 & $\Gamma_{2}^{+}$ \\
icsd\_026173 & CoMo$_{2}$S$_{4}$ & 12 & 12.58 & 0.00 & $\Gamma_{1}^{+}$ \\
icsd\_624874 & CoS$_{4}$Ti$_{2}$ & 12 & 12.62 & 0.00 & $\Gamma_{2}^{+}$ \\
icsd\_624884 & CoS$_{4}$V$_{2}$ & 12 & 12.58 & 0.00 & $\Gamma_{1}^{+}$ \\
icsd\_625002 & CoSe$_{4}$Ti$_{2}$ & 12 & 12.62 & 0.00 & $\Gamma_{2}^{+}$ \\
icsd\_625012 & CoSe$_{4}$V$_{2}$ & 12 & 12.58 & 0.00 & $\Gamma_{1}^{+}$ \\
icsd\_625931 & Cr$_{2}$FeS$_{4}$ & 12 & 12.62 & 0.27 & $\Gamma_{2}^{+}$ \\
icsd\_043042 & Cr$_{2}$FeSe$_{4}$ & 12 & 12.62 & 0.00 & $\Gamma_{2}^{+}$ \\
icsd\_016884 & Cr$_{2}$NiS$_{4}$ & 12 & 12.62 & 0.06 & $\Gamma_{2}^{+}$ \\
icsd\_626655 & CrS$_{4}$V$_{2}$ & 12 & 12.58 & 0.00 & $\Gamma_{1}^{+}$ \\
icsd\_633332 & Fe$_{0.5}$S$_{2}$Ti & 12 & 12.62 & 0.00 & $\Gamma_{2}^{+}$ \\
icsd\_015043 & Fe$_{3}$Se$_{4}$ & 12 & 12.62 & 0.00 & $\Gamma_{2}^{+}$ \\
icsd\_632972 & FeNi$_{2}$Se$_{4}$ & 12 & 12.62 & 0.00 & $\Gamma_{2}^{+}$ \\
icsd\_603354 & FeRh$_{2}$Se$_{4}$ & 12 & 12.58 & 0.00 & $\Gamma_{1}^{+}$ \\
icsd\_042563 & FeS$_{4}$Ti$_{2}$ & 12 & 12.62 & 0.00 & $\Gamma_{2}^{+}$ \\
icsd\_035634 & FeS$_{4}$V$_{2}$ & 12 & 12.62 & 0.06 & $\Gamma_{2}^{+}$ \\
icsd\_633504 & FeSe$_{4}$Ti$_{2}$ & 12 & 12.62 & 0.61 & $\Gamma_{2}^{+}$ \\
icsd\_193869 & Ni$_{0.5}$Se$_{2}$Ti & 12 & 12.62 & 0.00 & $\Gamma_{2}^{+}$ \\
icsd\_042558 & Ni$_{3}$Se$_{4}$ & 12 & 12.62 & 0.00 & $\Gamma_{2}^{+}$ \\
icsd\_646388 & NiS$_{4}$Ti$_{2}$ & 12 & 12.62 & 0.00 & $\Gamma_{2}^{+}$ \\
icsd\_035140 & NiS$_{4}$V$_{2}$ & 12 & 12.62 & 0.00 & $\Gamma_{2}^{+}$ \\
icsd\_646544 & NiSe$_{4}$Ti$_{2}$ & 12 & 12.62 & 0.00 & $\Gamma_{2}^{+}$ \\
icsd\_023970 & NiSe$_{4}$V$_{2}$ & 12 & 12.62 & 0.00 & $\Gamma_{2}^{+}$ \\
icsd\_024566 & S$_{4}$V$_{3}$ & 12 & 12.62 & 0.00 & $\Gamma_{2}^{+}$ \\
icsd\_601347 & Se$_{4}$Ti$_{3}$ & 12 & 12.58 & 0.00 & $\Gamma_{1}^{+}$ \\
icsd\_043412 & Te$_{4}$Ti$_{3}$ & 12 & 12.58 & 0.00 & $\Gamma_{1}^{+}$ \\
icsd\_041858 & AsCoS & 14 & 14.75 & 0.00 & $\Gamma_{1}^{+}$ \\
icsd\_239671 & Ca$_{2}$CrO$_{6}$Os & 14 & 14.79 & 0.00 & $\Gamma_{2}^{+}$ \\
icsd\_089955 & Ca$_{2}$FeMoO$_{6}$ & 14 & 14.75 & 0.67 & $\Gamma_{1}^{+}$ \\
icsd\_238148 & Ca$_{2}$FeO$_{6}$Os & 14 & 14.75 & 0.72 & $\Gamma_{1}^{+}$ \\
icsd\_181147 & FeMn$_{2}$O$_{6}$Sb & 14 & 14.79 & 1.53 & $\Gamma_{2}^{+}$ \\
icsd\_096120 & La$_{2}$NiO$_{6}$Ru & 14 & 14.79 & 0.76 & $\Gamma_{2}^{+}$ \\
icsd\_252567 & Mn$_{3}$O$_{6}$Re & 14 & 14.79 & 0.00 & $\Gamma_{2}^{+}$ \\
icsd\_602022 & HFeTi & 17 & 51.296 & 0.00 & $\Gamma_{3}$ \\
icsd\_632217 & H$_{2}$FeTi & 26 & 26.69 & 0.00 & $\Gamma_{3}$ \\
icsd\_627741 & Cu$_{2}$GeMnSe$_{4}$ & 31 & 31.127 & 1.01 & $\Gamma_{2}$ \\
icsd\_020082 & AlB$_{4}$Cr$_{3}$ & 47 & 47.252 & 0.00 & $\Gamma_{4}^{+}$ \\
icsd\_171434 & BaCo$_{2}$O$_{5}$Y & 51 & 51.296 & 0.48 & $\Gamma_{4}^{+}$ \\
icsd\_033996 & CoCu$_{2}$O$_{3}$ & 59 & 59.410 & 0.68 & $\Gamma_{4}^{+}$ \\
icsd\_610884 & AsMnNi & 62 & 62.446 & 0.00 & $\Gamma_{2}^{+}$ \\
icsd\_670822 & CCo$_{2}$Fe & 62 & 62.446 & 0.00 & $\Gamma_{2}^{+}$ \\
icsd\_670825 & CCrFe$_{2}$ & 62 & 62.441 & 0.00 & $\Gamma_{1}^{+}$ \\
icsd\_167127 & CFe$_{2}$Ni & 62 & 62.446 & 0.00 & $\Gamma_{2}^{+}$ \\
icsd\_025726 & Co$_{2}$P & 62 & 62.447 & 0.00 & $\Gamma_{3}^{+}$ \\
icsd\_016483 & CoMnP & 62 & 62.448 & 0.00 & $\Gamma_{4}^{+}$ \\
icsd\_005432 & CoMnSi & 62 & 62.446 & 0.00 & $\Gamma_{2}^{+}$ \\
icsd\_002421 & CoMoP & 62 & 62.446 & 0.00 & $\Gamma_{2}^{+}$ \\
icsd\_624646 & CoPTi & 62 & 62.446 & 0.00 & $\Gamma_{2}^{+}$ \\
icsd\_041918 & GeMnNi & 62 & 62.447 & 0.00 & $\Gamma_{3}^{+}$ \\
icsd\_076084 & MnNiSi & 62 & 62.448 & 0.00 & $\Gamma_{4}^{+}$ \\
icsd\_187466 & O$_{3}$Ti$_{2}$ & 62 & 62.446 & 0.30 & $\Gamma_{2}^{+}$ \\
\hline
\end{tabular}
\label{ColFiM}
\end{table*}
\clearpage

\begin{table*}[htbp]
\centering
\caption{Tabulated information on \textbf{collinear ferrimagnetic} materials, including the chemical formula, 
space group, magnetic space group, band gap and corresponding irreducible representations of crystallographic space group.}
\renewcommand{\arraystretch}{0.8}
\begin{tabular}{cccccc}
\hline
ICSD number & Chemical formula & SG NUM & BNS & Band Gap (eV)  & Irrep \\
\hline
icsd\_044188 & B$_{3}$CoV & 63 & 63.463 & 0.00 & $\Gamma_{3}^{+}$ \\
icsd\_042629 & CCr$_{3}$Ge & 63 & 63.464 & 0.00 & $\Gamma_{4}^{+}$ \\
icsd\_189439 & Fe$_{2}$O$_{3}$ & 63 & 63.464 & 0.59 & $\Gamma_{4}^{+}$ \\
icsd\_065881 & BaCu$_{3}$O$_{4}$ & 65 & 65.485 & 1.22 & $\Gamma_{2}^{+}$ \\
icsd\_050089 & Cu$_{6}$O$_{10}$Sr$_{4}$ & 65 & 65.485 & 0.00 & $\Gamma_{2}^{+}$ \\
icsd\_044293 & B$_{4}$Fe$_{2}$Mo & 71 & 71.536 & 0.00 & $\Gamma_{2}^{+}$ \\
icsd\_614748 & B$_{4}$Mn$_{2}$Mo & 71 & 71.536 & 0.00 & $\Gamma_{2}^{+}$ \\
icsd\_670346 & CaMnO$_{3}$ & 71 & 71.536 & 0.13 & $\Gamma_{3}^{+}$ \\
icsd\_416904 & Cu$_{3}$O$_{5}$Sr$_{2}$ & 71 & 71.536 & 0.37 & $\Gamma_{3}^{+}$ \\
icsd\_150701 & FeMoO$_{6}$Sr$_{2}$ & 87 & 12.62 & 0.00 & $\Gamma_{3}^+\Gamma_{4}^+$ \\
icsd\_052332 & Sb$_{4}$V$_{5}$ & 87 & 12.62 & 0.00 & $\Gamma_{3}^+\Gamma_{4}^+$ \\
icsd\_042881 & Te$_{4}$V$_{5}$ & 87 & 12.62 & 0.00 & $\Gamma_{3}^+\Gamma_{4}^+$ \\
icsd\_067978 & BaCuFeO$_{5}$Y & 99 & 25.59 & 0.00 & $\Gamma_{5}$ \\
icsd\_167196 & FeSe$_{0.875}$ & 99 & 25.59 & 0.00 & $\Gamma_{5}$ \\
icsd\_023779 & CrNNb & 100 & 99.167 & 0.00 & $\Gamma_{4}$ \\
icsd\_202705 & F$_{6}$Fe$_{2}$Li & 102 & 34.158 & 1.49 & $\Gamma_{5}$ \\
icsd\_067711 & Ba$_{2}$Fe$_{3}$O$_{8}$Y & 123 & 47.252 & 0.00 & $\Gamma_{5}^{+}$ \\
icsd\_015521 & ClFe$_{3}$O$_{8}$Pb$_{4}$ & 123 & 65.486 & 0.10 & $\Gamma_{5}^{+}$ \\
icsd\_053505 & FeNNi & 123 & 65.486 & 0.00 & $\Gamma_{5}^{+}$ \\
icsd\_613327 & B$_{2}$Co$_{5}$Ta$_{3}$ & 127 & 65.486 & 0.00 & $\Gamma_{5}^{+}$ \\
icsd\_614755 & B$_{2}$MnMo$_{2}$ & 127 & 55.358 & 0.00 & $\Gamma_{5}^{+}$ \\
icsd\_088317 & B$_{2}$V$_{3}$ & 127 & 65.486 & 0.00 & $\Gamma_{5}^{+}$ \\
icsd\_059553 & In$_{4}$Ti$_{3}$ & 127 & 55.358 & 0.00 & $\Gamma_{5}^{+}$ \\
icsd\_644412 & Mo$_{3}$Si$_{2}$ & 127 & 65.486 & 0.00 & $\Gamma_{5}^{+}$ \\
icsd\_016844 & AsFe$_{2}$ & 129 & 59.410 & 0.00 & $\Gamma_{5}^{+}$ \\
icsd\_093237 & AsFeMn & 129 & 129.417 & 0.00 & $\Gamma_{3}^{+}$ \\
icsd\_165984 & AsFeO$_{3}$Sr$_{2}$V & 129 & 59.410 & 0.00 & $\Gamma_{5}^{+}$ \\
icsd\_042329 & AsMn$_{2}$ & 129 & 129.417 & 0.00 & $\Gamma_{3}^{+}$ \\
icsd\_042325 & Mn$_{2}$Sb & 129 & 129.417 & 0.00 & $\Gamma_{3}^{+}$ \\
icsd\_200014 & MoO$_{6}$Rh$_{2}$ & 136 & 136.501 & 0.00 & $\Gamma_{3}^{+}$ \\
icsd\_032011 & As$_{2}$Ba$_{2}$Mn$_{3}$O$_{2}$ & 139 & 139.537 & 0.00 & $\Gamma_{3}^{+}$ \\
icsd\_032010 & As$_{2}$Mn$_{3}$O$_{2}$Sr$_{2}$ & 139 & 139.537 & 0.00 & $\Gamma_{3}^{+}$ \\
icsd\_246541 & Ba$_{2}$FeMoO$_{6}$ & 139 & 139.537 & 0.00 & $\Gamma_{3}^{+}$ \\
icsd\_032013 & Ba$_{2}$Mn$_{3}$O$_{2}$Sb$_{2}$ & 139 & 139.537 & 0.00 & $\Gamma_{3}^{+}$ \\
icsd\_032014 & Bi$_{2}$Mn$_{3}$O$_{2}$Sr$_{2}$ & 139 & 139.537 & 0.00 & $\Gamma_{3}^{+}$ \\
icsd\_617225 & BiTi$_{2}$ & 139 & 71.536 & 0.00 & $\Gamma_{5}^{+}$ \\
icsd\_094079 & FeMoO$_{6}$Sr$_{2}$ & 139 & 139.537 & 0.00 & $\Gamma_{3}^{+}$ \\
icsd\_084202 & Mn$_{3}$N$_{2}$ & 139 & 69.524 & 0.00 & $\Gamma_{5}^{+}$ \\
icsd\_032012 & Mn$_{3}$O$_{2}$Sb$_{2}$Sr$_{2}$ & 139 & 139.537 & 0.00 & $\Gamma_{3}^{+}$ \\
icsd\_188743 & MoO$_{6}$OsPb$_{2}$ & 139 & 139.537 & 0.00 & $\Gamma_{3}^{+}$ \\
icsd\_188742 & MoO$_{6}$OsSn$_{2}$ & 139 & 139.537 & 0.00 & $\Gamma_{3}^{+}$ \\
icsd\_246426 & Bi$_{2}$CrFeO$_{6}$ & 146 & 146.10 & 1.41 & $\Gamma_{1}$ \\
icsd\_031853 & MnNiO$_{3}$ & 148 & 2.4 & 0.90 & $\Gamma_{2}^+\Gamma_{3}^+$ \\
icsd\_626435 & CrNiP & 150 & 38.189 & 0.00 & $\Gamma_{3}$ \\
icsd\_029132 & F$_{3}$Fe & 150 & 5.13 & 0.00 & $\Gamma_{3}$ \\
icsd\_029134 & F$_{3}$Rh & 150 & 5.15 & 0.00 & $\Gamma_{3}$ \\
icsd\_155025 & Fe$_{2}$In$_{2}$Se$_{5}$ & 164 & 2.4 & 0.00 & $\Gamma_{3}^{+}$ \\
icsd\_062661 & Mn$_{3}$Nb$_{6}$O$_{11}$ & 164 & 12.58 & 0.25 & $\Gamma_{3}^{+}$ \\
icsd\_076020 & O$_{2}$PTi$_{3}$ & 164 & 164.89 & 0.00 & $\Gamma_{2}^{+}$ \\
icsd\_670856 & B$_{4}$Fe & 187 & 187.213 & 0.00 & $\Gamma_{2}$ \\
icsd\_610130 & AsCr$_{2}$ & 189 & 189.225 & 0.00 & $\Gamma_{4}$ \\
icsd\_043913 & AsCrNi & 189 & 189.225 & 0.00 & $\Gamma_{4}$ \\
icsd\_610275 & AsCrTi & 189 & 189.225 & 0.00 & $\Gamma_{4}$ \\
icsd\_610883 & AsMnNi & 189 & 38.191 & 0.00 & $\Gamma_{6}$ \\
icsd\_610927 & AsMnTi & 189 & 189.225 & 0.00 & $\Gamma_{4}$ \\
icsd\_042943 & CoGeTi & 189 & 38.191 & 0.00 & $\Gamma_{6}$ \\
icsd\_600596 & CrNiP & 189 & 38.191 & 0.00 & $\Gamma_{6}$ \\
icsd\_043394 & Mn$_{2}$P & 189 & 38.191 & 0.00 & $\Gamma_{6}$ \\
icsd\_643671 & MnSiTi & 189 & 189.225 & 0.00 & $\Gamma_{4}$ \\
icsd\_614407 & BGe$_{3}$V$_{5}$ & 193 & 63.464 & 0.00 & $\Gamma_{6}^{+}$ \\
icsd\_609885 & CAs$_{3}$V$_{5}$ & 193 & 63.464 & 0.00 & $\Gamma_{6}^{+}$ \\
icsd\_042585 & Fe$_{5}$Si$_{3}$ & 193 & 193.260 & 0.00 & $\Gamma_{2}^{+}$ \\
icsd\_643689 & Mn$_{3}$Si$_{3}$V$_{2}$ & 193 & 193.260 & 0.00 & $\Gamma_{2}^{+}$ \\
icsd\_182095 & B$_{4}$Mo & 194 & 63.463 & 0.00 & $\Gamma_{6}^{+}$ \\
icsd\_624067 & Co$_{2}$Mg & 194 & 63.464 & 0.00 & $\Gamma_{6}^{+}$ \\
\hline
\end{tabular}
\end{table*}
\clearpage

\begin{table*}[htbp]
\centering
\caption{Tabulated information on \textbf{collinear ferrimagnetic} materials, including the chemical formula, 
space group, magnetic space group, band gap and corresponding irreducible representations of crystallographic space group.}
\renewcommand{\arraystretch}{0.8}
\begin{tabular}{cccccc}
\hline
ICSD number & Chemical formula & SG NUM & BNS & Band Gap (eV)  & Irrep \\
\hline
icsd\_102673 & Co$_{2}$Sn & 194 & 194.270 & 0.00 & $\Gamma_{2}^{+}$ \\
icsd\_189226 & Co$_{3}$SiTi$_{2}$ & 194 & 11.54 & 0.00 & $\Gamma_{6}^{+}$ \\
icsd\_163332 & Mn$_{2}$Sb & 194 & 187.213 & 0.00 & $\Gamma_{2}^{+}$ \\
icsd\_670785 & AlCrHfV & 216 & 160.67 & 1.06 & $\Gamma_{5}$ \\
icsd\_670784 & AlCrVZr & 216 & 160.67 & 1.06 & $\Gamma_{5}$ \\
icsd\_670799 & CaCrPV & 216 & 160.67 & 0.11 & $\Gamma_{5}$ \\
icsd\_191684 & CoCrTe & 216 & 119.319 & 0.00 & $\Gamma_{5}$ \\
icsd\_670707 & CoFeGeZr & 216 & 44.231 & 0.00 & $\Gamma_{5}$ \\
icsd\_190988 & CoMnS & 216 & 119.319 & 0.00 & $\Gamma_{5}$ \\
icsd\_053001 & CoMnSb & 216 & 160.67 & 0.00 & $\Gamma_{5}$ \\
icsd\_190989 & CoMnSe & 216 & 119.319 & 0.00 & $\Gamma_{5}$ \\
icsd\_190990 & CoMnTe & 216 & 119.319 & 0.00 & $\Gamma_{5}$ \\
icsd\_053070 & CoSbTi & 216 & 44.231 & 0.00 & $\Gamma_{5}$ \\
icsd\_053071 & CoSbV & 216 & 160.67 & 0.00 & $\Gamma_{5}$ \\
icsd\_185079 & CoSnV & 216 & 119.319 & 0.00 & $\Gamma_{5}$ \\
icsd\_191682 & CoTeV & 216 & 119.319 & 0.00 & $\Gamma_{5}$ \\
icsd\_191685 & CrFeTe & 216 & 44.231 & 0.00 & $\Gamma_{5}$ \\
icsd\_670788 & CrGaHfV & 216 & 44.231 & 0.98 & $\Gamma_{5}$ \\
icsd\_670787 & CrGaVZr & 216 & 160.67 & 1.07 & $\Gamma_{5}$ \\
icsd\_670793 & CrGeScV & 216 & 44.231 & 0.78 & $\Gamma_{5}$ \\
icsd\_670796 & CrGeVY & 216 & 44.231 & 0.69 & $\Gamma_{5}$ \\
icsd\_670791 & CrHfInV & 216 & 160.67 & 0.94 & $\Gamma_{5}$ \\
icsd\_670790 & CrInVZr & 216 & 44.231 & 1.00 & $\Gamma_{5}$ \\
icsd\_670798 & CrKSV & 216 & 160.67 & 0.00 & $\Gamma_{5}$ \\
icsd\_182484 & CrNiSb & 216 & 44.231 & 0.00 & $\Gamma_{5}$ \\
icsd\_670801 & CrPSrV & 216 & 160.67 & 0.25 & $\Gamma_{5}$ \\
icsd\_670800 & CrRbSV & 216 & 44.231 & 0.00 & $\Gamma_{5}$ \\
icsd\_670792 & CrScSiV & 216 & 44.231 & 0.81 & $\Gamma_{5}$ \\
icsd\_670794 & CrScSnV & 216 & 160.67 & 0.66 & $\Gamma_{5}$ \\
icsd\_670795 & CrSiVY & 216 & 160.67 & 0.80 & $\Gamma_{5}$ \\
icsd\_670797 & CrSnVY & 216 & 44.231 & 0.58 & $\Gamma_{5}$ \\
icsd\_191687 & FeMnTe & 216 & 44.231 & 0.00 & $\Gamma_{5}$ \\
icsd\_053537 & FeSbTi & 216 & 160.67 & 0.00 & $\Gamma_{5}$ \\
icsd\_053539 & FeSbV & 216 & 119.319 & 0.00 & $\Gamma_{5}$ \\
icsd\_106680 & FeSnTi & 216 & 160.67 & 0.00 & $\Gamma_{5}$ \\
icsd\_191683 & FeTeV & 216 & 119.319 & 0.00 & $\Gamma_{5}$ \\
icsd\_184947 & GeMn$_{2}$ & 216 & 160.67 & 0.00 & $\Gamma_{5}$ \\
icsd\_670705 & GeMnVZr & 216 & 160.67 & 0.00 & $\Gamma_{5}$ \\
icsd\_044660 & IrMnSb & 216 & 160.67 & 0.00 & $\Gamma_{5}$ \\
icsd\_184948 & Mn$_{2}$Sb & 216 & 44.231 & 0.00 & $\Gamma_{5}$ \\
icsd\_671535 & Mn$_{2}$Si & 216 & 160.67 & 0.00 & $\Gamma_{5}$ \\
icsd\_161714 & MnNiP & 216 & 119.319 & 0.00 & $\Gamma_{5}$ \\
icsd\_054343 & MnRhSb & 216 & 44.231 & 0.00 & $\Gamma_{5}$ \\
icsd\_670704 & MnSiVZr & 216 & 44.231 & 0.00 & $\Gamma_{5}$ \\
icsd\_076702 & NiSbV & 216 & 44.231 & 0.00 & $\Gamma_{5}$ \\
icsd\_107127 & RuSbTi & 216 & 119.319 & 0.00 & $\Gamma_{5}$ \\
icsd\_107124 & RuSbV & 216 & 119.319 & 0.02 & $\Gamma_{5}$ \\
icsd\_043847 & CAlCo$_{3}$ & 221 & 123.345 & 0.00 & $\Gamma_{4}^{+}$ \\
icsd\_076790 & CCo$_{3}$Mg & 221 & 123.345 & 0.00 & $\Gamma_{4}^{+}$ \\
icsd\_076793 & CCo$_{3}$Sc & 221 & 47.252 & 0.00 & $\Gamma_{4}^{+}$ \\
icsd\_077152 & CMgNi$_{3}$ & 221 & 47.252 & 0.00 & $\Gamma_{4}^{+}$ \\
icsd\_077394 & CRu$_{3}$V & 221 & 123.345 & 0.00 & $\Gamma_{4}^{+}$ \\
icsd\_053506 & Fe$_{3}$NPd & 221 & 123.345 & 0.00 & $\Gamma_{4}^{+}$ \\
icsd\_044864 & Fe$_{3}$NPt & 221 & 123.345 & 0.00 & $\Gamma_{4}^{+}$ \\
icsd\_053502 & Fe$_{4}$N & 221 & 123.345 & 0.00 & $\Gamma_{4}^{+}$ \\
icsd\_044369 & Mn$_{4}$N & 221 & 123.345 & 0.00 & $\Gamma_{4}^{+}$ \\
icsd\_106087 & SnTi$_{3}$ & 221 & 123.345 & 0.00 & $\Gamma_{4}^{+}$ \\
icsd\_057600 & AlCo$_{2}$Cr & 225 & 139.537 & 0.00 & $\Gamma_{4}^{+}$ \\
icsd\_185966 & AlCo$_{2}$Ti & 225 & 139.537 & 0.00 & $\Gamma_{4}^{+}$ \\
icsd\_057643 & AlCo$_{2}$V & 225 & 166.101 & 0.00 & $\Gamma_{4}^{+}$ \\
icsd\_057654 & AlCrFe$_{2}$ & 225 & 139.537 & 0.00 & $\Gamma_{4}^{+}$ \\
icsd\_057806 & AlFe$_{2}$Mn & 225 & 71.536 & 0.00 & $\Gamma_{4}^{+}$ \\
icsd\_057807 & AlFe$_{2}$Mo & 225 & 166.101 & 0.00 & $\Gamma_{4}^{+}$ \\
icsd\_057827 & AlFe$_{2}$Ti & 225 & 166.101 & 0.00 & $\Gamma_{4}^{+}$ \\
icsd\_057832 & AlFe$_{2}$V & 225 & 166.101 & 0.00 & $\Gamma_{4}^{+}$ \\
\hline
\end{tabular}
\end{table*}
\clearpage

\begin{table*}[htbp]
\centering
\caption{Tabulated information on \textbf{collinear ferrimagnetic} materials, including the chemical formula, 
space group, magnetic space group, band gap and corresponding irreducible representations of crystallographic space group.}
\renewcommand{\arraystretch}{0.8}
\begin{tabular}{cccccc}
\hline
ICSD number & Chemical formula & SG NUM & BNS & Band Gap (eV)  & Irrep \\
\hline
icsd\_057994 & AlMn$_{2}$V & 225 & 166.101 & 0.00 & $\Gamma_{4}^{+}$ \\
icsd\_186059 & AsFe$_{2}$Ti & 225 & 166.101 & 0.00 & $\Gamma_{4}^{+}$ \\
icsd\_102318 & Co$_{2}$CrGa & 225 & 139.537 & 0.00 & $\Gamma_{4}^{+}$ \\
icsd\_416260 & Co$_{2}$CrIn & 225 & 139.537 & 0.00 & $\Gamma_{4}^{+}$ \\
icsd\_102453 & Co$_{2}$GaTi & 225 & 139.537 & 0.00 & $\Gamma_{4}^{+}$ \\
icsd\_102456 & Co$_{2}$GaV & 225 & 166.101 & 0.00 & $\Gamma_{4}^{+}$ \\
icsd\_052989 & Co$_{2}$GeTi & 225 & 71.536 & 0.00 & $\Gamma_{4}^{+}$ \\
icsd\_053080 & Co$_{2}$SiTi & 225 & 139.537 & 0.00 & $\Gamma_{4}^{+}$ \\
icsd\_102682 & Co$_{2}$SnTi & 225 & 139.537 & 0.00 & $\Gamma_{4}^{+}$ \\
icsd\_102684 & Co$_{2}$SnV & 225 & 166.101 & 0.00 & $\Gamma_{4}^{+}$ \\
icsd\_102437 & CoGa$_{2}$Mn & 225 & 166.101 & 0.00 & $\Gamma_{4}^{+}$ \\
icsd\_102755 & CrFe$_{2}$Ga & 225 & 139.537 & 0.00 & $\Gamma_{4}^{+}$ \\
icsd\_185999 & CrFe$_{2}$Sn & 225 & 71.536 & 0.00 & $\Gamma_{4}^{+}$ \\
icsd\_186721 & Fe$_{2}$GaMn & 225 & 166.101 & 0.00 & $\Gamma_{4}^{+}$ \\
icsd\_103469 & Fe$_{2}$GaTi & 225 & 139.537 & 0.00 & $\Gamma_{4}^{+}$ \\
icsd\_103473 & Fe$_{2}$GaV & 225 & 71.536 & 0.00 & $\Gamma_{4}^{+}$ \\
icsd\_186056 & Fe$_{2}$InTi & 225 & 166.101 & 0.00 & $\Gamma_{4}^{+}$ \\
icsd\_186060 & Fe$_{2}$SbTi & 225 & 71.536 & 0.00 & $\Gamma_{4}^{+}$ \\
icsd\_053555 & Fe$_{2}$SiV & 225 & 166.101 & 0.00 & $\Gamma_{4}^{+}$ \\
icsd\_103641 & Fe$_{2}$SnTi & 225 & 166.101 & 0.00 & $\Gamma_{4}^{+}$ \\
icsd\_103644 & Fe$_{2}$SnV & 225 & 166.101 & 0.00 & $\Gamma_{4}^{+}$ \\
icsd\_103813 & GaMn$_{2}$V & 225 & 166.101 & 0.00 & $\Gamma_{4}^{+}$ \\
icsd\_188332 & GaMn$_{3}$ & 225 & 166.101 & 0.00 & $\Gamma_{4}^{+}$ \\
icsd\_188334 & GeMn$_{3}$ & 225 & 166.101 & 0.00 & $\Gamma_{4}^{+}$ \\
icsd\_671340 & GeRu$_{2}$V & 225 & 166.101 & 0.00 & $\Gamma_{4}^{+}$ \\
icsd\_076227 & Mn$_{3}$Si & 225 & 166.101 & 0.00 & $\Gamma_{4}^{+}$ \\
icsd\_188333 & Mn$_{3}$Sn & 225 & 166.101 & 0.00 & $\Gamma_{4}^{+}$ \\
icsd\_671341 & Ru$_{2}$SbV & 225 & 166.101 & 0.00 & $\Gamma_{4}^{+}$ \\
\hline
\end{tabular}
\label{ColFiMfinal}
\end{table*}

\newpage

\subsection{Noncollinear ferrimagnetic materials}
The relevant information for noncollinear ferrimagnetic materials is summarized in Table \ref{NoCFiM}-\ref{NoCFiMfinal}, including their chemical formula, space group, magnetic space group, band gap and corresponding irreducible representations of crystallographic space group.
\begin{table*}[!h]
\centering
\caption{Tabulated information on \textbf{noncollinear ferrimagnetic} materials, including the chemical formula, 
space group, magnetic space group, band gap and corresponding irreducible representations of crystallographic space group.}
\renewcommand{\arraystretch}{0.8}
\begin{tabular}{cccccc}
\hline
ICSD number & Chemical formula & SG NUM & BNS & Band Gap (eV)  & Irrep \\
\hline
icsd\_065295 & Cs$_{4}$Cu$_{3}$F$_{10}$ & 2 & 1.1 & 3.20 & $\Gamma_{1}^{-}$ \\
icsd\_416823 & HCoO$_{5}$PZn & 2 & 2.4 & 1.69 & $\Gamma_{1}^{+}$ \\
icsd\_000902 & AsClCo$_{2}$O$_{4}$ & 11 & 11.50 & 3.38 & $\Gamma_{1}^{+}$ \\
icsd\_415798 & Cl$_{2}$Co$_{2}$O$_{3}$Te & 11 & 11.50 & 2.74 & $\Gamma_{1}^{+}$ \\
icsd\_657748 & O$_{2}$Ti & 11 & 2.4 & 0.00 & $\Gamma_{2}^{+}$ \\
icsd\_088156 & Ba$_{2}$IrLaO$_{6}$ & 14 & 14.79 & 0.50 & $\Gamma_{2}^{+}$ \\
icsd\_088158 & Ba$_{2}$IrLuO$_{6}$ & 14 & 14.79 & 0.27 & $\Gamma_{2}^{+}$ \\
icsd\_088153 & Ba$_{2}$IrO$_{6}$Sc & 14 & 14.75 & 0.09 & $\Gamma_{1}^{+}$ \\
icsd\_088155 & Ba$_{2}$IrO$_{6}$Y & 14 & 14.79 & 0.19 & $\Gamma_{2}^{+}$ \\
icsd\_152444 & Ca$_{2}$NiO$_{6}$Os & 14 & 14.79 & 0.12 & $\Gamma_{2}^{+}$ \\
icsd\_079495 & CoIrLa$_{2}$O$_{6}$ & 14 & 14.75 & 0.45 & $\Gamma_{1}^{+}$ \\
icsd\_030410 & CuO$_{6}$Sb$_{2}$ & 14 & 14.79 & 1.28 & $\Gamma_{2}^{+}$ \\
icsd\_165398 & F$_{4}$Ru & 14 & 14.75 & 1.55 & $\Gamma_{1}^{+}$ \\
icsd\_006044 & F$_{6}$Li$_{2}$Rh & 14 & 14.75 & 0.47 & $\Gamma_{1}^{+}$ \\
icsd\_195628 & FeMn$_{2}$O$_{6}$Re & 14 & 14.75 & 0.00 & $\Gamma_{1}^{+}$ \\
icsd\_238316 & InO$_{6}$OsSr$_{2}$ & 14 & 14.79 & 1.02 & $\Gamma_{2}^{+}$ \\
icsd\_414605 & IrLa$_{2}$LiO$_{6}$ & 14 & 14.79 & 0.36 & $\Gamma_{2}^{+}$ \\
icsd\_079492 & IrLa$_{2}$MgO$_{6}$ & 14 & 14.79 & 0.59 & $\Gamma_{2}^{+}$ \\
icsd\_413634 & IrLa$_{2}$NaO$_{6}$ & 14 & 14.79 & 0.47 & $\Gamma_{2}^{+}$ \\
icsd\_079494 & IrLa$_{2}$NiO$_{6}$ & 14 & 14.75 & 0.52 & $\Gamma_{1}^{+}$ \\
icsd\_075596 & IrLa$_{2}$O$_{6}$Zn & 14 & 14.79 & 0.50 & $\Gamma_{2}^{+}$ \\
icsd\_088157 & IrLuO$_{6}$Sr$_{2}$ & 14 & 14.79 & 0.24 & $\Gamma_{2}^{+}$ \\
icsd\_088152 & IrO$_{6}$ScSr$_{2}$ & 14 & 14.79 & 0.02 & $\Gamma_{2}^{+}$ \\
icsd\_088154 & IrO$_{6}$Sr$_{2}$Y & 14 & 14.79 & 0.26 & $\Gamma_{2}^{+}$ \\
icsd\_416199 & La$_{2}$LiO$_{6}$Os & 14 & 14.79 & 1.00 & $\Gamma_{2}^{+}$ \\
icsd\_088522 & La$_{2}$MgO$_{6}$Rh & 14 & 14.75 & 0.00 & $\Gamma_{1}^{+}$ \\
icsd\_088523 & La$_{2}$O$_{6}$RhZn & 14 & 14.79 & 0.09 & $\Gamma_{2}^{+}$ \\
icsd\_159030 & CaIrO$_{3}$ & 36 & 36.174 & 0.34 & $\Gamma_{4}$ \\
icsd\_429116 & BRuTa & 51 & 51.295 & 0.00 & $\Gamma_{3}^{+}$ \\
icsd\_263013 & Fe$_{3}$O$_{4}$ & 51 & 51.295 & 0.00 & $\Gamma_{3}^{+}$ \\
icsd\_612536 & B$_{2}$BaNi$_{2}$ & 58 & 58.398 & 0.00 & $\Gamma_{3}^{+}$ \\
icsd\_615019 & B$_{2}$Ni$_{2}$Sr & 58 & 14.75 & 0.00 & $\Gamma_{4}^{+}$ \\
icsd\_406953 & AsCoHf & 62 & 62.446 & 0.00 & $\Gamma_{2}^{+}$ \\
icsd\_193272 & Bi$_{3}$Co & 62 & 62.447 & 0.00 & $\Gamma_{3}^{+}$ \\
icsd\_245840 & CaCrO$_{3}$ & 62 & 62.448 & 0.40 & $\Gamma_{4}^{+}$ \\
icsd\_159433 & CaIrO$_{3}$ & 62 & 62.448 & 0.15 & $\Gamma_{4}^{+}$ \\
icsd\_167128 & CCoFe$_{2}$ & 62 & 62.447 & 0.00 & $\Gamma_{3}^{+}$ \\
icsd\_670824 & CCr$_{2}$Fe & 62 & 62.446 & 0.00 & $\Gamma_{2}^{+}$ \\
icsd\_181711 & CCr$_{3}$ & 62 & 62.446 & 0.00 & $\Gamma_{2}^{+}$ \\
icsd\_670838 & CFeV$_{2}$ & 62 & 62.446 & 0.00 & $\Gamma_{2}^{+}$ \\
icsd\_251180 & CMn$_{3}$ & 62 & 62.446 & 0.00 & $\Gamma_{2}^{+}$ \\
icsd\_625259 & Co$_{3}$Sn$_{2}$ & 62 & 62.447 & 0.00 & $\Gamma_{3}^{+}$ \\
icsd\_636746 & GeIrTi & 62 & 62.446 & 0.00 & $\Gamma_{2}^{+}$ \\
icsd\_196446 & IrO$_{3}$Sr & 62 & 62.448 & 0.07 & $\Gamma_{4}^{+}$ \\
icsd\_075569 & LaO$_{3}$Ru & 62 & 62.447 & 0.61 & $\Gamma_{3}^{+}$ \\
icsd\_056697 & O$_{3}$RuSr & 62 & 62.447 & 0.00 & $\Gamma_{3}^{+}$ \\
icsd\_236435 & CoO$_{6}$OsSr$_{2}$ & 87 & 12.62 & 0.04 & $\Gamma_{3}^+\Gamma_{4}^+$ \\
icsd\_245819 & CuO$_{6}$OsSr$_{2}$ & 87 & 12.62 & 0.00 & $\Gamma_{3}^+\Gamma_{4}^+$ \\
icsd\_024563 & S$_{4}$V$_{5}$ & 87 & 12.62 & 0.00 & $\Gamma_{3}^+\Gamma_{4}^+$ \\
icsd\_652166 & Se$_{4}$V$_{5}$ & 87 & 12.62 & 0.33 & $\Gamma_{3}^+\Gamma_{4}^+$ \\
icsd\_023173 & F$_{6}$Li$_{2}$Mo & 94 & 18.19 & 1.13 & $\Gamma_{5}$ \\
icsd\_025751 & Cr$_{3}$GeN & 113 & 18.19 & 0.00 & $\Gamma_{5}$ \\
icsd\_030447 & BCo$_{2}$ & 121 & 72.544 & 0.00 & $\Gamma_{5}$ \\
icsd\_160691 & CCr$_{2}$LaSi$_{2}$ & 123 & 65.486 & 0.00 & $\Gamma_{5}^{+}$ \\
icsd\_187494 & FeGaNi$_{2}$ & 123 & 12.58 & 0.00 & $\Gamma_{5}^{+}$ \\
icsd\_187493 & GaMnNi$_{2}$ & 123 & 12.58 & 0.00 & $\Gamma_{5}^{+}$ \\
icsd\_021110 & CuF$_{3}$K & 127 & 55.358 & 2.49 & $\Gamma_{5}^{+}$ \\
icsd\_611100 & As$_{2}$Ni$_{4}$Y & 136 & 65.486 & 0.00 & $\Gamma_{5}^{+}$ \\
icsd\_166673 & CoO$_{6}$Ta$_{2}$ & 136 & 58.398 & 3.01 & $\Gamma_{5}^{+}$ \\
icsd\_418676 & CrF$_{6}$Li$_{2}$ & 136 & 58.398 & 1.01 & $\Gamma_{5}^{+}$ \\
icsd\_424578 & Cs$_{3}$NiO$_{2}$ & 136 & 58.398 & 1.58 & $\Gamma_{5}^{+}$ \\
icsd\_084789 & CuO$_{6}$Sb$_{2}$ & 136 & 58.398 & 1.30 & $\Gamma_{5}^{+}$ \\
icsd\_074565 & F$_{6}$Li$_{2}$Mo & 136 & 58.398 & 1.20 & $\Gamma_{5}^{+}$ \\
icsd\_095778 & F$_{6}$Li$_{2}$Rh & 136 & 58.398 & 0.47 & $\Gamma_{5}^{+}$ \\
icsd\_040337 & FeO$_{6}$Ta$_{2}$ & 136 & 58.398 & 2.36 & $\Gamma_{5}^{+}$ \\
\hline
\end{tabular}
\label{NoCFiM}
\end{table*}
\clearpage

\begin{table*}[htbp]
\centering
\caption{Tabulated information on \textbf{noncollinear ferrimagnetic} materials, including the chemical formula, 
space group, magnetic space group, band gap and corresponding irreducible representations of crystallographic space group.}
\renewcommand{\arraystretch}{0.8}
\begin{tabular}{cccccc}
\hline
ICSD number & Chemical formula & SG NUM & BNS & Band Gap (eV)  & Irrep \\
\hline
icsd\_262579 & K$_{3}$NiO$_{2}$ & 136 & 58.398 & 1.58 & $\Gamma_{5}^{+}$ \\
icsd\_424579 & NiO$_{2}$Rb$_{3}$ & 136 & 58.398 & 1.31 & $\Gamma_{5}^{+}$ \\
icsd\_025775 & CGeMn$_{3}$ & 140 & 72.544 & 0.00 & $\Gamma_{5}^{+}$ \\
icsd\_024651 & Fe$_{2}$N & 149 & 162.77 & 0.00 & $\Gamma_{2}$ \\
icsd\_200999 & Li$_{2}$O$_{3}$Re & 161 & 9.37 & 0.37 & $\Gamma_{3}$ \\
icsd\_044612 & Fe$_{2}$N & 162 & 162.77 & 0.00 & $\Gamma_{2}^{+}$ \\
icsd\_041814 & Sb$_{2}$V$_{3}$ & 166 & 12.58 & 0.00 & $\Gamma_{3}^{+}$ \\
icsd\_016673 & F$_{3}$Ru & 167 & 15.85 & 1.39 & $\Gamma_{3}^{+}$ \\
icsd\_016649 & F$_{3}$Ti & 167 & 15.85 & 2.19 & $\Gamma_{3}^{+}$ \\
icsd\_030624 & F$_{3}$V & 167 & 15.85 & 2.03 & $\Gamma_{3}^{+}$ \\
icsd\_088670 & BaCoO$_{3}$ & 187 & 38.191 & 1.35 & $\Gamma_{6}$ \\
icsd\_624869 & Co$_{2}$S$_{6}$Ta$_{9}$ & 189 & 38.189 & 0.00 & $\Gamma_{6}$ \\
icsd\_623085 & CoGaHf & 189 & 38.189 & 0.00 & $\Gamma_{6}$ \\
icsd\_623254 & CoGaZr & 189 & 38.191 & 0.00 & $\Gamma_{6}$ \\
icsd\_626107 & Cr$_{6}$Ge$_{6}$Sc & 191 & 191.239 & 0.00 & $\Gamma_{3}^{+}$ \\
icsd\_658018 & Cr$_{6}$Ge$_{6}$Y & 191 & 191.239 & 0.00 & $\Gamma_{3}^{+}$ \\
icsd\_029285 & NP$_{3}$V$_{5}$ & 193 & 193.258 & 0.00 & $\Gamma_{4}^{+}$ \\
icsd\_016839 & CoSi & 198 & 19.27 & 0.00 & $\Gamma_{4}$ \\
icsd\_166458 & N$_{2}$Os & 205 & 61.436 & 0.00 & $\Gamma_{4}^{+}$ \\
icsd\_635637 & Ga$_{2}$V$_{3}$ & 213 & 155.45 & 0.00 & $\Gamma_{5}$ \\
icsd\_052592 & AgMn$_{3}$N & 221 & 166.97 & 0.00 & $\Gamma_{5}^{+}$ \\
icsd\_058547 & AuNV$_{3}$ & 221 & 12.58 & 0.00 & $\Gamma_{5}^{+}$ \\
icsd\_043853 & CAlFe$_{3}$ & 221 & 12.62 & 0.00 & $\Gamma_{4}^{+}$ \\
icsd\_043860 & CAlMn$_{3}$ & 221 & 12.58 & 0.00 & $\Gamma_{5}^{+}$ \\
icsd\_076842 & CFe$_{3}$Sn & 221 & 166.101 & 0.00 & $\Gamma_{4}^{+}$ \\
icsd\_076763 & CFe$_{3}$Zn & 221 & 65.486 & 0.00 & $\Gamma_{4}^{+}$ \\
icsd\_023586 & CGaMn$_{3}$ & 221 & 12.62 & 0.00 & $\Gamma_{4}^{+}$ \\
icsd\_044351 & CGeMn$_{3}$ & 221 & 12.58 & 0.00 & $\Gamma_{5}^{+}$ \\
icsd\_077036 & CInMn$_{3}$ & 221 & 12.62 & 0.00 & $\Gamma_{4}^{+}$ \\
icsd\_077153 & CMn$_{3}$Sn & 221 & 12.58 & 0.00 & $\Gamma_{5}^{+}$ \\
icsd\_247066 & Co$_{3}$InN & 221 & 10.46 & 0.00 & $\Gamma_{4}^{+}$ \\
icsd\_053125 & Cr$_{3}$GaN & 221 & 166.97 & 0.00 & $\Gamma_{5}^{+}$ \\
icsd\_053132 & Cr$_{3}$IrN & 221 & 166.101 & 0.00 & $\Gamma_{4}^{+}$ \\
icsd\_053143 & Cr$_{3}$NRh & 221 & 166.101 & 0.00 & $\Gamma_{4}^{+}$ \\
icsd\_053145 & Cr$_{3}$NSn & 221 & 12.58 & 0.00 & $\Gamma_{5}^{+}$ \\
icsd\_053306 & CuMn$_{3}$N & 221 & 166.97 & 0.00 & $\Gamma_{5}^{+}$ \\
icsd\_183372 & CuNNi$_{3}$ & 221 & 65.486 & 0.00 & $\Gamma_{4}^{+}$ \\
icsd\_044865 & Fe$_{3}$NNi & 221 & 166.101 & 0.00 & $\Gamma_{4}^{+}$ \\
icsd\_153274 & Fe$_{3}$NRh & 221 & 12.62 & 0.00 & $\Gamma_{4}^{+}$ \\
icsd\_087399 & GaMn$_{3}$N & 221 & 12.58 & 0.00 & $\Gamma_{5}^{+}$ \\
icsd\_097743 & GeMn$_{3}$ & 221 & 166.101 & 0.00 & $\Gamma_{4}^{+}$ \\
icsd\_044659 & IrMn$_{3}$N & 221 & 65.486 & 0.00 & $\Gamma_{4}^{+}$ \\
icsd\_076056 & Mn$_{3}$NNi & 221 & 166.101 & 0.00 & $\Gamma_{4}^{+}$ \\
icsd\_076057 & Mn$_{3}$NPd & 221 & 166.101 & 0.00 & $\Gamma_{4}^{+}$ \\
icsd\_076058 & Mn$_{3}$NPt & 221 & 166.101 & 0.00 & $\Gamma_{4}^{+}$ \\
icsd\_076060 & Mn$_{3}$NRh & 221 & 166.101 & 0.00 & $\Gamma_{4}^{+}$ \\
icsd\_076062 & Mn$_{3}$NSn & 221 & 166.101 & 0.00 & $\Gamma_{4}^{+}$ \\
icsd\_076070 & Mn$_{3}$NZn & 221 & 166.97 & 0.00 & $\Gamma_{5}^{+}$ \\
icsd\_096119 & Mn$_{3}$Sb & 221 & 166.101 & 0.00 & $\Gamma_{4}^{+}$ \\
icsd\_076403 & NNi$_{4}$ & 221 & 166.97 & 0.00 & $\Gamma_{5}^{+}$ \\
\hline
\end{tabular}
\label{NoCFiMfinal}
\end{table*}

\newpage
\subsection{Collinear antiferromagnetic materials}
The relevant information for collinear antiferromagnetic materials is summarized in Table \ref{ColAFM}-\ref{ColAFMfinal}, including their chemical formula, space group, magnetic space group, band gap and corresponding irreducible representations of crystallographic space group.
\begin{table*}[!h]
\centering
\caption{Tabulated information on \textbf{collinear antiferromagnetic} materials, including the chemical formula, 
space group, magnetic space group, band gap and corresponding irreducible representations of crystallographic space group.}
\renewcommand{\arraystretch}{0.8}
% [inline block 1: 10 envs, 49152 chars -> data_tex | \begin{tabular}{cccccc} \hline...]

\label{ColAFMfinal}
\end{table*}

\newpage

\newpage
\subsection{Noncollinear antiferromagnetic materials}
The relevant information for noncollinear antiferromagnetic materials is summarized in Table \ref{NoCAFM}-\ref{NoCAFMfinal}, including their chemical formula, space group, magnetic space group, band gap and corresponding irreducible representations of crystallographic space group.
\begin{table*}[!h]
\centering
\caption{Tabulated information on \textbf{noncollinear antiferromagnetic} materials, including the chemical formula, 
space group, magnetic space group, band gap and corresponding irreducible representations of crystallographic space group.}
\renewcommand{\arraystretch}{0.8}
\begin{tabular}{cccccc}
\hline
ICSD number & Chemical formula & SG NUM & BNS & Band Gap (eV)  & Irrep \\
\hline
icsd\_000453 & Ni$_{3}$S$_{2}$Sn$_{2}$ & 12 & 12.58 & 0.00 & $\Gamma_{1}^{+}$ \\
icsd\_186046 & Fe$_{4}$Ge$_{2}$Lu & 58 & 58.396 & 0.00 & $\Gamma_{2}^{-}$ \\
icsd\_670828 & CFeMn$_{2}$ & 62 & 62.441 & 0.00 & $\Gamma_{1}^{+}$ \\
icsd\_185418 & MnO$_{3}$V & 62 & 62.441 & 0.78 & $\Gamma_{1}^{+}$ \\
icsd\_057009 & C$_{2}$Cr$_{3}$ & 63 & 63.465 & 0.00 & $\Gamma_{1}^{-}$ \\
icsd\_609880 & CAsCr$_{3}$ & 63 & 63.465 & 0.00 & $\Gamma_{1}^{-}$ \\
icsd\_291338 & CCr$_{3}$P & 63 & 63.459 & 0.00 & $\Gamma_{3}^{-}$ \\
icsd\_291339 & Cr$_{3}$NP & 63 & 63.464 & 0.00 & $\Gamma_{4}^{+}$ \\
icsd\_180767 & Ni$_{3}$S$_{2}$ & 63 & 63.459 & 0.00 & $\Gamma_{3}^{-}$ \\
icsd\_644620 & NPV$_{3}$ & 63 & 63.465 & 0.00 & $\Gamma_{1}^{-}$ \\
icsd\_055075 & Se$_{4}$Ti$_{5}$ & 87 & 87.79 & 0.01 & $\Gamma_{2}^{-}$ \\
icsd\_015451 & Te$_{4}$Ti$_{5}$ & 87 & 87.78 & 0.05 & $\Gamma_{1}^{-}$ \\
icsd\_102500 & CoIn$_{3}$ & 118 & 34.158 & 0.00 & $\Gamma_{5}$ \\
icsd\_042335 & AsCr$_{2}$ & 129 & 67.503 & 0.00 & $\Gamma_{5}^{-}$ \\
icsd\_024794 & Cr$_{2}$O$_{6}$Te & 136 & 58.395 & 1.74 & $\Gamma_{5}^{-}$ \\
icsd\_078778 & CrF$_{4}$ & 136 & 136.502 & 1.19 & $\Gamma_{4}^{-}$ \\
icsd\_613152 & B$_{4}$Co$_{4}$Lu & 137 & 137.510 & 0.00 & $\Gamma_{4}^{+}$ \\
icsd\_613410 & B$_{4}$Co$_{4}$Y & 137 & 137.510 & 0.00 & $\Gamma_{4}^{+}$ \\
icsd\_025760 & AsCr$_{3}$N & 140 & 140.543 & 0.00 & $\Gamma_{3}^{-}$ \\
icsd\_182435 & Mn$_{3}$O$_{6}$Te & 148 & 2.6 & 1.68 & $\Gamma_{2}^-\Gamma_{3}^-$ \\
icsd\_016316 & Mo$_{3}$Se$_{4}$ & 148 & 1.1 & 0.00 & $\Gamma_{1}^{-}$ \\
icsd\_020389 & Fe$_{3}$N & 149 & 182.181 & 0.00 & $\Gamma_{1}$ \\
icsd\_025813 & BaCoO$_{2}$ & 152 & 5.13 & 2.11 & $\Gamma_{3}$ \\
icsd\_004266 & FeO$_{4}$P & 152 & 152.35 & 2.69 & $\Gamma_{2}$ \\
icsd\_010424 & Ni$_{3}$S$_{2}$ & 155 & 5.15 & 0.00 & $\Gamma_{3}$ \\
icsd\_401027 & Cl$_{8}$Na$_{2}$Ti$_{3}$ & 160 & 8.32 & 1.85 & $\Gamma_{3}$ \\
icsd\_036207 & Fe$_{3}$O$_{7}$P & 160 & 160.67 & 2.31 & $\Gamma_{2}$ \\
icsd\_029312 & NiS & 160 & 160.65 & 0.00 & $\Gamma_{1}$ \\
icsd\_042596 & NiSe & 160 & 8.32 & 0.00 & $\Gamma_{3}$ \\
icsd\_001846 & Cl$_{8}$Mn$_{3}$Na$_{2}$ & 166 & 166.101 & 4.28 & $\Gamma_{2}^{+}$ \\
icsd\_401026 & Cl$_{8}$Na$_{2}$Ti$_{3}$ & 166 & 166.97 & 2.53 & $\Gamma_{1}^{+}$ \\
icsd\_291388 & Cs$_{2}$Cu$_{3}$F$_{12}$Sn & 166 & 12.62 & 3.55 & $\Gamma_{3}^{+}$ \\
icsd\_425834 & H$_{6}$Cl$_{2}$Cu$_{3}$O$_{6}$Zn & 166 & 12.62 & 2.25 & $\Gamma_{3}^{+}$ \\
icsd\_024176 & Ni$_{3}$Pb$_{2}$S$_{2}$ & 166 & 166.97 & 0.00 & $\Gamma_{1}^{+}$ \\
icsd\_100217 & Ni$_{3}$S$_{2}$Sn$_{2}$ & 166 & 12.58 & 0.00 & $\Gamma_{3}^{+}$ \\
icsd\_094318 & BLiMnO$_{3}$ & 174 & 174.135 & 2.94 & $\Gamma_{2}$ \\
icsd\_072920 & S$_{4}$V$_{3}$ & 176 & 11.53 & 0.00 & $\Gamma_{3}^-\Gamma_{5}^-$ \\
icsd\_638088 & Ge$_{2}$V & 180 & 180.169 & 0.00 & $\Gamma_{4}$ \\
icsd\_168997 & FeO$_{4}$P & 181 & 21.41 & 3.13 & $\Gamma_{6}$ \\
icsd\_069692 & Co$_{6}$LiP$_{4}$ & 187 & 187.211 & 0.00 & $\Gamma_{4}$ \\
icsd\_094412 & Co$_{6}$MgP$_{4}$ & 187 & 187.211 & 0.00 & $\Gamma_{4}$ \\
icsd\_251064 & Ag$_{2}$S$_{6}$TeV$_{3}$ & 189 & 189.224 & 0.00 & $\Gamma_{2}$ \\
icsd\_610509 & AsFeNi & 189 & 189.223 & 0.00 & $\Gamma_{3}$ \\
icsd\_610530 & AsFeTi & 189 & 189.223 & 0.00 & $\Gamma_{3}$ \\
icsd\_610532 & AsFeV & 189 & 38.191 & 0.00 & $\Gamma_{6}$ \\
icsd\_614205 & BFeTa & 189 & 38.191 & 0.00 & $\Gamma_{6}$ \\
icsd\_042735 & CoSiTi & 189 & 189.223 & 0.00 & $\Gamma_{3}$ \\
icsd\_002278 & CrCsF$_{4}$ & 189 & 189.224 & 2.12 & $\Gamma_{2}$ \\
icsd\_042060 & CrNbSi & 189 & 38.191 & 0.00 & $\Gamma_{6}$ \\
icsd\_042402 & Fe$_{2}$P & 189 & 38.191 & 0.00 & $\Gamma_{6}$ \\
icsd\_086364 & FeGeSc & 189 & 38.191 & 0.00 & $\Gamma_{6}$ \\
icsd\_632938 & FeNiP & 189 & 189.223 & 0.00 & $\Gamma_{3}$ \\
icsd\_290889 & FePTi & 189 & 189.224 & 0.00 & $\Gamma_{2}$ \\
icsd\_099080 & Ga$_{2}$Lu$_{3}$Mn$_{3}$Si & 189 & 189.223 & 0.00 & $\Gamma_{3}$ \\
icsd\_409925 & GePdTi & 189 & 38.189 & 0.00 & $\Gamma_{6}$ \\
icsd\_410967 & In$_{3}$Rh$_{2}$Ti$_{3}$ & 189 & 189.223 & 0.00 & $\Gamma_{3}$ \\
icsd\_086369 & MnScSi & 189 & 189.223 & 0.00 & $\Gamma_{3}$ \\
icsd\_643653 & MnSiTa & 189 & 189.224 & 0.00 & $\Gamma_{2}$ \\
icsd\_023550 & B$_{2}$Co$_{3}$Hf & 191 & 191.238 & 0.00 & $\Gamma_{4}^{+}$ \\
icsd\_044171 & B$_{2}$Co$_{3}$Lu & 191 & 65.486 & 0.00 & $\Gamma_{6}^{+}$ \\
icsd\_044179 & B$_{2}$Co$_{3}$Sc & 191 & 191.238 & 0.00 & $\Gamma_{4}^{+}$ \\
icsd\_023655 & B$_{2}$Co$_{3}$Y & 191 & 191.238 & 0.00 & $\Gamma_{4}^{+}$ \\
icsd\_044191 & B$_{2}$Co$_{3}$Zr & 191 & 191.238 & 0.00 & $\Gamma_{4}^{+}$ \\
icsd\_089437 & Ge$_{6}$Mn$_{6}$Sc & 191 & 191.237 & 0.00 & $\Gamma_{4}^{-}$ \\
icsd\_240144 & Mn$_{6}$Sn$_{6}$Y & 191 & 65.486 & 0.00 & $\Gamma_{6}^{+}$ \\
\hline
\end{tabular}
\label{NoCAFM}
\end{table*}
\clearpage

\begin{table*}[htbp]
\centering
\caption{Tabulated information on \textbf{noncollinear antiferromagnetic} materials, including the chemical formula, 
space group, magnetic space group, band gap and corresponding irreducible representations of crystallographic space group.}
\renewcommand{\arraystretch}{0.8}
\begin{tabular}{cccccc}
\hline
ICSD number & Chemical formula & SG NUM & BNS & Band Gap (eV)  & Irrep \\
\hline
icsd\_182148 & Sn$_{6}$V$_{6}$Y & 191 & 65.486 & 0.00 & $\Gamma_{6}^{+}$ \\
icsd\_635612 & Ga$_{3}$V$_{5}$ & 193 & 193.259 & 0.00 & $\Gamma_{3}^{+}$ \\
icsd\_044504 & Ge$_{3}$V$_{5}$ & 193 & 193.259 & 0.00 & $\Gamma_{3}^{+}$ \\
icsd\_191487 & Si$_{3}$V$_{5}$ & 193 & 193.259 & 0.00 & $\Gamma_{3}^{+}$ \\
icsd\_109292 & Sn$_{3}$Ti$_{5}$ & 193 & 193.255 & 0.00 & $\Gamma_{2}^{-}$ \\
icsd\_187992 & AlCo$_{3}$ & 194 & 194.269 & 0.00 & $\Gamma_{3}^{+}$ \\
icsd\_603351 & GaMn$_{3}$ & 194 & 63.463 & 0.00 & $\Gamma_{6}^{+}$ \\
icsd\_603343 & GeMn$_{3}$ & 194 & 63.464 & 0.00 & $\Gamma_{6}^{+}$ \\
icsd\_104978 & Mn$_{3}$Sn & 194 & 63.464 & 0.00 & $\Gamma_{6}^{+}$ \\
icsd\_652343 & SiTa$_{2}$V$_{3}$ & 194 & 194.271 & 0.00 & $\Gamma_{1}^{-}$ \\
icsd\_106098 & SnV$_{3}$ & 194 & 194.268 & 0.00 & $\Gamma_{4}^{+}$ \\
icsd\_093901 & AsNiSe & 198 & 198.9 & 0.00 & $\Gamma_{1}$ \\
icsd\_624862 & CoSSb & 198 & 19.25 & 0.24 & $\Gamma_{2}\Gamma_{3}$ \\
icsd\_100568 & F$_{2}$Pd & 198 & 198.9 & 1.54 & $\Gamma_{1}$ \\
icsd\_187195 & GeMn & 198 & 146.10 & 0.00 & $\Gamma_{4}$ \\
icsd\_038843 & NiSSb & 198 & 198.9 & 0.00 & $\Gamma_{1}$ \\
icsd\_041209 & F$_{2}$Pd & 205 & 205.33 & 1.54 & $\Gamma_{1}^{+}$ \\
icsd\_633869 & FeTe$_{2}$ & 205 & 61.433 & 0.00 & $\Gamma_{2}^+\Gamma_{3}^+$ \\
icsd\_024021 & MnTe$_{2}$ & 205 & 205.33 & 0.49 & $\Gamma_{1}^{+}$ \\
icsd\_040328 & NiS$_{2}$ & 205 & 205.33 & 0.54 & $\Gamma_{1}^{+}$ \\
icsd\_040330 & NiSe$_{2}$ & 205 & 61.436 & 0.19 & $\Gamma_{4}^{+}$ \\
icsd\_608469 & Al$_{0.6}$Mn$_{0.4}$ & 213 & 92.115 & 0.00 & $\Gamma_{5}$ \\
icsd\_044729 & CFe$_{4}$ & 215 & 111.255 & 0.00 & $\Gamma_{5}$ \\
icsd\_052642 & AlNTi$_{3}$ & 221 & 8.34 & 0.00 & $\Gamma_{4}^{+}$ \\
icsd\_053141 & Cr$_{3}$NPd & 221 & 166.97 & 0.00 & $\Gamma_{5}^{+}$ \\
icsd\_053142 & Cr$_{3}$NPt & 221 & 166.101 & 0.00 & $\Gamma_{4}^{+}$ \\
icsd\_168836 & H$_{2}$Mg$_{0.25}$Ti$_{0.75}$ & 221 & 166.97 & 0.00 & $\Gamma_{5}^{+}$ \\
icsd\_193569 & MgNi$_{3}$ & 221 & 5.13 & 0.00 & $\Gamma_{5}^{+}$ \\
icsd\_102767 & Cr$_{3}$Ga & 223 & 167.105 & 0.00 & $\Gamma_{4}^{-}$ \\
icsd\_053127 & Cr$_{3}$Ge & 223 & 167.106 & 0.00 & $\Gamma_{5}^{-}$ \\
icsd\_015904 & Cr$_{3}$O & 223 & 2.6 & 0.00 & $\Gamma_{5}^{-}$ \\
icsd\_016835 & Cr$_{3}$Si & 223 & 167.106 & 0.00 & $\Gamma_{5}^{-}$ \\
icsd\_104020 & GaV$_{3}$ & 223 & 167.106 & 0.00 & $\Gamma_{5}^{-}$ \\
icsd\_611953 & H$_{3}$AuTi$_{3}$ & 223 & 167.105 & 0.00 & $\Gamma_{4}^{-}$ \\
icsd\_052330 & SbV$_{3}$ & 223 & 223.106 & 0.00 & $\Gamma_{2}^{-}$ \\
icsd\_022412 & SiV$_{3}$ & 223 & 167.106 & 0.00 & $\Gamma_{5}^{-}$ \\
\hline
\end{tabular}
\label{NoCAFMfinal}
\end{table*}

\newpage
\subsection{Altermagnetic materials}
The relevant information for  altermagnetic materials is summarized in Table \ref{Alter}-\ref{Alterfinal}, including their chemical formula, space group, magnetic space group, band gap and corresponding irreducible representations of crystallographic space group.

\begin{table*}[!h]
\centering
\caption{Tabulated information on \textbf{altermagnetic} materials, including the chemical formula, 
space group, magnetic space group, band gap and corresponding irreducible representations of crystallographic space group.}
\renewcommand{\arraystretch}{0.8}
% [inline block 2: 8 envs, 30995 chars -> data_tex | \begin{tabular}{cccccc} \hline...]

% \end{table*}

\newpage

\section{Topological Magnetic Materials in our Magnetic Materials Database}
For decades, the topology of electronic band structures has been a central research focus \cite{RevModPhys.82.3045,Zhang2009,RevModPhys.90.015001,PhysRevB.83.205101,PhysRevB.85.195320,PhysRevX.5.011029,Huang2015}. Owing to the development of topological quantum chemistry and symmetry-indicator theory \cite{Bradlyn2017,Po2017,PhysRevX.7.041069,Tang2019,Song2018}, tens of thousands of nonmagnetic topological materials have been identified \cite{natureTang2019,natureZhang2019,natureVergniory2019}.
However, due to the limited number of known magnetic structures, theoretical predictions of magnetic topological materials remain relatively scarce, with only a few hundred reported to date \cite{natureBernevig2022,xu2020high}. Based on our magnetic structure database, we employ magnetic topological quantum chemistry to identify 1,070 magnetic topological materials \cite{Elcoro2021,xu2020high}, substantially expanding the known database of magnetic topological materials.

Among the more than 2,900 magnetic materials contained in our constructed magnetic structure database, we successfully determined the topological classifications of 2,814 materials. Fig. \ref{fig:Topological} presents a statistical overview of the topological classifications of these magnetic materials. The data are divided into five distinct topological classifications, as defined by the accompanying abbreviations:

The magnetic topological insulating phases (TIs) comprise 125 materials, accounting for 4.4\% of the dataset. These include axion insulators (AXIs), three-dimensional quantum anomalous Hall insulators (3D QAHIs), magnetic topological crystalline insulators (TCIs), and higher-order topological insulators (HOTIs). The detailed information of these materials is fully listed in \autoref{TABLETI}.

Smith-index semimetals (SISMs) are defined as topological semimetals whose band crossings do not occur at high-symmetry points, lines, or planes, but are instead enforced at generic momenta in the Brillouin zone. We identify 57 SISMs, corresponding to 2.0\% of the dataset. Detailed information on these materials is provided in \autoref{TABLESISM}.

Enforced semimetals with Fermi degeneracy (ESFD) are topological semimetals characterized by degenerate points at high-symmetry points in the Brillouin zone. A total of 85 ESFD are found, accounting for 3.0\%. A complete list of detailed information for these materials is presented in \autoref{TABLEESFD}.

Enforced semimetals (ESs) are topological semimetals in which band crossings occur along high-symmetry lines or planes due to the violation of compatibility relations. We identify 803 ESs, representing 28.5\% of the dataset. The complete details of these materials are presented in \autoref{TABLEES}.

Linear combinations of elementary band representations (LCEBR) indicate the absence of symmetry-protected topological features and comprise 1744 entries, accounting for 61.9\% of the total dataset. Further details of these materials can be found in \autoref{TABLELCEBR}.

The magnetic structure, electronic band structures, and associated information of topological magnetic materials is available at \url{https://magdatabase.nju.edu.cn}, which is continuously updated.
\begin{figure}[h]
\centering
\includegraphics[width=0.9\textwidth]{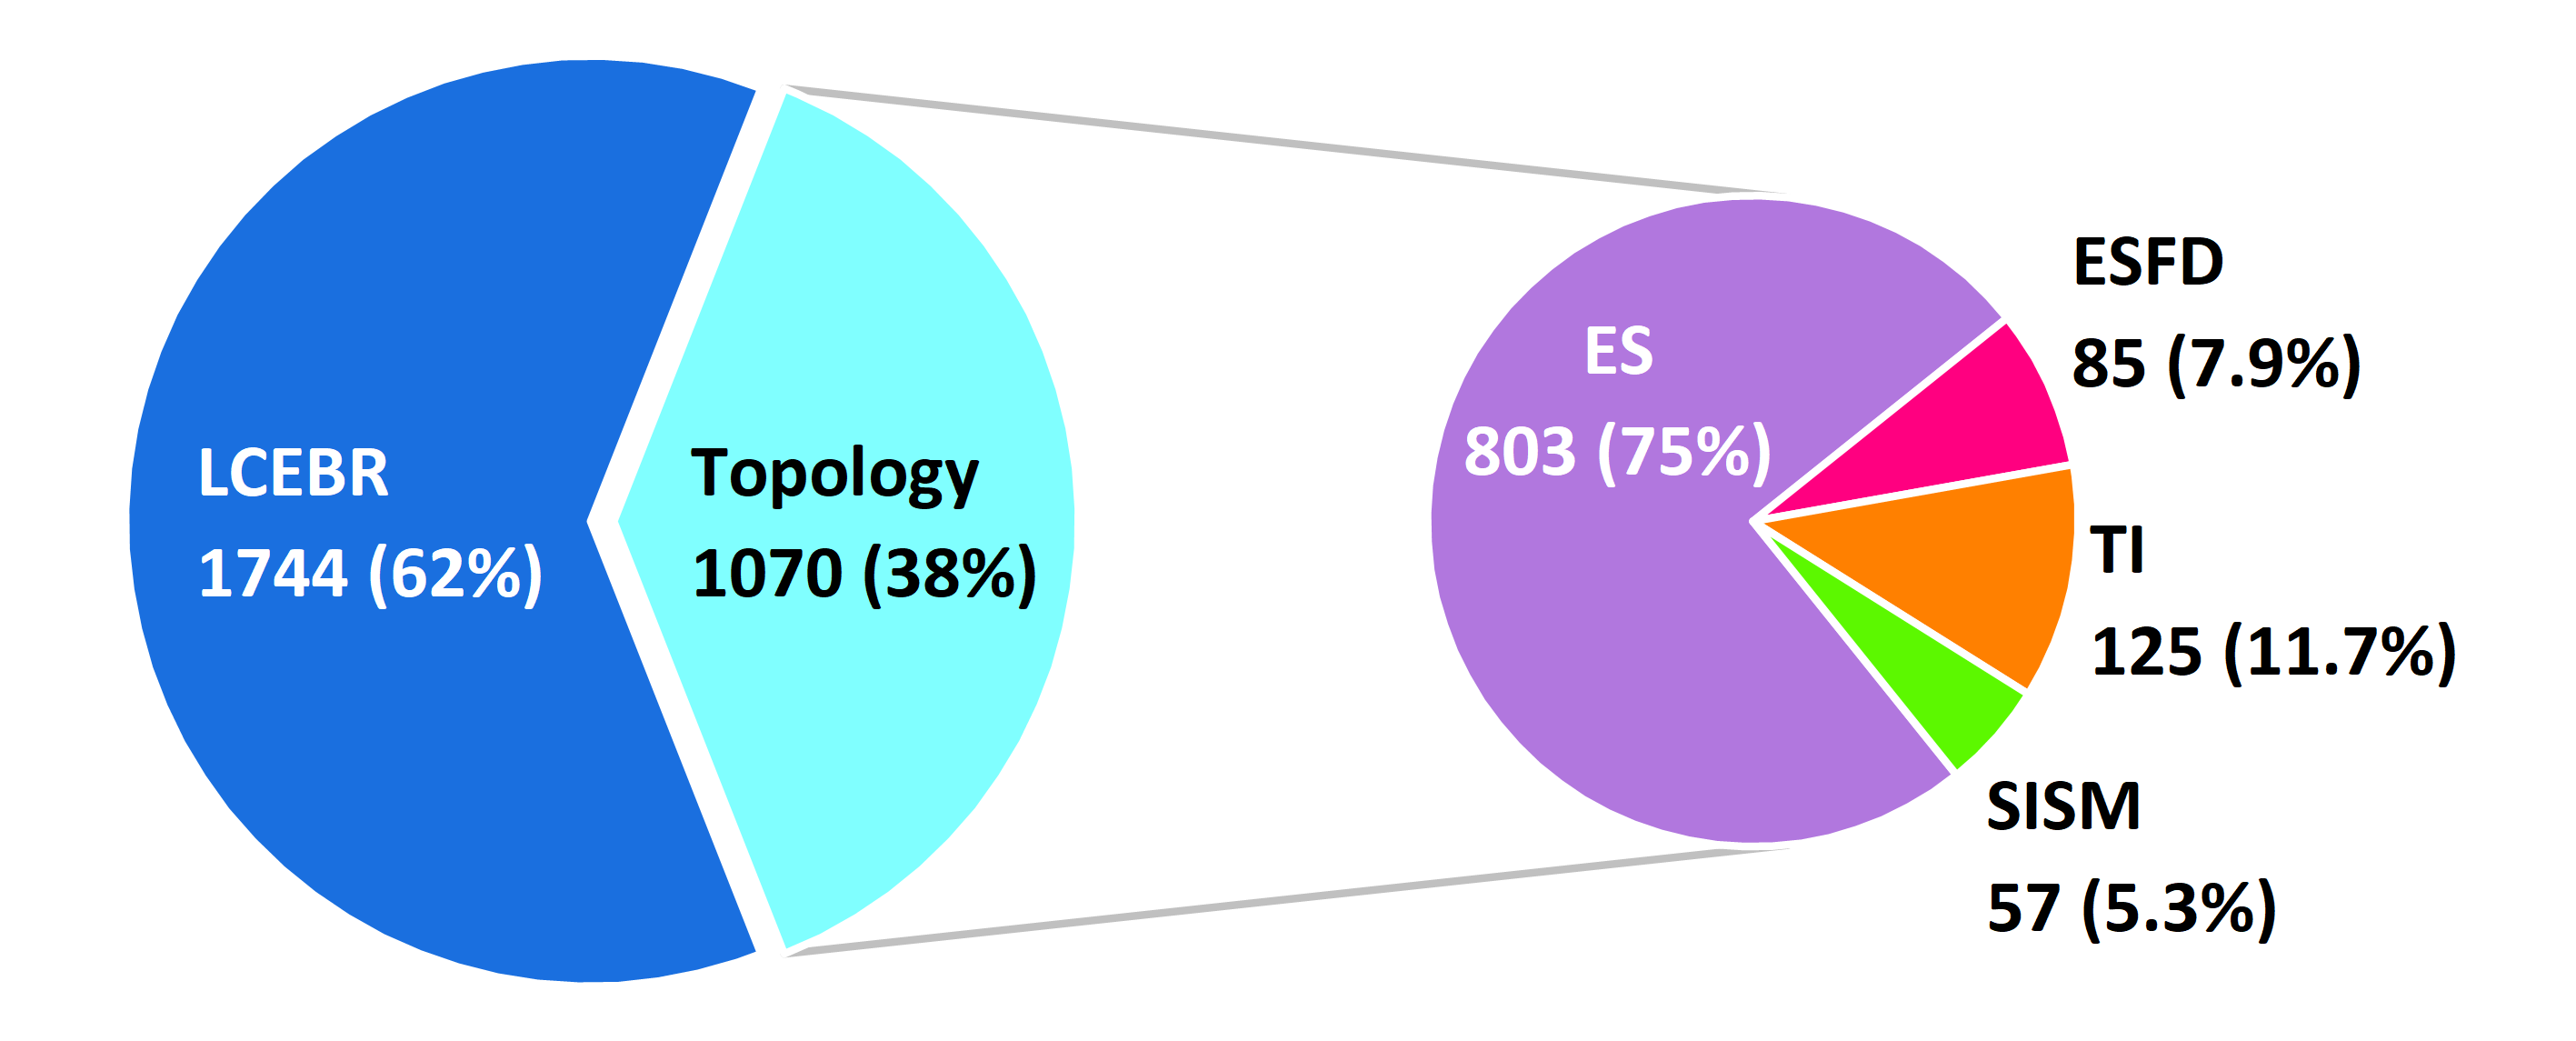}
\caption{Statistics of Topological Classification.}

\label{fig:Topological}
\end{figure}

\clearpage
\subsection{Table of Magnetic Topological Insulators}
\label{TABLETI}
In this subsection, we summarize all magnetic topological insulating phases (TIs) in a series of tables. These tables list the ICSD numbers, chemical formulas, MSGs, symmetry indicators, and topological subclassification. The symmetry indicators adopted here follow the conventions established in Refs. \cite{Elcoro2021, xu2020high}. The possible topological subclassifications include axion insulators (AXIs), three-dimensional quantum anomalous Hall insulators (3D QAHIs), magnetic topological crystalline insulators (TCIs), higher-order topological insulators (HOTIs). Notably, some symmetry indicators cannot uniquely determine the topological subclassifications. For example, $(\eta_{4I}, z_{2I,1}, z_{2I,2}, z_{2I,3})=(2,0,0,0)$ may correspond either to an AXI or to a high-Chern-number 3D QAHI. In such cases, further calculation of topological invariants is required to confirm the subclassification. We separate the possible topological subclassification with a slash (“/”).

\begin{table*}[htbp]
\centering
\caption{ICSD numbers, chemical formulas, magnetic space groups (MSGs), symmetry indicators, and topological subclassifications for magnetic topological insulating phases (TI).}
\begin{tabular}{c c c l c}
\hline
ICSD & Formula & MSG & Symmetry indicators & Topological subclassification \\
\hline
icsd\_015079 & B$_{4}$Mn & 12.62 & \makecell[l]{$\eta_{4I} = 0; z_{2I,1} = 1; z_{2I,2} = 1$ \\ $z_{2I,3} = 0$} & 3D QAHI \\ \hline
icsd\_066509 & Cu$_{2}$Li$_{3}$O$_{4}$ & 12.62 & \makecell[l]{$\eta_{4I} = 0; z_{2I,1} = 1; z_{2I,2} = 1$ \\ $z_{2I,3} = 1$} & 3D QAHI \\ \hline
icsd\_075420 & CrS$_{2}$ & 12.62 & \makecell[l]{$\eta_{4I} = 2; z_{2I,1} = 0; z_{2I,2} = 0$ \\ $z_{2I,3} = 1$} & 3D QAHI \\ \hline
icsd\_251718 & CrSe$_{2}$ & 12.62 & \makecell[l]{$\eta_{4I} = 2; z_{2I,1} = 0; z_{2I,2} = 0$ \\ $z_{2I,3} = 1$} & 3D QAHI \\ \hline
icsd\_646533 & NiSe$_{4}$Si$_{2}$ & 12.62 & \makecell[l]{$\eta_{4I} = 2; z_{2I,1} = 1; z_{2I,2} = 1$ \\ $z_{2I,3} = 0$} & 3D QAHI \\ \hline
icsd\_169074 & As$_{2}$BaOTi$_{2}$ & 65.486 & \makecell[l]{$\eta_{4I} = 2; z_{2I,1} = 0; z_{2I,2} = 0$ \\ $\delta_{2m} = 1; z^{-}_{2m,\pi} = 0; z^{+}_{2m,\pi} = 0$} & AXI/3D QAHI/TCI \\ \hline
icsd\_094745 & ClMnO$_{3}$Sr$_{2}$ & 129.417 & \makecell[l]{$\eta_{4I} = 0; z_{2I,3} = 0; z_{2R} = 0$ \\ $z_{4R} = 2; z_{2} = 0; z_{4S} = 2$} & 3D QAHI \\ \hline
icsd\_069044 & CaNNi & 66.496 & $\eta_{4I} = 2; z_{2I,1} = 1; z_{2I,2} = 1$ & 3D QAHI \\ \hline
icsd\_187709 & NTc & 66.496 & $\eta_{4I} = 2; z_{2I,1} = 1; z_{2I,2} = 1$ & 3D QAHI \\ \hline
icsd\_407550 & CoIn$_{3}$ & 136.499 & $\eta_{4I} = 2; \delta_{2m} = 1$ & AXI/TCI \\ \hline
icsd\_010462 & CaCo$_{2}$P$_{2}$ & 139.536 & $z_{2} = 1$ & AXI \\ \hline
icsd\_430064 & Bi$_{2}$F$_{2}$OSr$_{2}$Ti$_{2}$ & 139.534 & $\eta_{4I} = 0; \delta_{2m} = 0; z_{4} = 2$ & TCI/HOTI \\ \hline
icsd\_042531 & BCo$_{2}$ & 72.544 & \makecell[l]{$\eta_{4I} = 0; z_{2I,1} = 1; z_{2I,2} = 1$ \\ $z_{2I,3} = 1; \eta_{2I}^{'} = 0; z_{2R}^{'} = 1$} & 3D QAHI \\ \hline
icsd\_062157 & BaMo$_{6}$S$_{8}$ & 2.4 & \makecell[l]{$\eta_{4I} = 2; z_{2I,1} = 0; z_{2I,2} = 0$ \\ $z_{2I,3} = 0$} & AXI/3D QAHI \\ \hline
icsd\_639106 & HgMo$_{6}$S$_{8}$ & 2.4 & \makecell[l]{$\eta_{4I} = 2; z_{2I,1} = 0; z_{2I,2} = 0$ \\ $z_{2I,3} = 0$} & AXI/3D QAHI \\ \hline
icsd\_641241 & KMo$_{6}$S$_{8}$ & 148.17 & \makecell[l]{$\eta_{4I} = 0; z_{2I,1} = 1; z_{2I,2} = 1$ \\ $z_{2I,3} = 1$} & 3D QAHI \\ \hline
icsd\_671511 & AsInNi$_{3}$ & 2.4 & \makecell[l]{$\eta_{4I} = 2; z_{2I,1} = 0; z_{2I,2} = 0$ \\ $z_{2I,3} = 1$} & 3D QAHI \\ \hline
icsd\_169980 & HNiO$_{2}$ & 156.51 & $z_{3R} = 2$ & 3D QAHI \\ \hline
icsd\_044612 & Fe$_{2}$N & 162.77 & $\eta_{4I} = 0; z_{2I,3} = 1; z_{3R} = 0$ & 3D QAHI \\ \hline
icsd\_042559 & NiTe$_{2}$ & 164.89 & $\eta_{4I} = 2; z_{2I,3} = 0; z_{3R} = 0$ & AXI/3D QAHI \\ \hline
icsd\_603582 & Te$_{2}$V & 12.62 & \makecell[l]{$\eta_{4I} = 0; z_{2I,1} = 0; z_{2I,2} = 0$ \\ $z_{2I,3} = 1$} & 3D QAHI \\ \hline
icsd\_001004 & ClSc & 166.101 & \makecell[l]{$\eta_{4I} = 0; z_{2I,1} = 1; z_{2I,2} = 1$ \\ $z_{2I,3} = 1$} & 3D QAHI \\ \hline
icsd\_005435 & Co$_{3}$S$_{2}$Sn$_{2}$ & 12.62 & \makecell[l]{$\eta_{4I} = 2; z_{2I,1} = 0; z_{2I,2} = 0$ \\ $z_{2I,3} = 1$} & 3D QAHI \\ \hline
icsd\_108894 & In$_{2}$Ni$_{3}$S$_{2}$ & 12.58 & \makecell[l]{$\eta_{4I} = 2; z_{2I,1} = 0; z_{2I,2} = 0$ \\ $\delta_{2m} = 1; z^{-}_{2m,\pi} = 0; z^{+}_{2m,\pi} = 0$} & AXI/3D QAHI/TCI \\ \hline
icsd\_168949 & CoY & 12.62 & \makecell[l]{$\eta_{4I} = 2; z_{2I,1} = 0; z_{2I,2} = 0$ \\ $z_{2I,3} = 1$} & 3D QAHI \\ \hline
icsd\_425966 & Bi$_{2}$MnTe$_{4}$ & 166.101 & \makecell[l]{$\eta_{4I} = 2; z_{2I,1} = 0; z_{2I,2} = 0$ \\ $z_{2I,3} = 0$} & AXI/3D QAHI \\ \hline
icsd\_670141 & CrGa$_{4}$ & 12.62 & \makecell[l]{$\eta_{4I} = 2; z_{2I,1} = 0; z_{2I,2} = 0$ \\ $z_{2I,3} = 0$} & AXI/3D QAHI \\ \hline
icsd\_670405 & Fe$_{6}$Ge$_{4}$Mg & 166.101 & \makecell[l]{$\eta_{4I} = 3; z_{2I,1} = 1; z_{2I,2} = 1$ \\ $z_{2I,3} = 1$} & 3D QAHI \\ \hline
icsd\_182148 & Sn$_{6}$V$_{6}$Y & 65.486 & \makecell[l]{$\eta_{4I} = 2; z_{2I,1} = 0; z_{2I,2} = 0$ \\ $\delta_{2m} = 1; z^{-}_{2m,\pi} = 0; z^{+}_{2m,\pi} = 0$} & AXI/3D QAHI/TCI \\ \hline
icsd\_023910 & SbV & 63.462 & $\eta_{4I} = 2$ & AXI/3D QAHI \\ \hline
icsd\_042557 & NiTe & 63.462 & $\eta_{4I} = 2$ & AXI/3D QAHI \\ \hline
icsd\_044074 & AsTi & 63.457 & $\eta_{4I} = 2; \delta_{2m} = 1$ & AXI/TCI \\ \hline
icsd\_056142 & FeTe & 63.462 & $\eta_{4I} = 2$ & AXI/3D QAHI \\ \hline
icsd\_057506 & AlAuTi & 63.457 & $\eta_{4I} = 2; \delta_{2m} = 1$ & AXI/TCI \\ \hline
\end{tabular}
\label{tableSI}
\end{table*}

\clearpage

\begin{table*}[htbp]
\centering
\caption{ICSD numbers, chemical formulas, magnetic space groups (MSGs), symmetry indicators, and topological subclassifications for magnetic topological insulating phases (TI).}
\begin{tabular}{c c c l c}
\hline
ICSD & Formula & MSG & Symmetry indicators & Topological subclassification \\
\hline
icsd\_076118 & CoSb & 63.463 & \makecell[l]{$\eta_{4I} = 2; z_{2I,1} = 0; z_{2I,2} = 0$ \\ $\delta_{2m} = 1; z^{-}_{2m,\pi} = 0; z^{+}_{2m,\pi} = 0$} & AXI/3D QAHI/TCI \\ \hline
icsd\_076406 & SbTi & 63.462 & $\eta_{4I} = 2$ & AXI/3D QAHI \\ \hline
icsd\_169821 & NV & 63.464 & \makecell[l]{$\eta_{4I} = 2; z_{2I,1} = 0; z_{2I,2} = 0$ \\ $\eta_{2I}^{'} = 1; z_{2R}^{'} = 0$} & AXI/3D QAHI \\ \hline
icsd\_603343 & GeMn$_{3}$ & 63.464 & \makecell[l]{$\eta_{4I} = 2; z_{2I,1} = 0; z_{2I,2} = 0$ \\ $\eta_{2I}^{'} = 1; z_{2R}^{'} = 0$} & AXI/3D QAHI \\ \hline
icsd\_616410 & Be$_{2}$Ru & 63.462 & $\eta_{4I} = 2$ & AXI/3D QAHI \\ \hline
icsd\_077829 & LaSe & 2.4 & \makecell[l]{$\eta_{4I} = 0; z_{2I,1} = 0; z_{2I,2} = 0$ \\ $z_{2I,3} = 1$} & 3D QAHI \\ \hline
icsd\_633475 & FeSe$_{2}$ & 61.436 & $\eta_{4I} = 2$ & AXI/3D QAHI \\ \hline
icsd\_633869 & FeTe$_{2}$ & 61.433 & $\eta_{4I} = 2$ & AXI \\ \hline
icsd\_646897 & NiTe$_{2}$ & 61.436 & $\eta_{4I} = 2$ & AXI/3D QAHI \\ \hline
icsd\_044729 & CFe$_{4}$ & 111.255 & \makecell[l]{$z_{2R} = 0; \delta_{2S} = 0; z_{2} = 1$ \\ $z_{4S} = 0$} & AXI/3D QAHI \\ \hline
icsd\_023586 & CGaMn$_{3}$ & 166.101 & \makecell[l]{$\eta_{4I} = 0; z_{2I,1} = 1; z_{2I,2} = 1$ \\ $z_{2I,3} = 1$} & 3D QAHI \\ \hline
icsd\_052642 & AlNTi$_{3}$ & 65.486 & \makecell[l]{$\eta_{4I} = 2; z_{2I,1} = 1; z_{2I,2} = 1$ \\ $\delta_{2m} = 1; z^{-}_{2m,\pi} = 1; z^{+}_{2m,\pi} = 1$} & 3D QAHI/TCI \\ \hline
icsd\_057928 & AlIr & 123.345 & $\delta_{4m}=2; z_{4m,\pi}^{-}=2; z_{4m,\pi}^{+}=2$ & TCI \\ \hline
icsd\_058726 & BeNi & 65.486 & \makecell[l]{$\eta_{4I} = 2; z_{2I,1} = 0; z_{2I,2} = 0$ \\ $\delta_{2m} = 1; z^{-}_{2m,\pi} = 0; z^{+}_{2m,\pi} = 0$} & AXI/3D QAHI/TCI \\ \hline
icsd\_058728 & BePd & 65.486 & \makecell[l]{$\eta_{4I} = 2; z_{2I,1} = 0; z_{2I,2} = 0$ \\ $\delta_{2m} = 1; z^{-}_{2m,\pi} = 0; z^{+}_{2m,\pi} = 0$} & AXI/3D QAHI/TCI \\ \hline
icsd\_096119 & Mn$_{3}$Sb & 166.101 & \makecell[l]{$\eta_{4I} = 2; z_{2I,1} = 1; z_{2I,2} = 1$ \\ $z_{2I,3} = 1$} & 3D QAHI \\ \hline
icsd\_168838 & H$_{2}$Mg$_{0.75}$Ti$_{0.25}$ & 65.486 & \makecell[l]{$\eta_{4I} = 2; z_{2I,1} = 0; z_{2I,2} = 0$ \\ $\delta_{2m} = 1; z^{-}_{2m,\pi} = 0; z^{+}_{2m,\pi} = 0$} & AXI/3D QAHI/TCI \\ \hline
icsd\_187256 & MgNi & 166.101 & \makecell[l]{$\eta_{4I} = 2; z_{2I,1} = 0; z_{2I,2} = 0$ \\ $z_{2I,3} = 0$} & AXI/3D QAHI \\ \hline
icsd\_052330 & SbV$_{3}$ & 223.106 & $z_{2} = 1$ & AXI \\ \hline
icsd\_026630 & H$_{2}$Cr & 166.101 & \makecell[l]{$\eta_{4I} = 2; z_{2I,1} = 0; z_{2I,2} = 0$ \\ $z_{2I,3} = 0$} & AXI/3D QAHI \\ \hline
icsd\_057008 & CCr & 166.101 & \makecell[l]{$\eta_{4I} = 2; z_{2I,1} = 0; z_{2I,2} = 0$ \\ $z_{2I,3} = 0$} & AXI/3D QAHI \\ \hline
icsd\_180457 & CNi & 71.536 & \makecell[l]{$\eta_{4I} = 2; z_{2I,1} = 0; z_{2I,2} = 0$ \\ $z_{2I,3} = 0; \delta_{2m} = 1; z^{-}_{2m,\pi} = 0$ \\ $z^{+}_{2m,\pi} = 0$} & AXI/3D QAHI/TCI \\ \hline
icsd\_086427 & CuO$_{5}$Sr$_{2}$Tl & 47.252 & $\delta_{2m}=0; z_{2m,\pi}^{-}=1; z_{2m,\pi}^{+}=1$ & TCI \\ \hline
icsd\_041726 & CrSb$_{2}$ & 58.398 & $\eta_{4I} = 2$ & AXI/3D QAHI \\ \hline
icsd\_169570 & NiS$_{2}$ & 58.398 & $\eta_{4I} = 2$ & AXI/3D QAHI \\ \hline
icsd\_196424 & B$_{4}$Fe & 58.398 & $\eta_{4I} = 2$ & AXI/3D QAHI \\ \hline
icsd\_166445 & FeSe & 62.441 & $\eta_{4I} = 2$ & AXI \\ \hline
icsd\_168323 & H$_{0.5}$Ti & 13.69 & $\eta_{4I} = 0; z_{2I,1} = 1; z_{2I,2} = 1$ & 3D QAHI \\ \hline
icsd\_084827 & CoHf$_{2}$P & 11.54 & $\eta_{4I} = 2; z_{2I,1} = 0; z_{2I,3} = 0$ & AXI/3D QAHI \\ \hline
icsd\_172559 & Ag$_{2}$NiO$_{2}$ & 12.58 & \makecell[l]{$\eta_{4I} = 2; z_{2I,1} = 0; z_{2I,2} = 0$ \\ $\delta_{2m} = 1; z^{-}_{2m,\pi} = 0; z^{+}_{2m,\pi} = 0$} & AXI/3D QAHI/TCI \\ \hline
icsd\_617514 & C$_{3}$Cr$_{2}$Lu$_{2}$ & 12.62 & \makecell[l]{$\eta_{4I} = 0; z_{2I,1} = 0; z_{2I,2} = 0$ \\ $z_{2I,3} = 1$} & 3D QAHI \\ \hline
icsd\_617562 & C$_{3}$Cr$_{2}$Y$_{2}$ & 12.62 & \makecell[l]{$\eta_{4I} = 0; z_{2I,1} = 0; z_{2I,2} = 0$ \\ $z_{2I,3} = 1$} & 3D QAHI \\ \hline
icsd\_670103 & AuCuO$_{2}$ & 12.62 & \makecell[l]{$\eta_{4I} = 2; z_{2I,1} = 1; z_{2I,2} = 1$ \\ $z_{2I,3} = 0$} & 3D QAHI \\ \hline
icsd\_049726 & CoPZr & 62.446 & $\eta_{4I} = 2$ & AXI/3D QAHI \\ \hline
icsd\_068280 & MnNbP & 62.446 & $\eta_{4I} = 2$ & AXI/3D QAHI \\ \hline
icsd\_076095 & MnPZr & 62.447 & $\eta_{4I} = 2$ & AXI/3D QAHI \\ \hline
icsd\_085947 & MnPTa & 62.446 & $\eta_{4I} = 2$ & AXI/3D QAHI \\ \hline
icsd\_165245 & CoScSi & 62.447 & $\eta_{4I} = 2$ & AXI/3D QAHI \\ \hline
icsd\_614256 & BFeW & 62.446 & $\eta_{4I} = 2$ & AXI/3D QAHI \\ \hline
icsd\_632129 & FeGeTa & 62.446 & $\eta_{4I} = 2$ & AXI/3D QAHI \\ \hline
icsd\_416513 & CoPd$_{2}$Se$_{2}$ & 72.544 & \makecell[l]{$\eta_{4I} = 0; z_{2I,1} = 1; z_{2I,2} = 1$ \\ $z_{2I,3} = 1; \eta_{2I}^{'} = 0; z_{2R}^{'} = 1$} & 3D QAHI \\ \hline
icsd\_600147 & FeGa$_{8}$Lu$_{2}$ & 47.252 & \makecell[l]{$\eta_{4I} = 0; z_{2I,3} = 0; z_{2R} = 0$ \\ $\delta_{2m} = 0; z^{-}_{2m,\pi} = 1; z^{+}_{2m,\pi} = 1$} & TCI \\ \hline
icsd\_044449 & B$_{2}$MnW$_{2}$ & 55.358 & $\eta_{4I} = 2$ & AXI/3D QAHI \\ \hline
\end{tabular}
\end{table*}

\clearpage

\begin{table*}[htbp]
\centering
\caption{ICSD numbers, chemical formulas, magnetic space groups (MSGs), symmetry indicators, and topological subclassifications for magnetic topological insulating phases (TI).}
\begin{tabular}{c c c l c}
\hline
ICSD & Formula & MSG & Symmetry indicators & Topological subclassification \\
\hline
icsd\_107331 & Co$_{2}$InZr$_{2}$ & 127.391 & \makecell[l]{$\eta_{4I} = 0; \delta_{2m} = 0; z^{-}_{2m,\pi} = 0$ \\ $z^{+}_{2m,\pi} = 0; z_{2w,3} = 0; z_{4} = 2$} & TCI \\ \hline
icsd\_614047 & B$_{2}$FeNb$_{2}$ & 55.358 & $\eta_{4I} = 2$ & AXI/3D QAHI \\ \hline
icsd\_614207 & B$_{2}$FeTa$_{2}$ & 55.358 & $\eta_{4I} = 2$ & AXI/3D QAHI \\ \hline
icsd\_062598 & C$_{2}$CoSc & 129.417 & \makecell[l]{$\eta_{4I} = 2; z_{2I,3} = 0; z_{2R} = 0$ \\ $z_{4R} = 0; z_{2} = 1; z_{4S} = 0$} & AXI \\ \hline
icsd\_085283 & CBNiY & 59.41 & $\eta_{4I} = 2$ & AXI/3D QAHI \\ \hline
icsd\_191258 & CrN$_{3}$Nb & 129.417 & \makecell[l]{$\eta_{4I} = 2; z_{2I,3} = 1; z_{2R} = 1$ \\ $z_{4R} = 3; z_{2} = 1; z_{4S} = 3$} & 3D QAHI \\ \hline
icsd\_031916 & CoO$_{2}$Pt & 12.58 & \makecell[l]{$\eta_{4I} = 2; z_{2I,1} = 0; z_{2I,2} = 0$ \\ $\delta_{2m} = 1; z^{-}_{2m,\pi} = 0; z^{+}_{2m,\pi} = 0$} & AXI/3D QAHI/TCI \\ \hline
icsd\_031917 & CoO$_{2}$Pd & 12.62 & \makecell[l]{$\eta_{4I} = 2; z_{2I,1} = 0; z_{2I,2} = 0$ \\ $z_{2I,3} = 0$} & AXI/3D QAHI \\ \hline
icsd\_160574 & Ag$_{2}$NiO$_{2}$ & 12.58 & \makecell[l]{$\eta_{4I} = 2; z_{2I,1} = 0; z_{2I,2} = 0$ \\ $\delta_{2m} = 1; z^{-}_{2m,\pi} = 0; z^{+}_{2m,\pi} = 0$} & AXI/3D QAHI/TCI \\ \hline
icsd\_173362 & Bi$_{5}$La$_{3}$Mn & 63.464 & \makecell[l]{$\eta_{4I} = 0; z_{2I,1} = 1; z_{2I,2} = 1$ \\ $\eta_{2I}^{'} = 0; z_{2R}^{'} = 1$} & 3D QAHI \\ \hline
icsd\_053018 & Co$_{3}$Nb$_{2}$Si & 63.464 & \makecell[l]{$\eta_{4I} = 2; z_{2I,1} = 0; z_{2I,2} = 0$ \\ $\eta_{2I}^{'} = 1; z_{2R}^{'} = 0$} & AXI/3D QAHI \\ \hline
icsd\_010509 & Al$_{11}$Mn$_{4}$ & 2.4 & \makecell[l]{$\eta_{4I} = 2; z_{2I,1} = 0; z_{2I,2} = 1$ \\ $z_{2I,3} = 0$} & AXI/3D QAHI \\ \hline
icsd\_015214 & NiRh$_{2}$Se$_{4}$ & 12.62 & \makecell[l]{$\eta_{4I} = 2; z_{2I,1} = 1; z_{2I,2} = 1$ \\ $z_{2I,3} = 1$} & 3D QAHI \\ \hline
icsd\_023970 & NiSe$_{4}$V$_{2}$ & 12.62 & \makecell[l]{$\eta_{4I} = 2; z_{2I,1} = 1; z_{2I,2} = 1$ \\ $z_{2I,3} = 1$} & 3D QAHI \\ \hline
icsd\_035140 & NiS$_{4}$V$_{2}$ & 12.62 & \makecell[l]{$\eta_{4I} = 2; z_{2I,1} = 1; z_{2I,2} = 1$ \\ $z_{2I,3} = 1$} & 3D QAHI \\ \hline
icsd\_038369 & Te$_{2}$V$_{1.04}$ & 12.58 & \makecell[l]{$\eta_{4I} = 2; z_{2I,1} = 1; z_{2I,2} = 1$ \\ $\delta_{2m} = 1; z^{-}_{2m,\pi} = 1; z^{+}_{2m,\pi} = 1$} & 3D QAHI/TCI \\ \hline
icsd\_042558 & Ni$_{3}$Se$_{4}$ & 12.62 & \makecell[l]{$\eta_{4I} = 2; z_{2I,1} = 1; z_{2I,2} = 1$ \\ $z_{2I,3} = 0$} & 3D QAHI \\ \hline
icsd\_042563 & FeS$_{4}$Ti$_{2}$ & 12.62 & \makecell[l]{$\eta_{4I} = 2; z_{2I,1} = 1; z_{2I,2} = 1$ \\ $z_{2I,3} = 0$} & 3D QAHI \\ \hline
icsd\_603354 & FeRh$_{2}$Se$_{4}$ & 12.58 & \makecell[l]{$\eta_{4I} = 0; z_{2I,1} = 1; z_{2I,2} = 1$ \\ $\delta_{2m} = 0; z^{-}_{2m,\pi} = 1; z^{+}_{2m,\pi} = 1$} & 3D QAHI/TCI \\ \hline
icsd\_622979 & CoFe$_{2}$Se$_{4}$ & 12.62 & \makecell[l]{$\eta_{4I} = 0; z_{2I,1} = 0; z_{2I,2} = 0$ \\ $z_{2I,3} = 1$} & 3D QAHI \\ \hline
icsd\_624485 & Co$_{2}$NiSe$_{4}$ & 12.62 & \makecell[l]{$\eta_{4I} = 2; z_{2I,1} = 1; z_{2I,2} = 1$ \\ $z_{2I,3} = 0$} & 3D QAHI \\ \hline
icsd\_624874 & CoS$_{4}$Ti$_{2}$ & 12.62 & \makecell[l]{$\eta_{4I} = 2; z_{2I,1} = 1; z_{2I,2} = 1$ \\ $z_{2I,3} = 1$} & 3D QAHI \\ \hline
icsd\_625002 & CoSe$_{4}$Ti$_{2}$ & 12.62 & \makecell[l]{$\eta_{4I} = 2; z_{2I,1} = 1; z_{2I,2} = 1$ \\ $z_{2I,3} = 1$} & 3D QAHI \\ \hline
icsd\_626577 & CrRh$_{2}$Se$_{4}$ & 12.62 & \makecell[l]{$\eta_{4I} = 2; z_{2I,1} = 0; z_{2I,2} = 0$ \\ $z_{2I,3} = 1$} & 3D QAHI \\ \hline
icsd\_633332 & Fe$_{0.5}$S$_{2}$Ti & 12.62 & \makecell[l]{$\eta_{4I} = 2; z_{2I,1} = 1; z_{2I,2} = 1$ \\ $z_{2I,3} = 0$} & 3D QAHI \\ \hline
icsd\_085291 & Ba$_{2}$Cu$_{3}$LaO$_{8}$ & 47.252 & \makecell[l]{$\eta_{4I} = 2; z_{2I,3} = 1; z_{2R} = 1$ \\ $\delta_{2m} = 1; z^{-}_{2m,\pi} = 1; z^{+}_{2m,\pi} = 0$} & 3D QAHI/TCI \\ \hline
icsd\_615019 & B$_{2}$Ni$_{2}$Sr & 58.398 & $\eta_{4I} = 2$ & AXI/3D QAHI \\ \hline
icsd\_044339 & BCo$_{3}$ & 62.446 & $\eta_{4I} = 2$ & AXI/3D QAHI \\ \hline
icsd\_167127 & CFe$_{2}$Ni & 62.446 & $\eta_{4I} = 2$ & AXI/3D QAHI \\ \hline
icsd\_251180 & CMn$_{3}$ & 62.446 & $\eta_{4I} = 2$ & AXI/3D QAHI \\ \hline
icsd\_636746 & GeIrTi & 62.446 & $\eta_{4I} = 2$ & AXI/3D QAHI \\ \hline
icsd\_641017 & IrSiTi & 62.447 & $\eta_{4I} = 2$ & AXI/3D QAHI \\ \hline
icsd\_670822 & CCo$_{2}$Fe & 62.446 & $\eta_{4I} = 2$ & AXI/3D QAHI \\ \hline
icsd\_670824 & CCr$_{2}$Fe & 62.446 & $\eta_{4I} = 2$ & AXI/3D QAHI \\ \hline
icsd\_670825 & CCrFe$_{2}$ & 62.441 & $\eta_{4I} = 2$ & AXI \\ \hline
icsd\_670827 & CCuFe$_{2}$ & 62.447 & $\eta_{4I} = 2$ & AXI/3D QAHI \\ \hline
icsd\_052332 & Sb$_{4}$V$_{5}$ & 12.62 & \makecell[l]{$\eta_{4I} = 2; z_{2I,1} = 0; z_{2I,2} = 0$ \\ $z_{2I,3} = 0$} & AXI/3D QAHI \\ \hline
icsd\_614755 & B$_{2}$MnMo$_{2}$ & 55.358 & $\eta_{4I} = 2$ & AXI/3D QAHI \\ \hline
icsd\_091199 & CuMnO$_{3}$SSr$_{2}$ & 129.417 & \makecell[l]{$\eta_{4I} = 2; z_{2I,3} = 1; z_{2R} = 1$ \\ $z_{4R} = 3; z_{2} = 1; z_{4S} = 3$} & 3D QAHI \\ \hline
\end{tabular}
\end{table*}

\clearpage

\begin{table*}[htbp]
\centering
\caption{ICSD numbers, chemical formulas, magnetic space groups (MSGs), symmetry indicators, and topological subclassifications for magnetic topological insulating phases (TI).}
\begin{tabular}{c c c l c}
\hline
ICSD & Formula & MSG & Symmetry indicators & Topological subclassification \\
\hline
icsd\_610777 & As$_{2}$LaRh$_{2}$ & 129.417 & \makecell[l]{$\eta_{4I} = 0; z_{2I,3} = 1; z_{2R} = 1$ \\ $z_{4R} = 3; z_{2} = 0; z_{4S} = 3$} & 3D QAHI \\ \hline
icsd\_163549 & C$_{3}$AlV$_{4}$ & 63.457 & $\eta_{4I} = 2; \delta_{2m} = 1$ & AXI/TCI \\ \hline
icsd\_671080 & NiSbV & 63.462 & $\eta_{4I} = 2$ & AXI/3D QAHI \\ \hline
icsd\_076056 & Mn$_{3}$NNi & 166.101 & \makecell[l]{$\eta_{4I} = 2; z_{2I,1} = 0; z_{2I,2} = 0$ \\ $z_{2I,3} = 0$} & AXI/3D QAHI \\ \hline
icsd\_076060 & Mn$_{3}$NRh & 166.101 & \makecell[l]{$\eta_{4I} = 2; z_{2I,1} = 0; z_{2I,2} = 0$ \\ $z_{2I,3} = 0$} & AXI/3D QAHI \\ \hline
icsd\_052989 & Co$_{2}$GeTi & 71.536 & \makecell[l]{$\eta_{4I} = 2; z_{2I,1} = 0; z_{2I,2} = 0$ \\ $z_{2I,3} = 0; \delta_{2m} = 1; z^{-}_{2m,\pi} = 0$ \\ $z^{+}_{2m,\pi} = 0$} & AXI/3D QAHI/TCI \\ \hline
icsd\_057643 & AlCo$_{2}$V & 166.101 & \makecell[l]{$\eta_{4I} = 2; z_{2I,1} = 0; z_{2I,2} = 0$ \\ $z_{2I,3} = 0$} & AXI/3D QAHI \\ \hline
icsd\_057994 & AlMn$_{2}$V & 166.101 & \makecell[l]{$\eta_{4I} = 2; z_{2I,1} = 0; z_{2I,2} = 0$ \\ $z_{2I,3} = 0$} & AXI/3D QAHI \\ \hline
icsd\_185936 & Co$_{2}$FeGe & 71.536 & \makecell[l]{$\eta_{4I} = 2; z_{2I,1} = 0; z_{2I,2} = 0$ \\ $z_{2I,3} = 0; \delta_{2m} = 1; z^{-}_{2m,\pi} = 0$ \\ $z^{+}_{2m,\pi} = 0$} & AXI/3D QAHI/TCI \\ \hline
\end{tabular}
\end{table*}

\clearpage

\clearpage

\subsection{Table of Magnetic Smith-index Semimetals}
\label{TABLESISM}
Smith-index semimetals (SISMs) are topological semimetals whose band representations satisfy the compatibility relations, while their symmetry indicators are incompatible with any insulating phase. Consequently, the electronic structure is gapped at all high-symmetry points, lines, and planes, and gapless band crossings are enforced at generic momenta.

In this subsection, we summarize all magnetic SISMs in a series of tables. These tables list the ICSD numbers, chemical formulas, MSGs, symmetry indicators. The symmetry indicators adopted here follow the conventions established in Refs. \cite{Elcoro2021, xu2020high}.

\begin{table*}[htbp]
\centering
\caption{ICSD numbers, chemical formulas, magnetic space groups (MSGs), and symmetry indicators for magnetic Smith-index semimetals (SISM).}
\begin{tabular}{c c c l}
\hline
ICSD & Formula & MSG & Symmetry indicators \\
\hline
icsd\_018176 & CoO$_{4}$S & 11.54 & $\eta_{4I} = 1; z_{2I,1} = 0; z_{2I,3} = 0$ \\ \hline
icsd\_099894 & CoO$_{3}$Sr$_{2}$ & 12.62 & $\eta_{4I} = 3; z_{2I,1} = 0; z_{2I,2} = 0; z_{2I,3} = 0$ \\ \hline
icsd\_624999 & CoSe$_{4}$Si$_{2}$ & 12.62 & $\eta_{4I} = 3; z_{2I,1} = 0; z_{2I,2} = 0; z_{2I,3} = 0$ \\ \hline
icsd\_246938 & BaCoS$_{2}$ & 13.69 & $\eta_{4I} = 1; z_{2I,1} = 1; z_{2I,2} = 0$ \\ \hline
icsd\_062156 & Mo$_{6}$S$_{8}$Sr & 148.17 & $\eta_{4I} = 1; z_{2I,1} = 1; z_{2I,2} = 1; z_{2I,3} = 1$ \\ \hline
icsd\_237739 & Au$_{5}$MnY$_{3}$ & 148.17 & $\eta_{4I} = 1; z_{2I,1} = 1; z_{2I,2} = 1; z_{2I,3} = 1$ \\ \hline
icsd\_075962 & D$_{12}$Ba$_{3}$Ir$_{2}$ & 12.62 & $\eta_{4I} = 1; z_{2I,1} = 0; z_{2I,2} = 0; z_{2I,3} = 0$ \\ \hline
icsd\_079991 & D$_{8}$BaFeMg$_{2}$ & 12.62 & $\eta_{4I} = 3; z_{2I,1} = 0; z_{2I,2} = 0; z_{2I,3} = 1$ \\ \hline
icsd\_086197 & D$_{2}$CoO$_{2}$ & 12.62 & $\eta_{4I} = 3; z_{2I,1} = 0; z_{2I,2} = 0; z_{2I,3} = 0$ \\ \hline
icsd\_626718 & CrSe$_{2}$ & 12.62 & $\eta_{4I} = 3; z_{2I,1} = 0; z_{2I,2} = 0; z_{2I,3} = 0$ \\ \hline
icsd\_420728 & Rh$_{3}$S$_{2}$Sn$_{2}$ & 166.101 & $\eta_{4I} = 3; z_{2I,1} = 0; z_{2I,2} = 0; z_{2I,3} = 0$ \\ \hline
icsd\_053564 & Fe$_{3}$Te$_{3}$Tl & 11.54 & $\eta_{4I} = 1; z_{2I,1} = 0; z_{2I,3} = 1$ \\ \hline
icsd\_080771 & Ba$_{3}$MnN$_{3}$ & 11.54 & $\eta_{4I} = 3; z_{2I,1} = 0; z_{2I,3} = 0$ \\ \hline
icsd\_000316 & FeS$_{2}$ & 148.17 & $\eta_{4I} = 1; z_{2I,1} = 0; z_{2I,2} = 0; z_{2I,3} = 0$ \\ \hline
icsd\_191175 & MnSb & 119.319 & $\delta_{2S} = 1; z_{2} = 0; z_{4S} = 2$ \\ \hline
icsd\_077036 & CInMn$_{3}$ & 166.101 & $\eta_{4I} = 3; z_{2I,1} = 0; z_{2I,2} = 0; z_{2I,3} = 0$ \\ \hline
icsd\_160196 & CrO$_{3}$Pb & 166.101 & $\eta_{4I} = 3; z_{2I,1} = 0; z_{2I,2} = 0; z_{2I,3} = 0$ \\ \hline
icsd\_181144 & NZr & 166.101 & $\eta_{4I} = 1; z_{2I,1} = 0; z_{2I,2} = 0; z_{2I,3} = 0$ \\ \hline
icsd\_236827 & MnN & 166.101 & $\eta_{4I} = 3; z_{2I,1} = 0; z_{2I,2} = 0; z_{2I,3} = 0$ \\ \hline
icsd\_236829 & FeN & 166.101 & $\eta_{4I} = 3; z_{2I,1} = 0; z_{2I,2} = 0; z_{2I,3} = 0$ \\ \hline
icsd\_043356 & SbTi$_{3}$ & 167.107 & $\eta_{4I} = 3$ \\ \hline
icsd\_611501 & AsTi$_{3}$ & 167.107 & $\eta_{4I} = 3$ \\ \hline
icsd\_056182 & H$_{2}$Ti & 166.101 & $\eta_{4I} = 3; z_{2I,1} = 0; z_{2I,2} = 0; z_{2I,3} = 0$ \\ \hline
icsd\_096297 & D$_{2}$Ti & 166.101 & $\eta_{4I} = 3; z_{2I,1} = 0; z_{2I,2} = 0; z_{2I,3} = 0$ \\ \hline
icsd\_424636 & Ga$_{4}$Mn & 166.101 & $\eta_{4I} = 3; z_{2I,1} = 0; z_{2I,2} = 0; z_{2I,3} = 0$ \\ \hline
icsd\_611737 & Au$_{4}$Cr & 12.62 & $\eta_{4I} = 3; z_{2I,1} = 1; z_{2I,2} = 1; z_{2I,3} = 0$ \\ \hline
icsd\_014026 & Cr$_{0.5}$NbSe$_{2}$ & 12.62 & $\eta_{4I} = 1; z_{2I,1} = 1; z_{2I,2} = 1; z_{2I,3} = 0$ \\ \hline
icsd\_645395 & Nb$_{2}$Se$_{4}$Ti & 12.62 & $\eta_{4I} = 1; z_{2I,1} = 1; z_{2I,2} = 1; z_{2I,3} = 0$ \\ \hline
icsd\_100785 & LaRu$_{3}$Si$_{2}$ & 11.54 & $\eta_{4I} = 1; z_{2I,1} = 0; z_{2I,3} = 0$ \\ \hline
icsd\_040908 & MnPdTe & 119.319 & $\delta_{2S} = 1; z_{2} = 0; z_{4S} = 0$ \\ \hline
icsd\_052673 & AuMnSb & 119.319 & $\delta_{2S} = 1; z_{2} = 0; z_{4S} = 0$ \\ \hline
icsd\_057504 & AlAu$_{2}$Mn & 166.101 & $\eta_{4I} = 3; z_{2I,1} = 0; z_{2I,2} = 0; z_{2I,3} = 0$ \\ \hline
icsd\_057981 & AlMnPd$_{2}$ & 166.101 & $\eta_{4I} = 1; z_{2I,1} = 0; z_{2I,2} = 0; z_{2I,3} = 0$ \\ \hline
icsd\_001501 & O$_{2}$V & 2.4 & $\eta_{4I} = 3; z_{2I,1} = 0; z_{2I,2} = 0; z_{2I,3} = 1$ \\ \hline
icsd\_159792 & CoLi$_{0.5}$O$_{2}$ & 10.46 & $\eta_{4I} = 1; z_{2I,1} = 1; z_{2I,2} = 0; z_{2I,3} = 1$ \\ \hline
icsd\_020953 & Co$_{4}$GaY$_{4}$ & 12.62 & $\eta_{4I} = 1; z_{2I,1} = 0; z_{2I,2} = 0; z_{2I,3} = 1$ \\ \hline
icsd\_084195 & Se$_{4}$V$_{3}$ & 12.62 & $\eta_{4I} = 1; z_{2I,1} = 0; z_{2I,2} = 0; z_{2I,3} = 1$ \\ \hline
icsd\_201787 & Mo$_{2}$S$_{4}$V & 12.62 & $\eta_{4I} = 1; z_{2I,1} = 0; z_{2I,2} = 0; z_{2I,3} = 1$ \\ \hline
icsd\_624816 & CoRh$_{2}$Se$_{4}$ & 12.62 & $\eta_{4I} = 3; z_{2I,1} = 1; z_{2I,2} = 1; z_{2I,3} = 1$ \\ \hline
icsd\_632972 & FeNi$_{2}$Se$_{4}$ & 12.62 & $\eta_{4I} = 1; z_{2I,1} = 0; z_{2I,2} = 0; z_{2I,3} = 1$ \\ \hline
\end{tabular}
\label{tableSISM}
\end{table*}

\clearpage

\begin{table*}[htbp]
\centering
\caption{ICSD numbers, chemical formulas, magnetic space groups (MSGs), and symmetry indicators for magnetic Smith-index semimetals (SISM).}
\begin{tabular}{c c c l}
\hline
ICSD & Formula & MSG & Symmetry indicators \\
\hline
icsd\_646388 & NiS$_{4}$Ti$_{2}$ & 12.62 & $\eta_{4I} = 1; z_{2I,1} = 1; z_{2I,2} = 1; z_{2I,3} = 0$ \\ \hline
icsd\_646544 & NiSe$_{4}$Ti$_{2}$ & 12.62 & $\eta_{4I} = 1; z_{2I,1} = 1; z_{2I,2} = 1; z_{2I,3} = 0$ \\ \hline
icsd\_095948 & NiO$_{3}$Tl & 14.79 & $\eta_{4I} = 3; z_{2I,1} = 1$ \\ \hline
icsd\_239671 & Ca$_{2}$CrO$_{6}$Os & 14.79 & $\eta_{4I} = 1; z_{2I,1} = 1$ \\ \hline
icsd\_031343 & Li$_{0.33}$Se$_{2}$Ti & 12.62 & $\eta_{4I} = 1; z_{2I,1} = 0; z_{2I,2} = 0; z_{2I,3} = 1$ \\ \hline
icsd\_076020 & O$_{2}$PTi$_{3}$ & 164.89 & $\eta_{4I} = 3; z_{2I,3} = 1; z_{3R} = 1$ \\ \hline
icsd\_025561 & STi & 12.62 & $\eta_{4I} = 1; z_{2I,1} = 0; z_{2I,2} = 0; z_{2I,3} = 0$ \\ \hline
icsd\_189226 & Co$_{3}$SiTi$_{2}$ & 11.54 & $\eta_{4I} = 1; z_{2I,1} = 0; z_{2I,3} = 0$ \\ \hline
icsd\_190988 & CoMnS & 119.319 & $\delta_{2S} = 1; z_{2} = 0; z_{4S} = 2$ \\ \hline
icsd\_190989 & CoMnSe & 119.319 & $\delta_{2S} = 1; z_{2} = 0; z_{4S} = 2$ \\ \hline
icsd\_052971 & Co$_{2}$GeMn & 166.101 & $\eta_{4I} = 3; z_{2I,1} = 0; z_{2I,2} = 0; z_{2I,3} = 0$ \\ \hline
icsd\_053312 & Cu$_{2}$MnSb & 166.101 & $\eta_{4I} = 1; z_{2I,1} = 0; z_{2I,2} = 0; z_{2I,3} = 0$ \\ \hline
icsd\_053687 & GeMnNi$_{2}$ & 166.101 & $\eta_{4I} = 3; z_{2I,1} = 0; z_{2I,2} = 0; z_{2I,3} = 0$ \\ \hline
icsd\_076080 & MnNi$_{2}$Sb & 166.101 & $\eta_{4I} = 3; z_{2I,1} = 0; z_{2I,2} = 0; z_{2I,3} = 0$ \\ \hline
icsd\_103813 & GaMn$_{2}$V & 166.101 & $\eta_{4I} = 1; z_{2I,1} = 0; z_{2I,2} = 0; z_{2I,3} = 0$ \\ \hline
icsd\_103892 & GaNi$_{2}$V & 166.101 & $\eta_{4I} = 3; z_{2I,1} = 0; z_{2I,2} = 0; z_{2I,3} = 0$ \\ \hline
icsd\_188333 & Mn$_{3}$Sn & 166.101 & $\eta_{4I} = 1; z_{2I,1} = 0; z_{2I,2} = 0; z_{2I,3} = 0$ \\ \hline
\end{tabular}
\end{table*}

\clearpage

\subsection{Table of Magnetic Enforced Semimetals with Fermi Degeneracy}
\label{TABLEESFD}
Enforced semimetals with Fermi degeneracy (ESFD) are topological semimetals whose band degeneracies are symmetry-enforced at high-symmetry points of the Brillouin zone.
In this subsection, we summarize all magnetic ESFD in a series of tables. These tables list the ICSD numbers, chemical formulas, and MSGs.

\begin{table*}[htbp]
\centering
\caption{ICSD numbers, chemical formulas, and magnetic space groups (MSGs) for magnetic enforced semimetals with Fermi degeneracy (ESFD).}
% [inline block 3: 7 envs, 37033 chars -> data_tex | \begin{tabular}{c c c | c c c} \hline...]

\end{table*}

\clearpage

\subsection{Table of Linear Combinations of Elementary Band Representation}
\label{TABLELCEBR}
Linear combinations of elementary band representations (LCEBR) indicate phases that do not exhibit symmetry-protected topological features. In this subsection, we summarize all magnetic LCEBR in a series of tables. These tables list the ICSD numbers, chemical formulas, and MSGs.

\begin{table*}[htbp]
\centering
\caption{ICSD numbers, chemical formulas, and magnetic space groups (MSGs) for magnetic linear combinations of elementary band representation (LCEBR).}
% [inline block 4: 13 envs, 74150 chars -> data_tex | \begin{tabular}{c c c | c c c} \hline...]

\end{table*}

\clearpage

\section{Altermagnetic Materials}

Altermagnets constitute a novel magnetic class distinct from conventional antiferromagnets, attracting considerable 
interest due to their unique band characteristics and transport properties 
\cite%
{PhysRevX.12.040501,PhysRevX.12.031042,PhysRevLett.132.056701,PhysRevLett.132.036702,gomonay2024structure,PhysRevLett.133.056701,bose2022tilted,zhu2024observation,krempasky2024altermagnetic,d41586-024-00190-w,PhysRevLett.134.106801,PhysRevLett.134.106802,zhou2025manipulation,PhysRevLett.126.127701,PhysRevLett.128.197202,PhysRevX.12.011028,PhysRevB.99.184432,PhysRevB.102.144441,PhysRevMaterials.5.014409,doi:10.1126/sciadv.aaz8809,PhysRevB.102.014422,Liu-nwaf528}.% 
 Altermagnets exhibit the collinear-compensated magnetic phase which are characterized by crystal-rotation
symmetries connecting opposite-spin sublattices separated in the real space, i.e. the symmetry $[C_2||A]$, where 
$C_2$ is the 180° rotation of
the spin space around an axis perpendicular to the spins, while transformations $A$ that can be only real-space proper or
improper rotations and cannot be real-space inversion. 
Based on this symmetry criterion, we identify 392 altermagnetic materials in our database, representing 13.5\% of all compounds.
A complete list of the candidate altermagnetic materials is provided in the Table \ref{Alter}. The magnetic structure, electronic band structures, and associated information of altermagnetic materials is available at \url{https://magdatabase.nju.edu.cn}, which is continuously updated.
Below we present representative material of Altermagnetism CsV$_2$S$_2$O in \autoref{CsV2S2O}.

\newpage
\subsection{Representative material of Altermagnetism CsV$_2$S$_2$O}
\label{CsV2S2O}
\begin{figure}[htbp]
    \centering
    \includegraphics[width=1\linewidth]{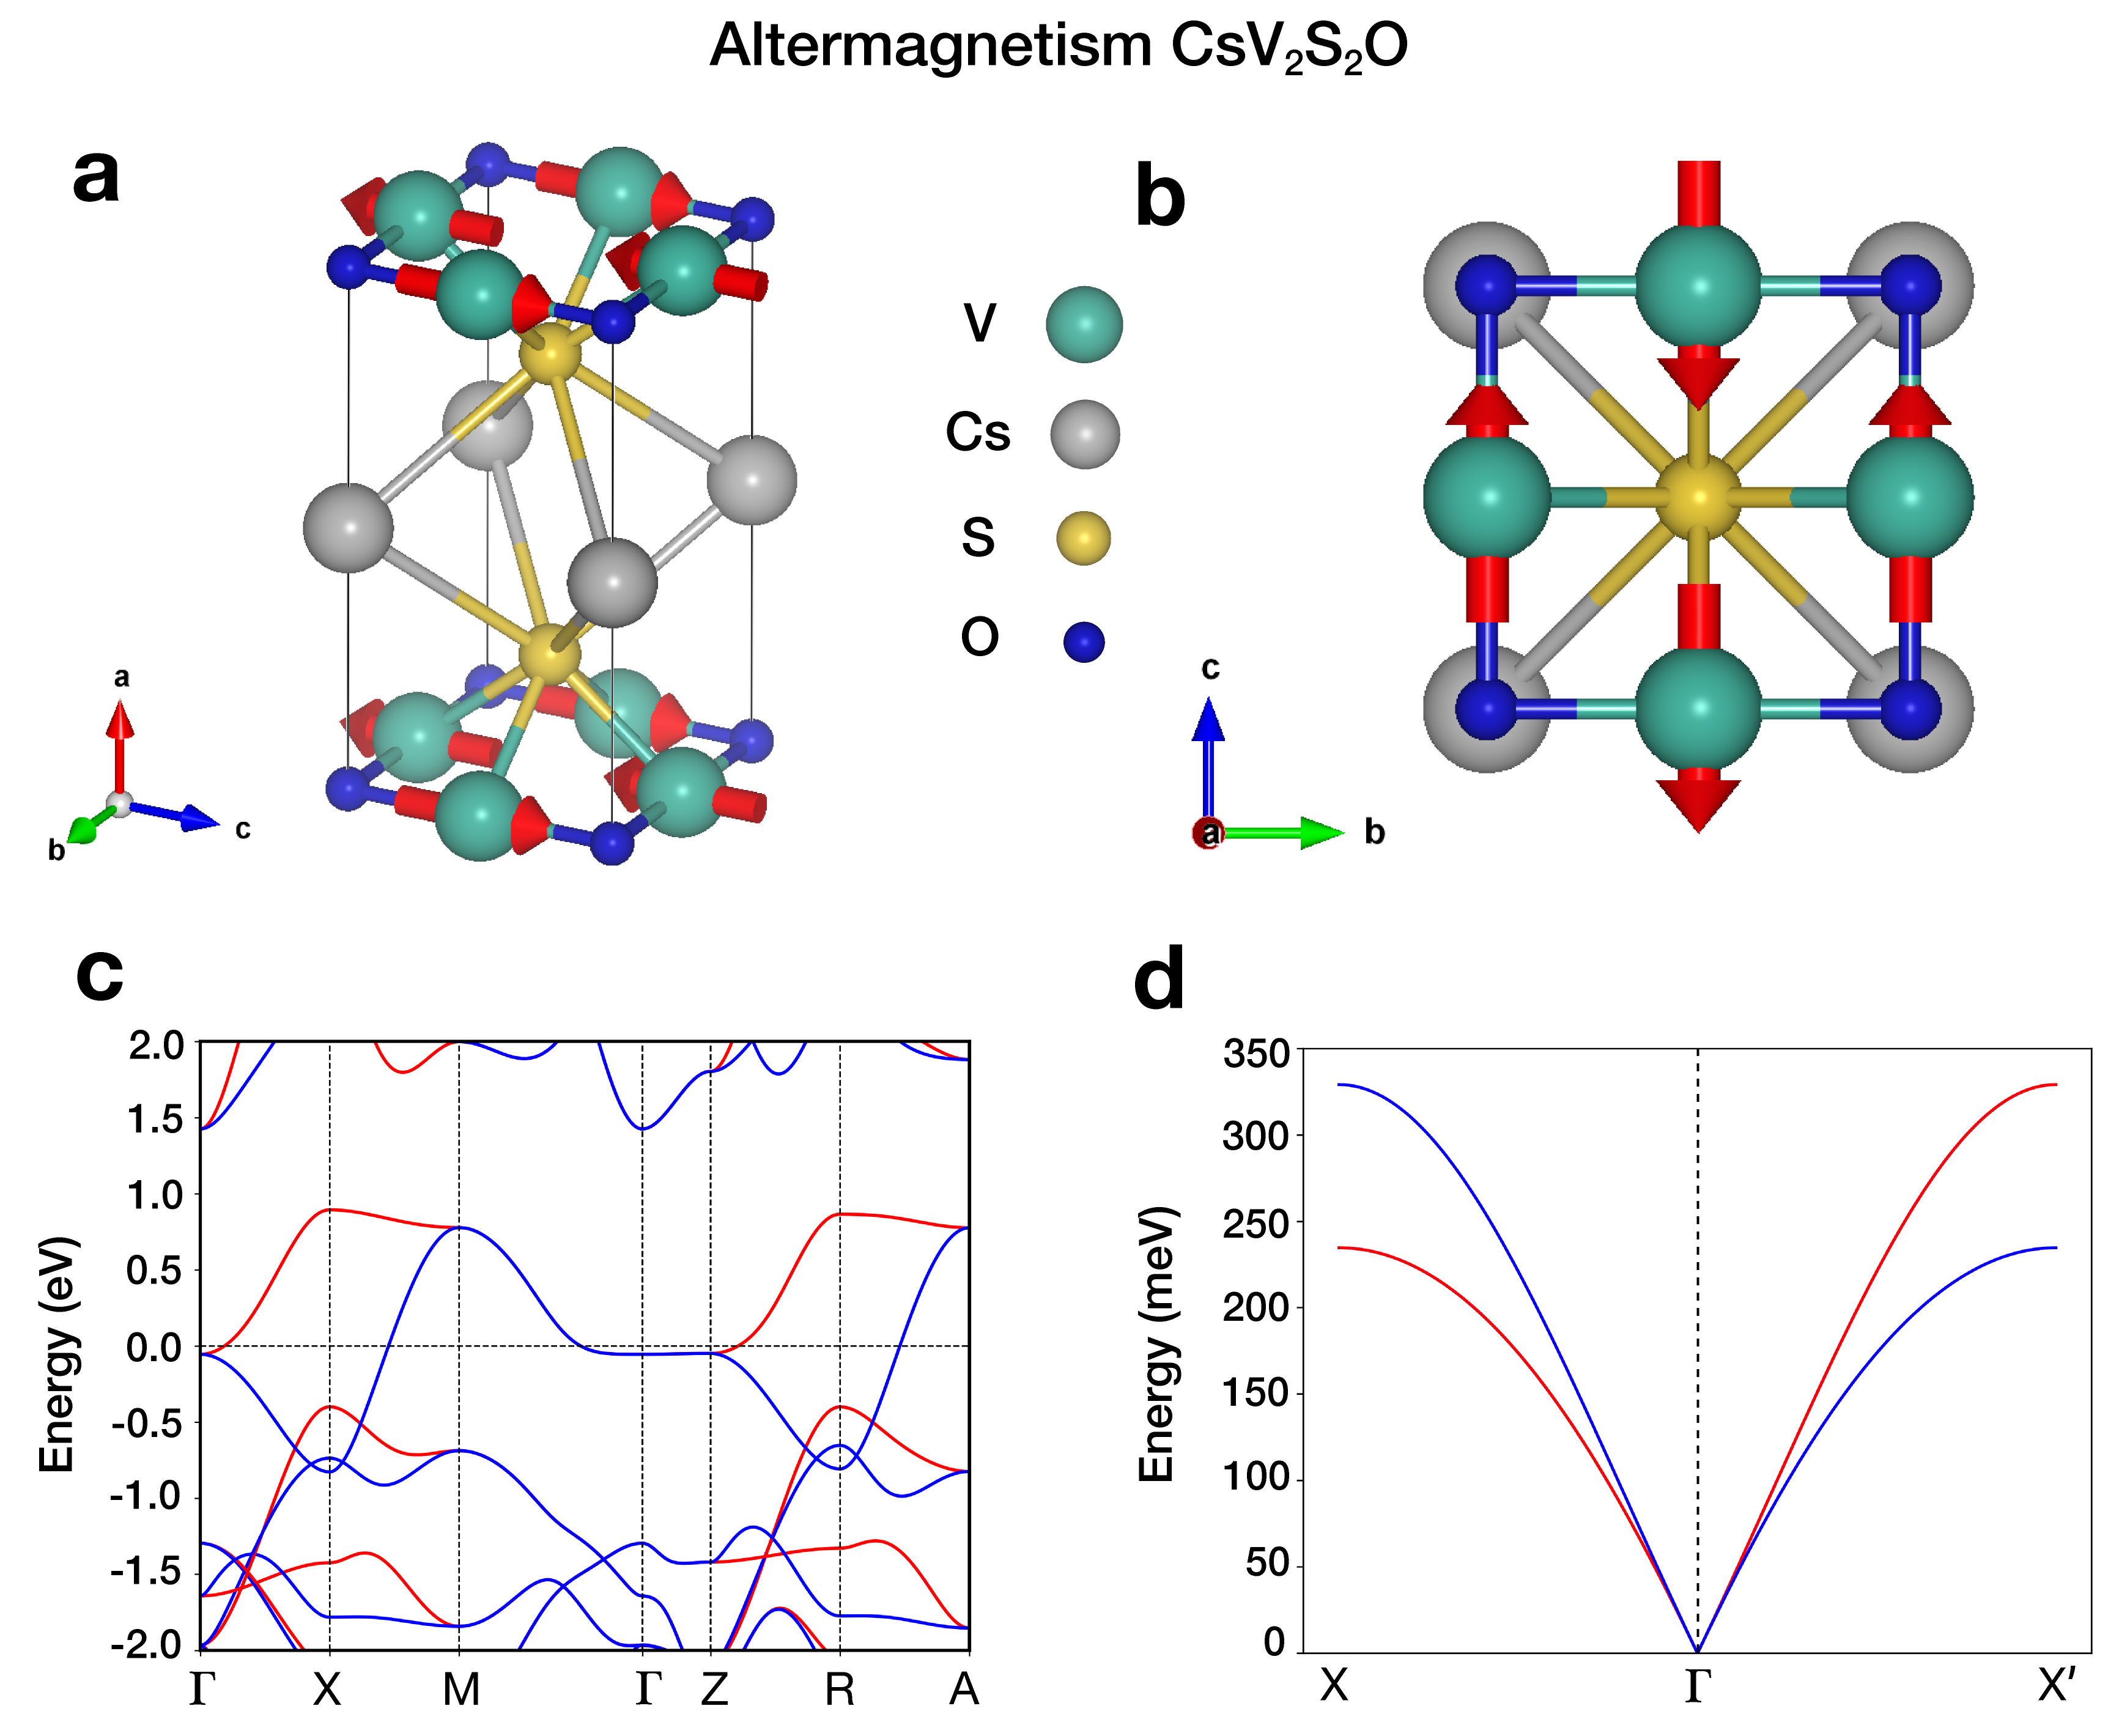}

    \caption{(a)(b) Crystal structure of CsV$_2$S$_2$O. 
        (c) Electron band splitting of CsV$_2$S$_2$O from first-principles calculations.
        (d) Chiral-magnon band splitting calculated based on the exchange interactions described in the main text, showing a maximum splitting of 94.4 meV at the X point. }
    \label{fig-altermagnetic}
\end{figure}

CsV$_2$S$_2$O crystallizes in space group $P4/mmm$ (No.~123) with magnetic ions occupying the $1b$ 
Wyckoff positions, 
as shown in Fig.~\ref{fig-altermagnetic}(a). It exhibits a pronounced altermagnetic spin splitting along high-symmetry paths [Fig.~\ref{fig-altermagnetic}(b)], with a momentum-dependent maximum of about 1.7~eV near the X point, 
indicating a very strong electronic altermagnetic effect. 

Typically, altermagnets exhibiting chiral splitting in magnon spectra originate from disparities 
in their exchange interactions with long-distance. 
In prototypical systems such as MnF$_2$ and MnTe, the exchange parameters (e.g., $J_{7a}$ versus $J_{7b}$ in MnF$_2$) 
produce minimal splitting amplitudes: experimental measurements show negligible chiral splitting in MnF$_2$ \cite{morano2025absence} and approximately 2~meV in MnTe \cite{liu2024chiral}. Based on the magnetic force theorem and linear-response calculations~\cite{CALJ-1,CALJ-2,CALJ-3}, 
the nearest-neighbor exchange interaction is $J_1 = 56.4$~meV, 
while two symmetry-inequivalent next-nearest-neighbor interactions take values $J_{2a} = -2.3$~meV and $J_{2b} = -25.8$~meV. 
This large disparity reflects the nonequivalent magnetic environments of the two sublattices and 
gives rise to a sizable chiral-magnon band splitting.
As shown in Fig.~\ref{fig-altermagnetic}(c), 
the splitting reaches up to 94.4~meV at the high-symmetry X point in the Brillouin zone, 
an exceptionally large value among known materials.

\bibliographystyle{aps}
\bibliography{MstrSM}

\end{document}
